# Supplementary material for: KIC 9406652: A laboratory of the tilted disk in cataclysmic variable stars
Source: arXiv:2008.11328 ancillary file (2020-08-27)
Supplement: Supplementary file 1 [file si-kic940-1.pdf]

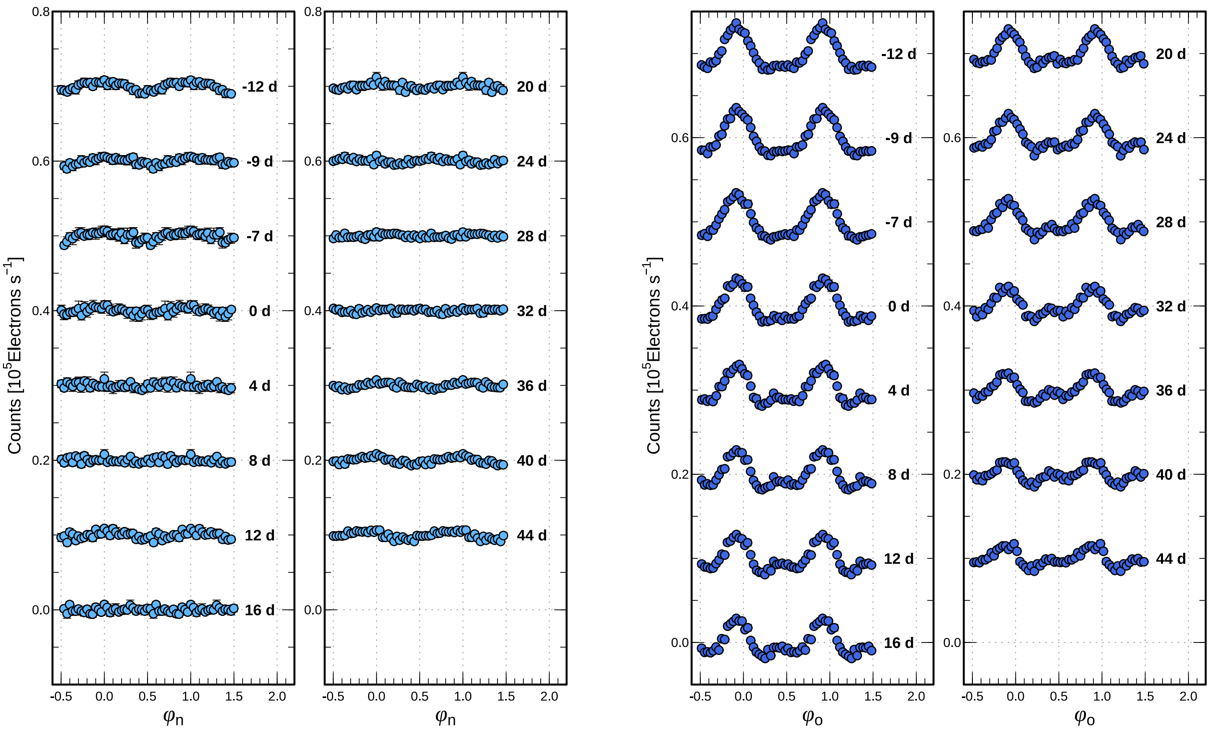


**Fig. E1.** Time evolution of phase-averaged profiles of negative superhumps (left) and orbital signals (right) during interval 1 in Fig. 1. We here fold light curves in a small window with the 12.7-d length by shifting the window with a certain time step. The number at the right side of each profile represents the date at the center of each window.

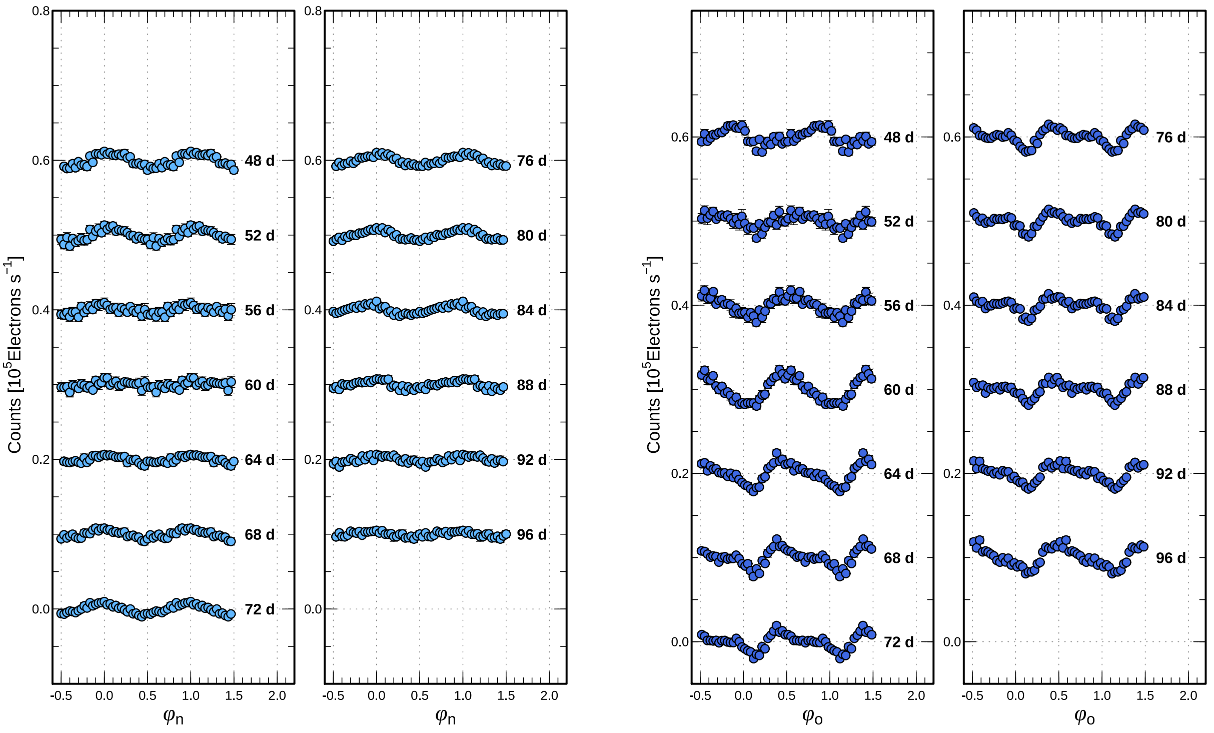


**Fig. E2.** As Fig. E1 but during interval 2 in Fig. 1.

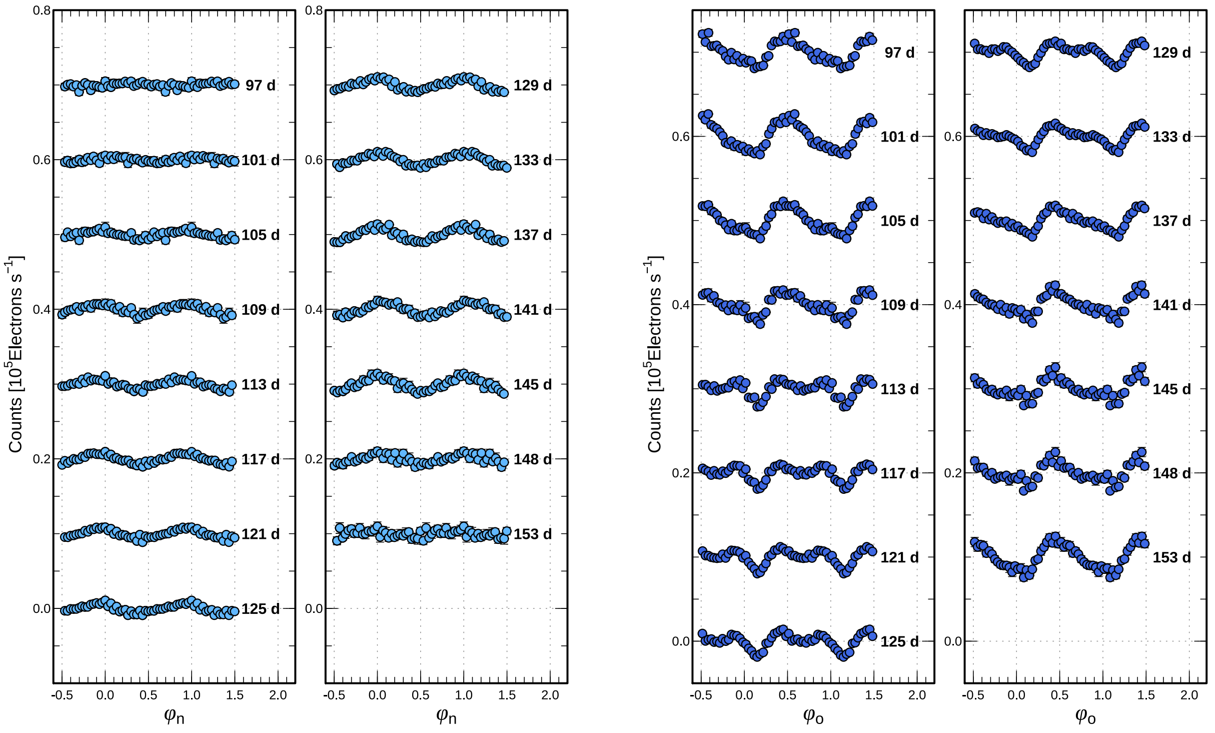


**Fig. E3.** As Fig. E1 but during interval 3 in Fig. 1.

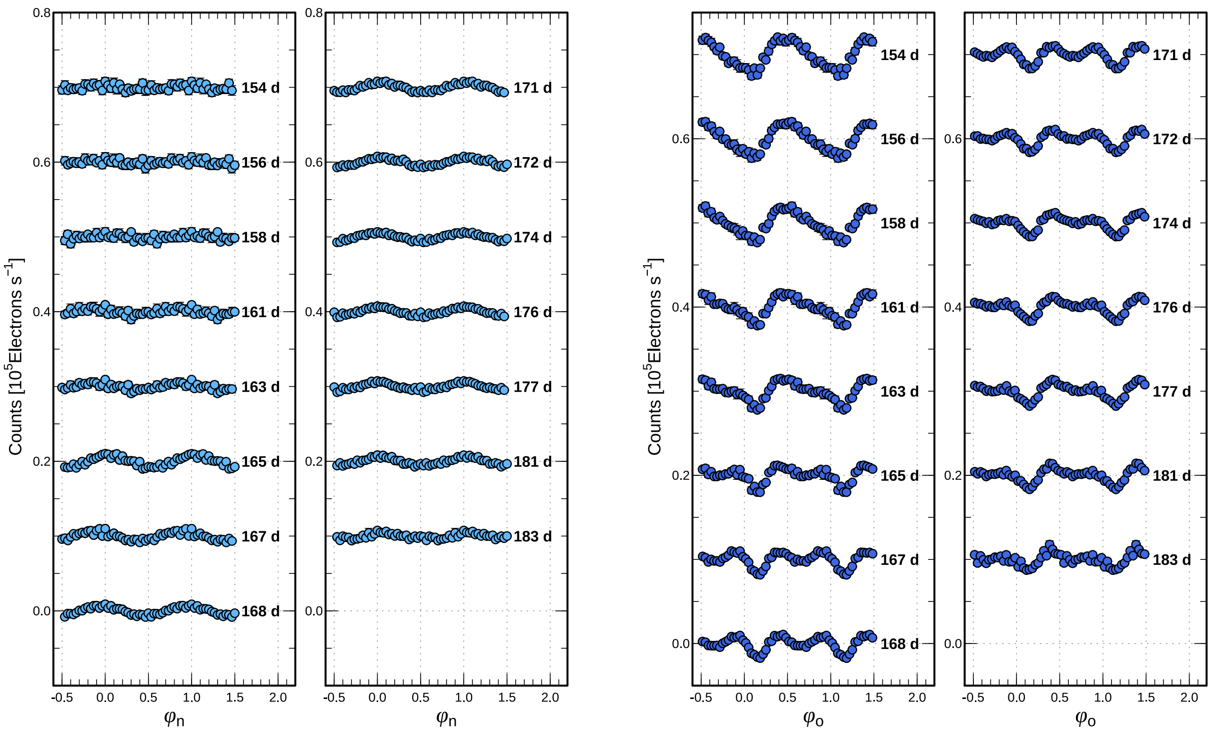


**Fig. E4.** As Fig. E1 but during interval 4 in Fig. 1.

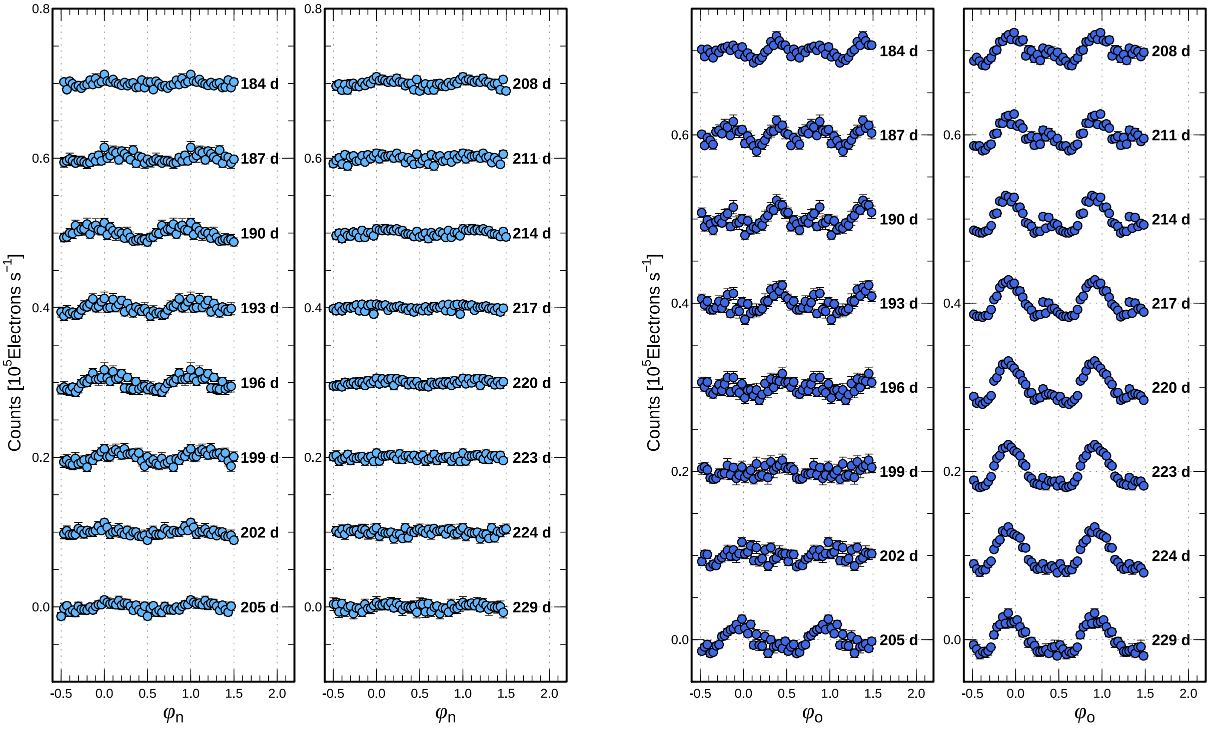


**Fig. E5.** As Fig. E1 but during interval 5 in Fig. 1.

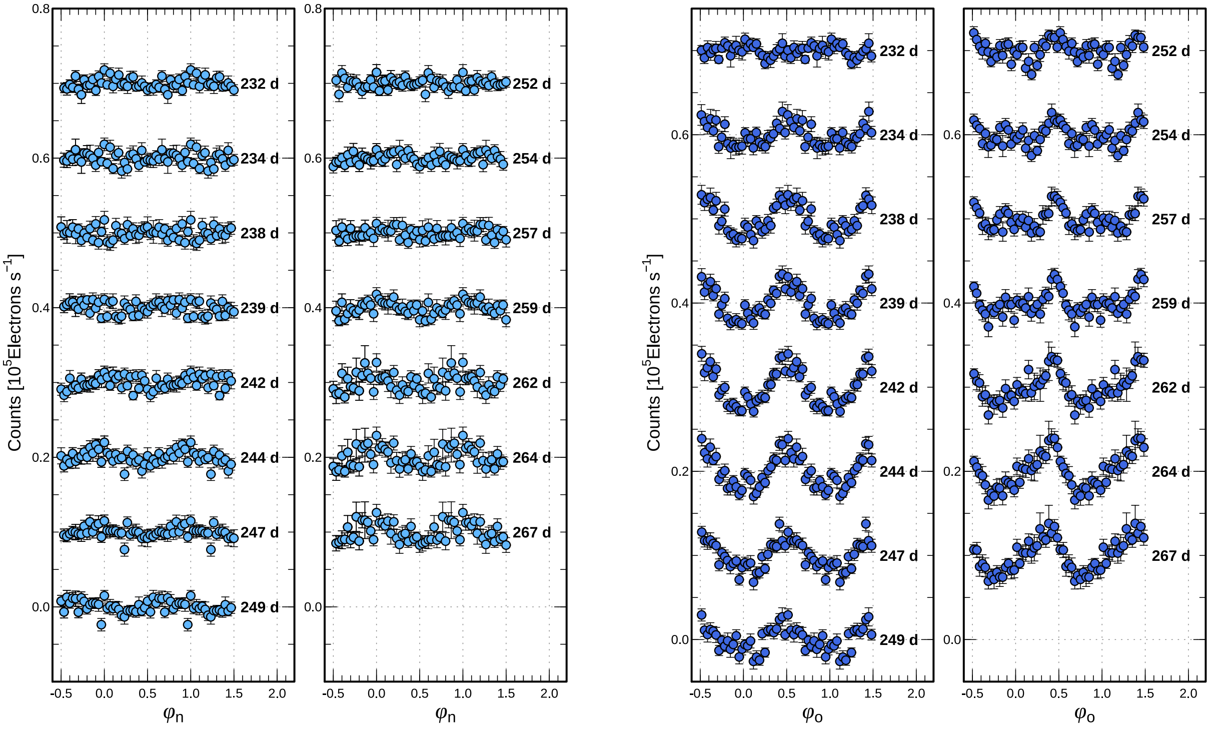


**Fig. E6.** As Fig. E1 but during interval 6 in Fig. 1.

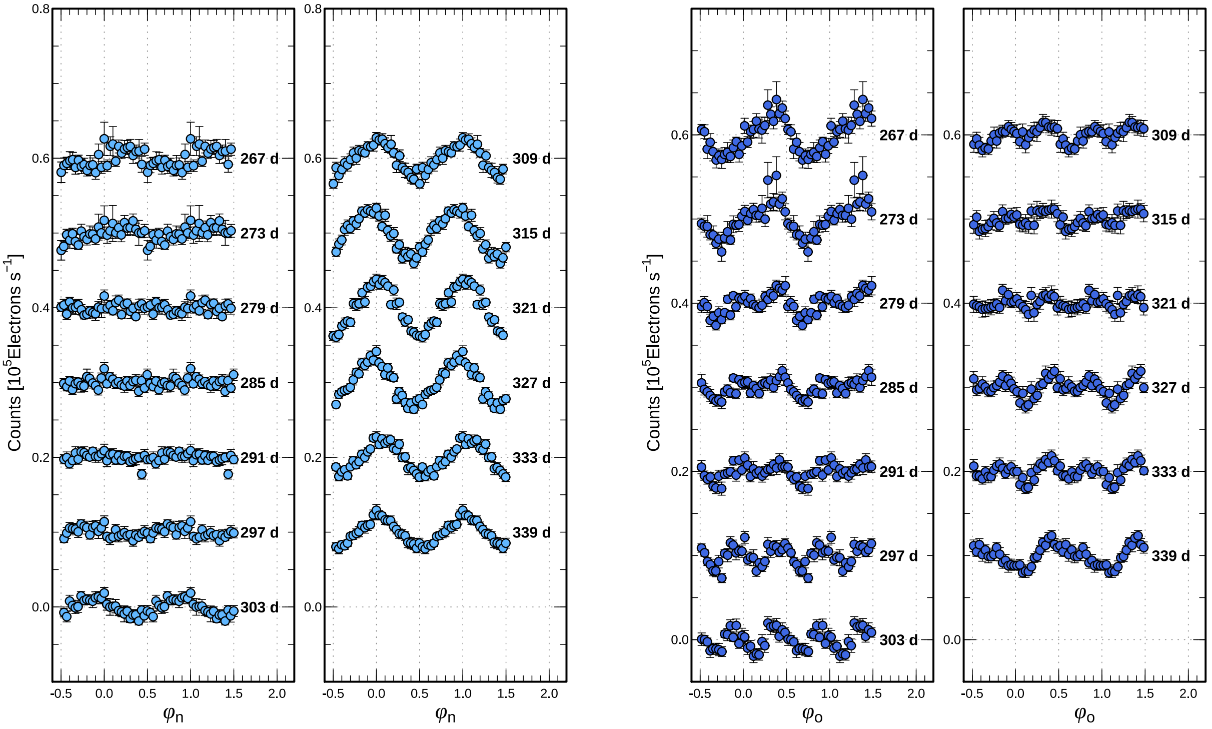


**Fig. E7.** As Fig. E1 but during interval 7 in Fig. 1.

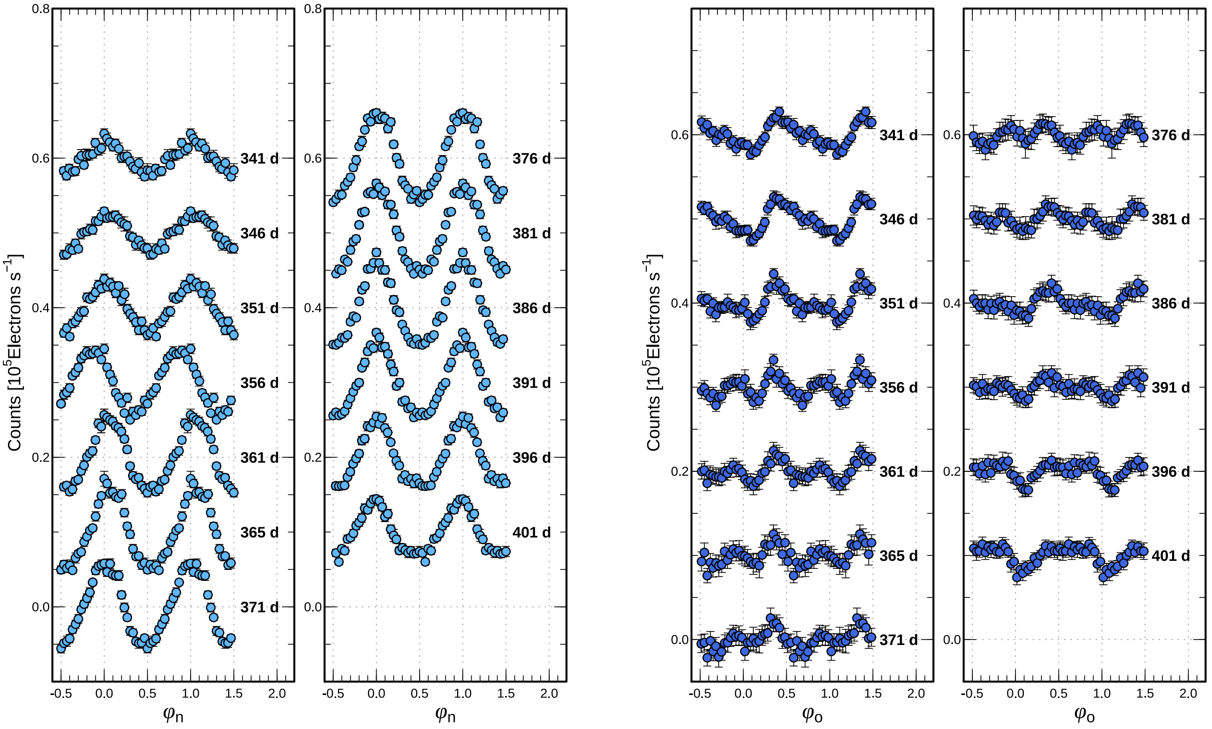


**Fig. E8.** As Fig. E1 but during interval 8 in Fig. 1.

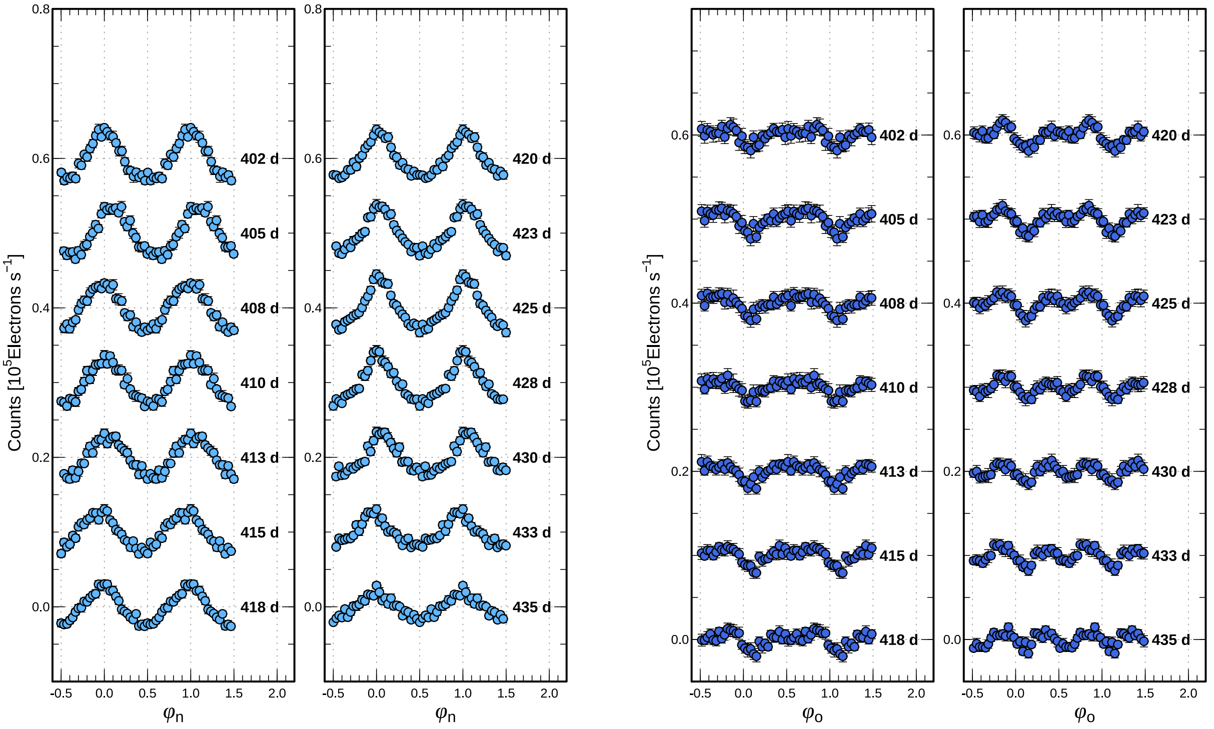


**Fig. E9.** As Fig. E1 but during interval 9 in Fig. 1.

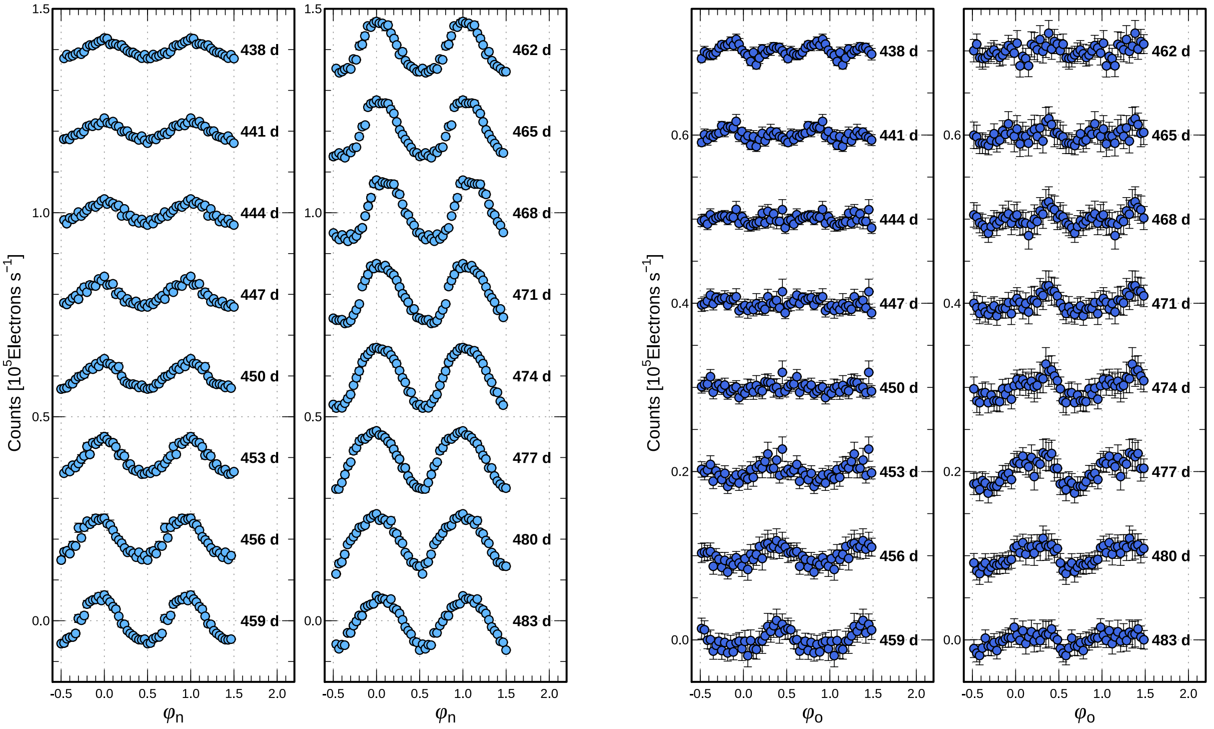


**Fig. E10.** As Fig. E1 but during interval 10 in Fig. 1. The scale of the vertical axis in the left panel is wider because of the large amplitude of negative superhumps.

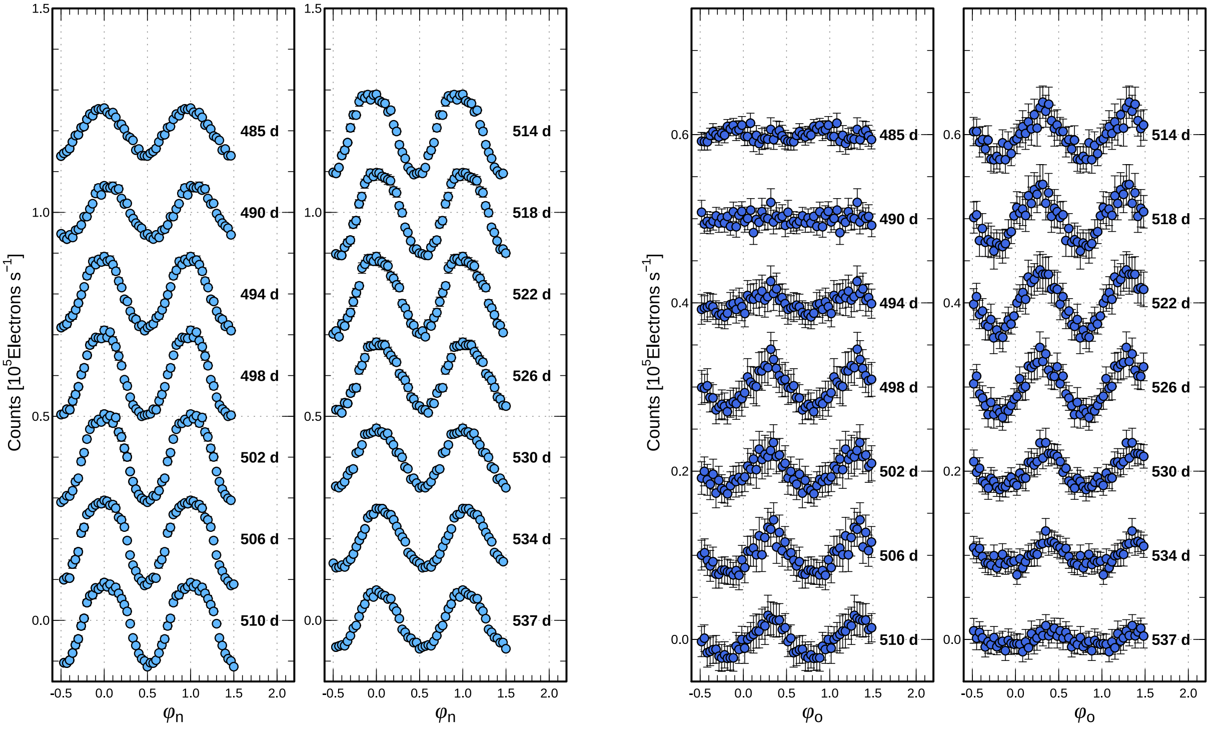

**Fig. E11.** As Fig. E1 but during interval 11 in Fig. 1. The scale of the vertical axis in the left panel is wider because of the large amplitude of negative superhumps.

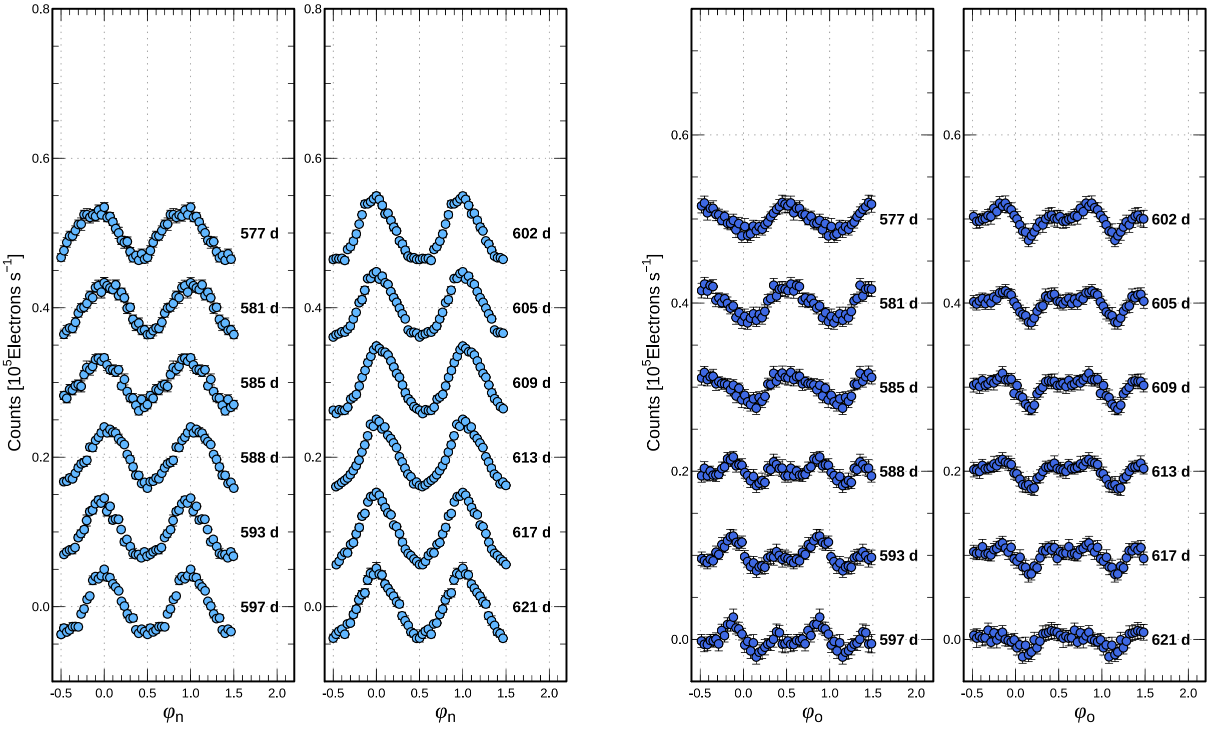

**Fig. E12.** As Fig. E1 but during interval 12 in Fig. 1.

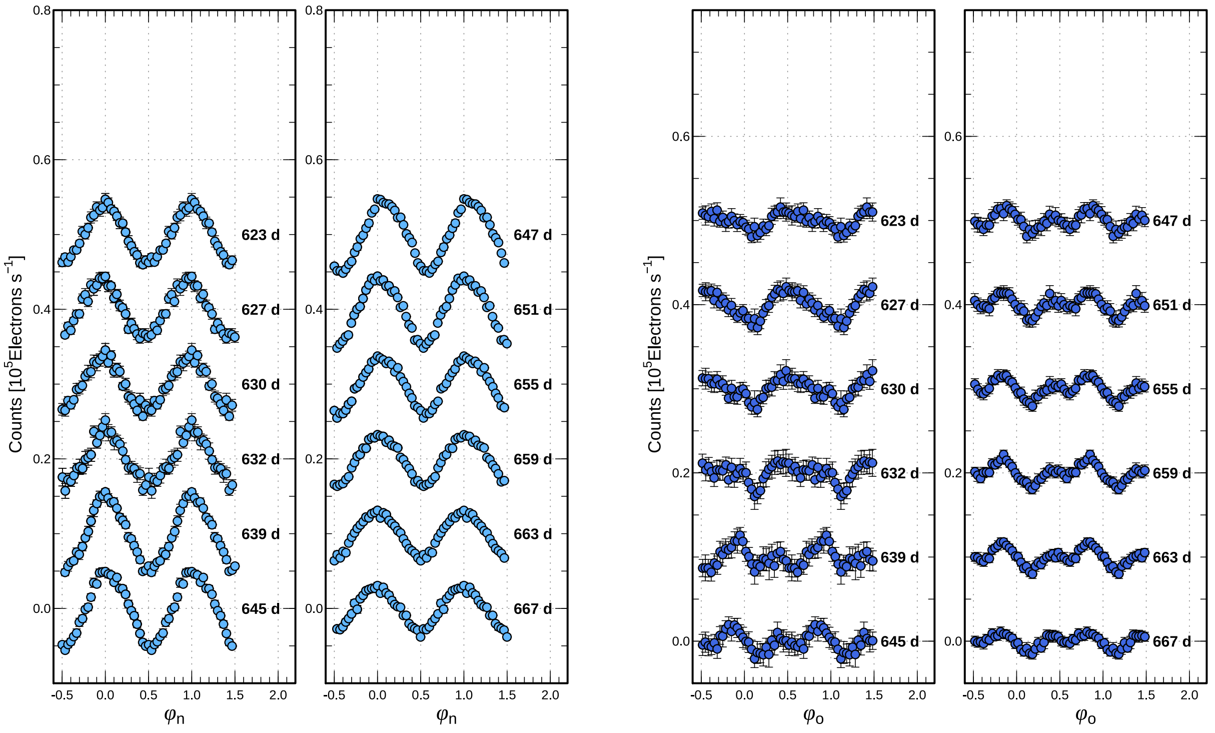


**Fig. E13.** As Fig. E1 but during interval 13 in Fig. 1.

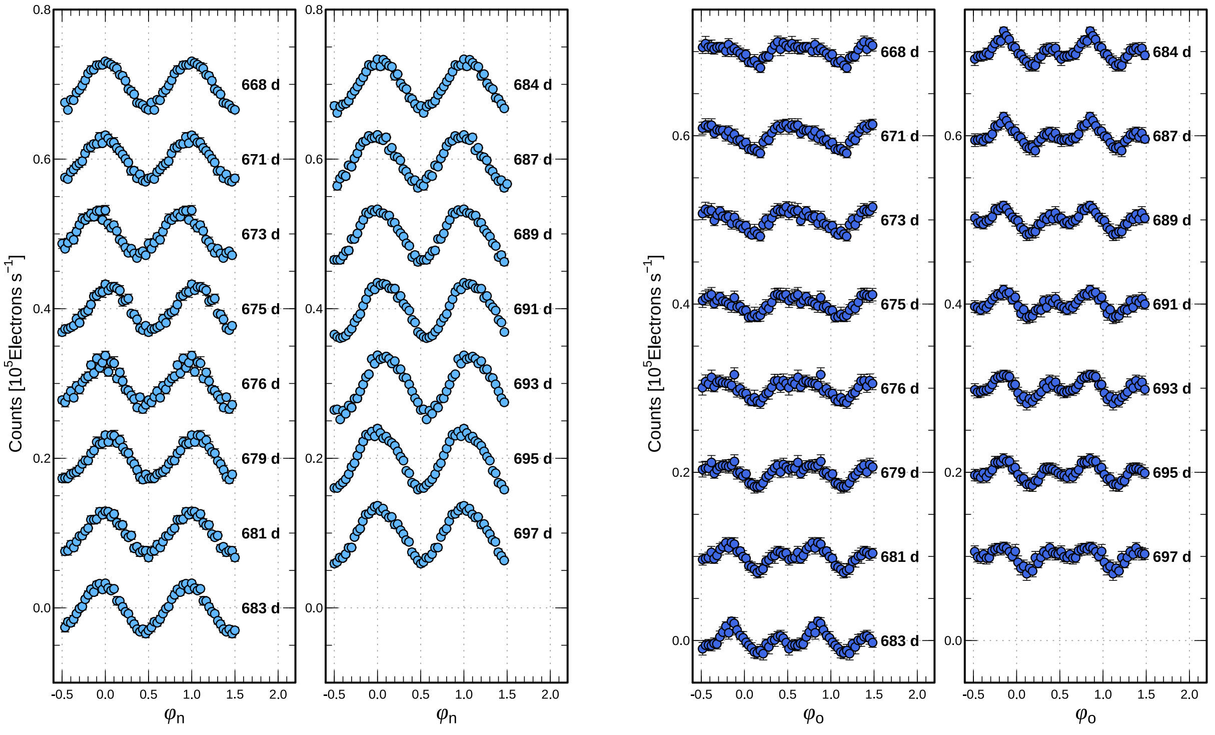


**Fig. E14.** As Fig. E1 but during interval 14 in Fig. 1.

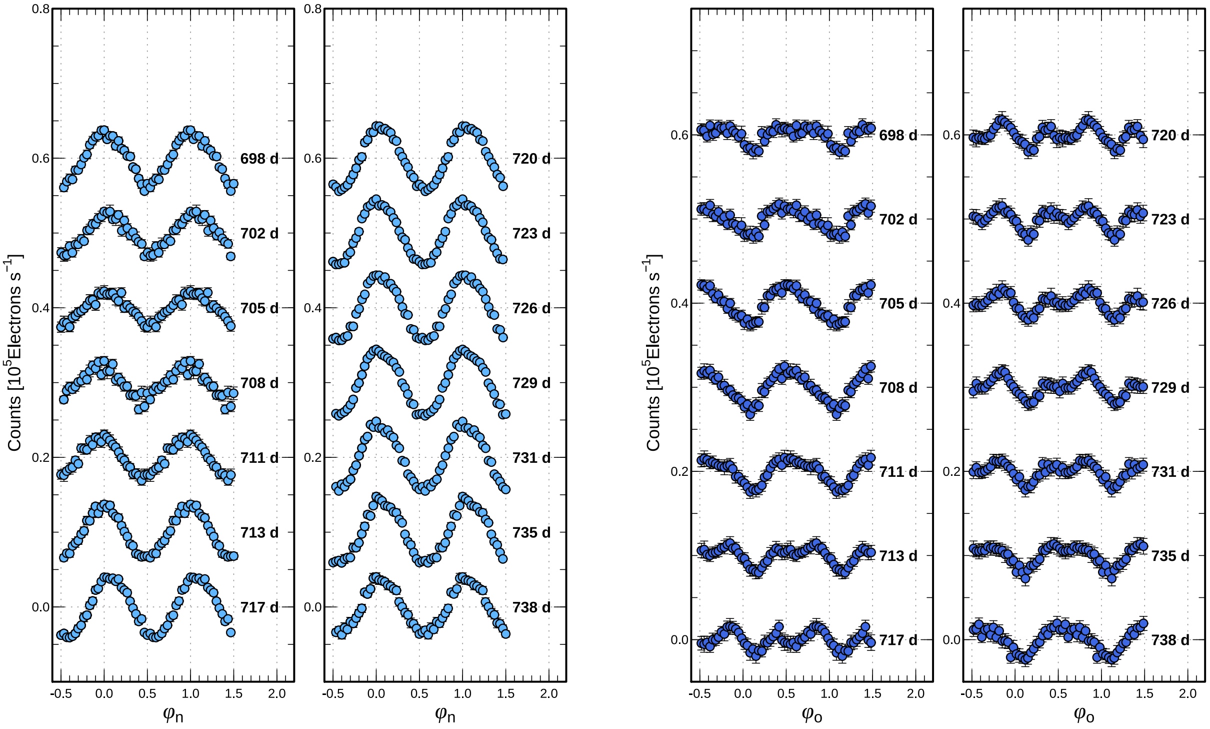

**Fig. E15.** As Fig. E1 but during interval 15 in Fig. 1.

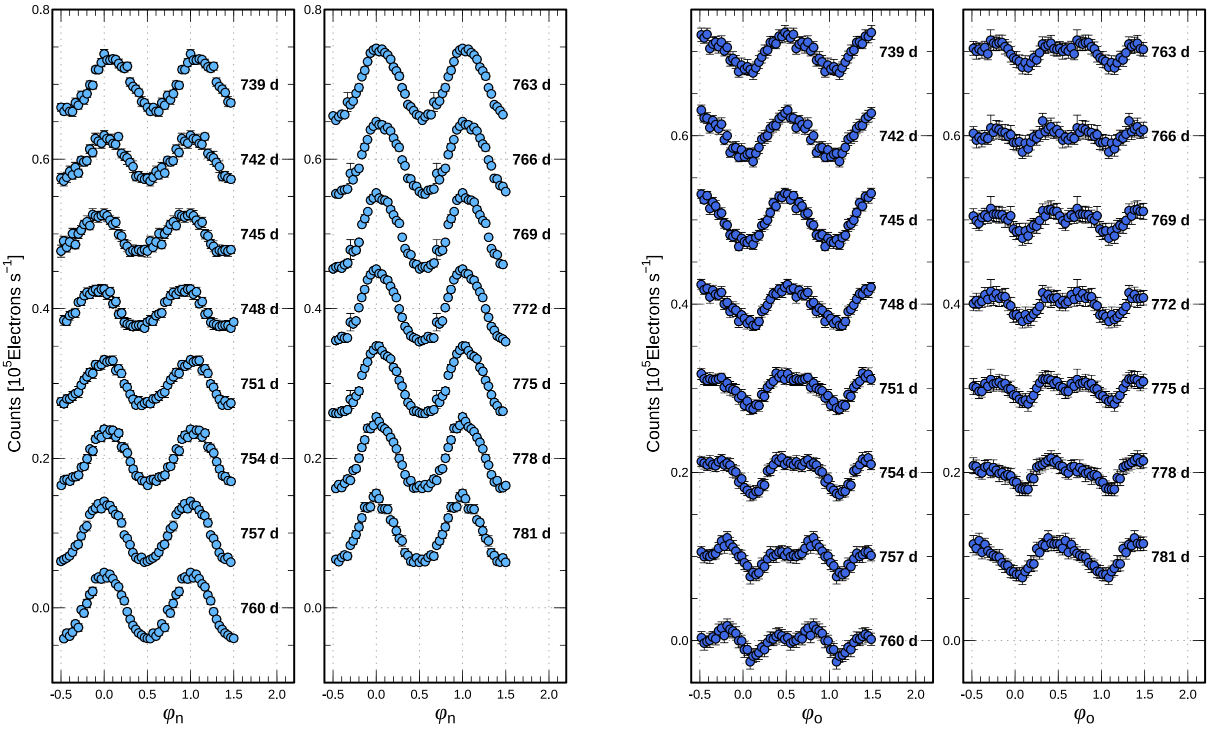

**Fig. E16.** As Fig. E1 but during interval 16 in Fig. 1.

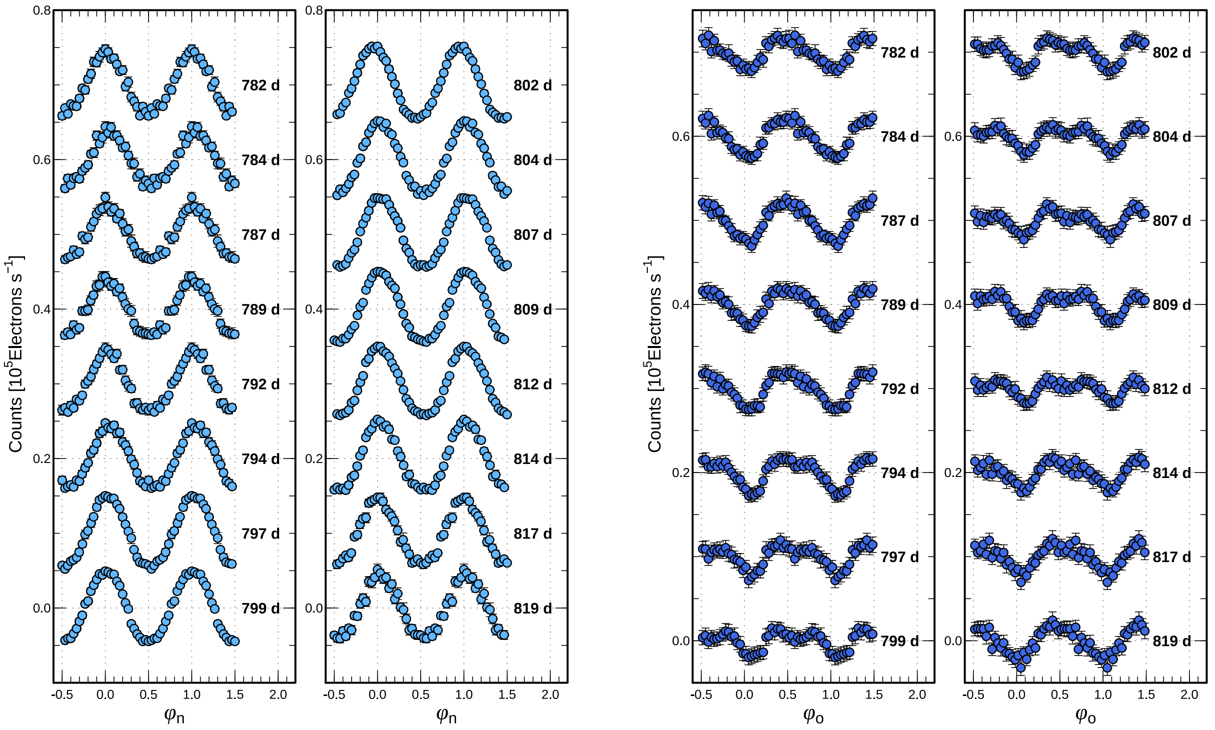


**Fig. E17.** As Fig. E1 but during interval 17 in Fig. 1.

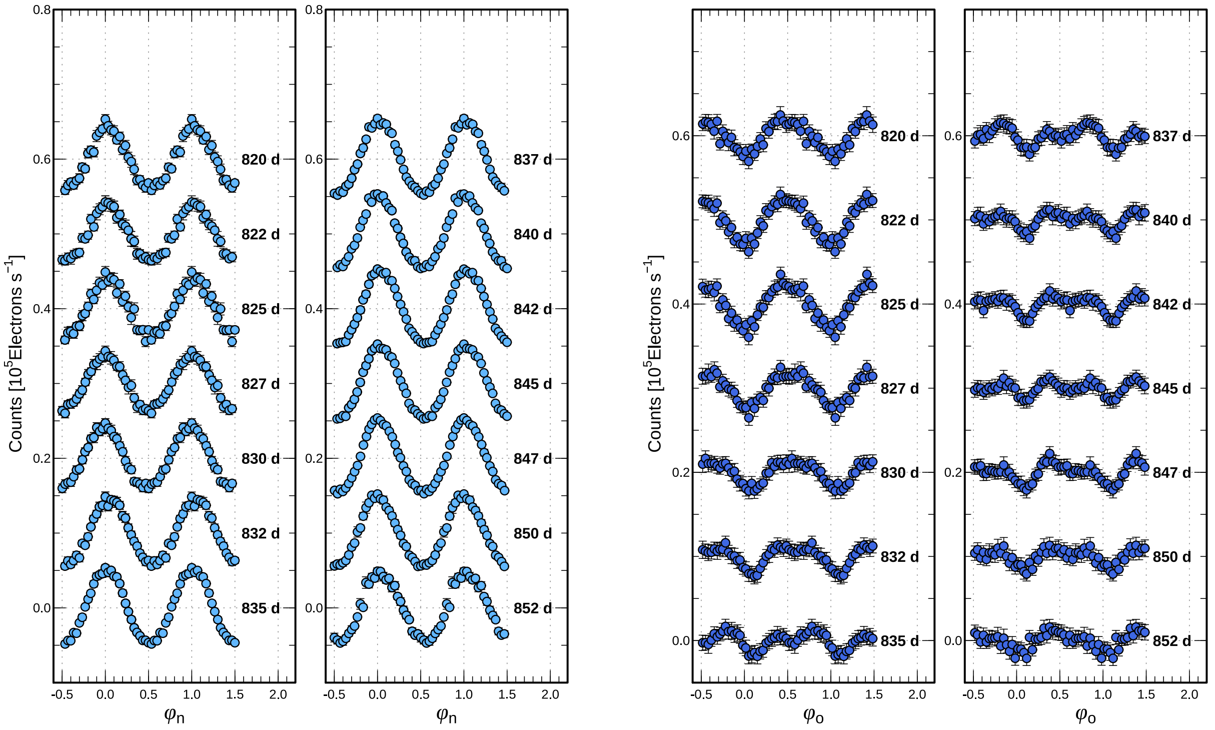


**Fig. E18.** As Fig. E1 but during interval 18 in Fig. 1.

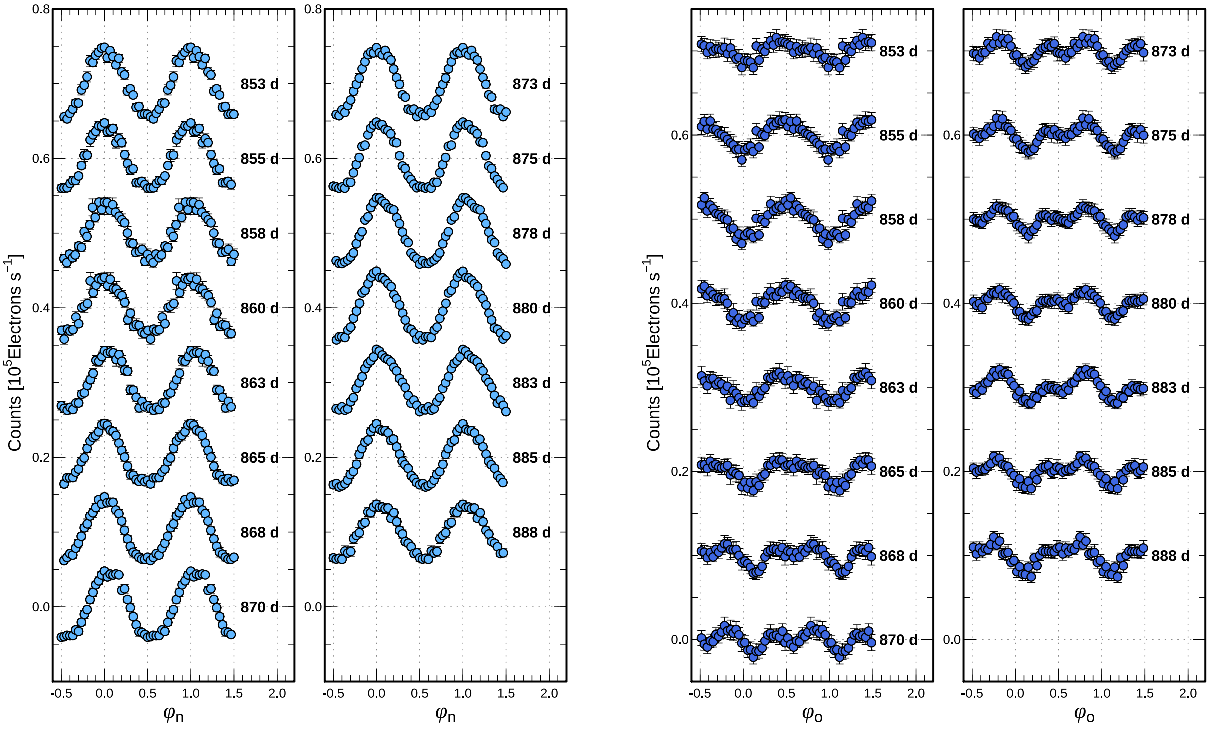


**Fig. E19.** As Fig. E1 but during interval 19 in Fig. 1.

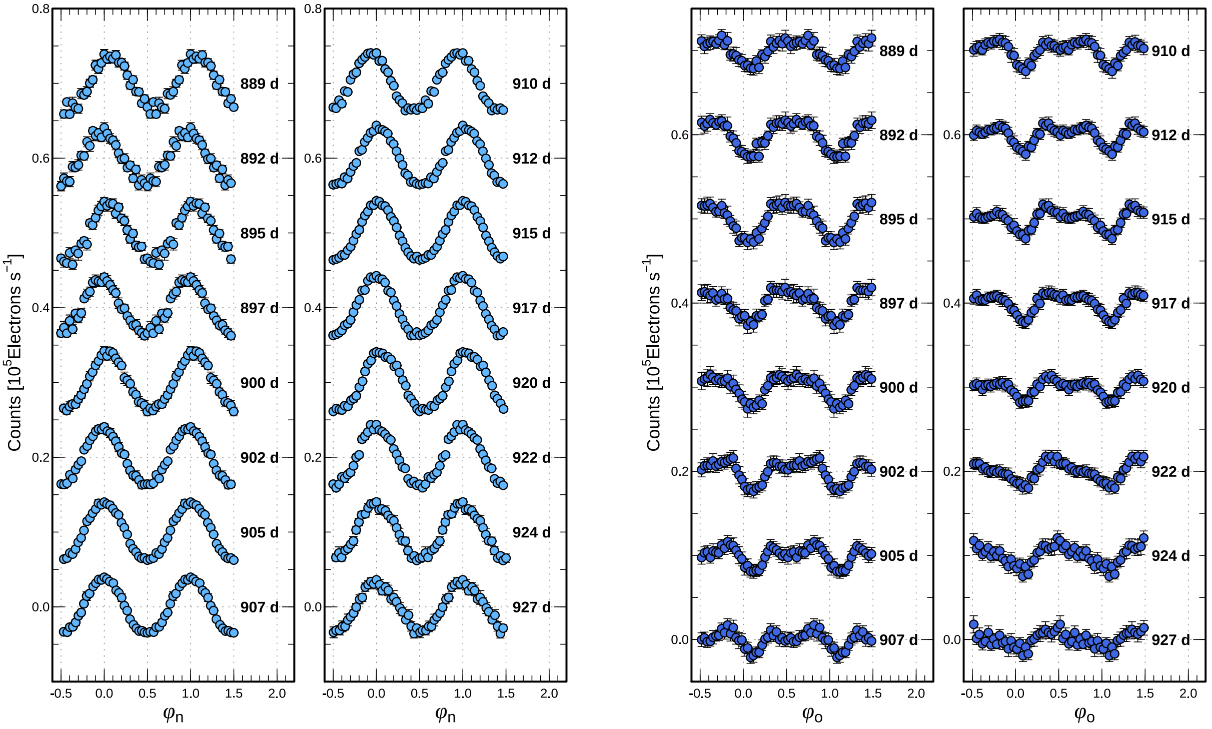


**Fig. E20.** As Fig. E1 but during interval 20 in Fig. 1.

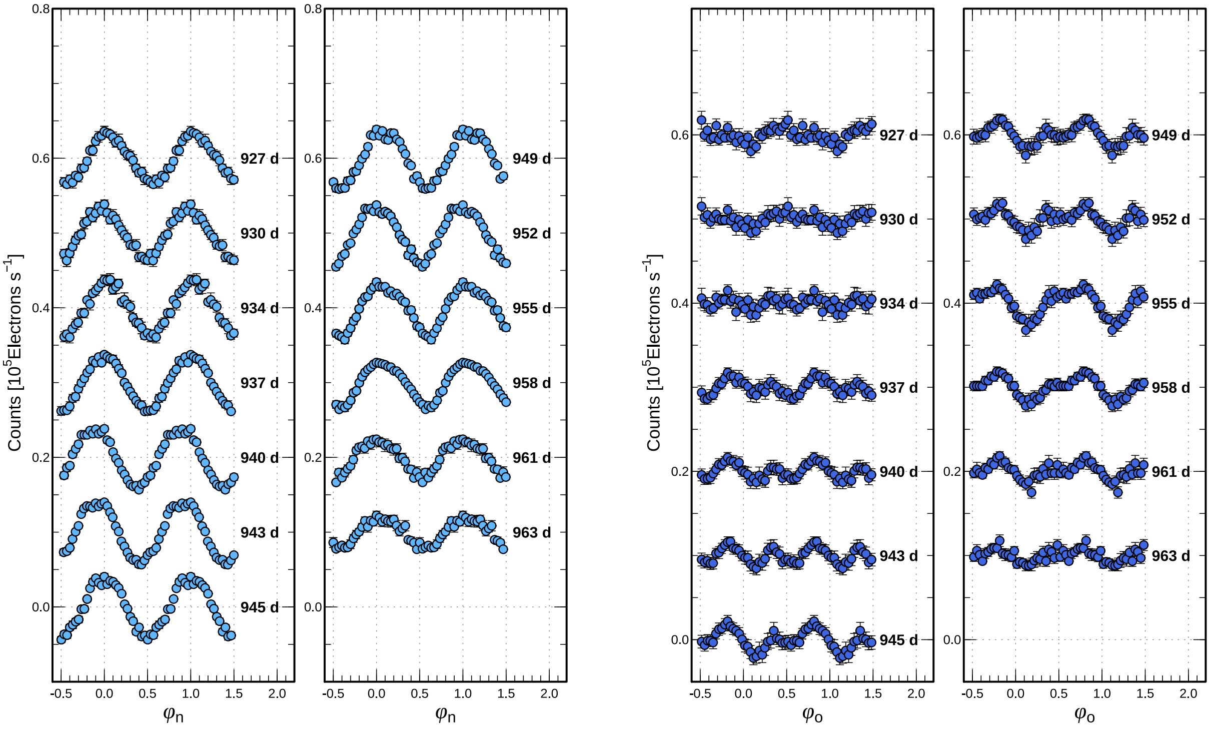


**Fig. E21.** As Fig. E1 but during interval 21 in Fig. 1.

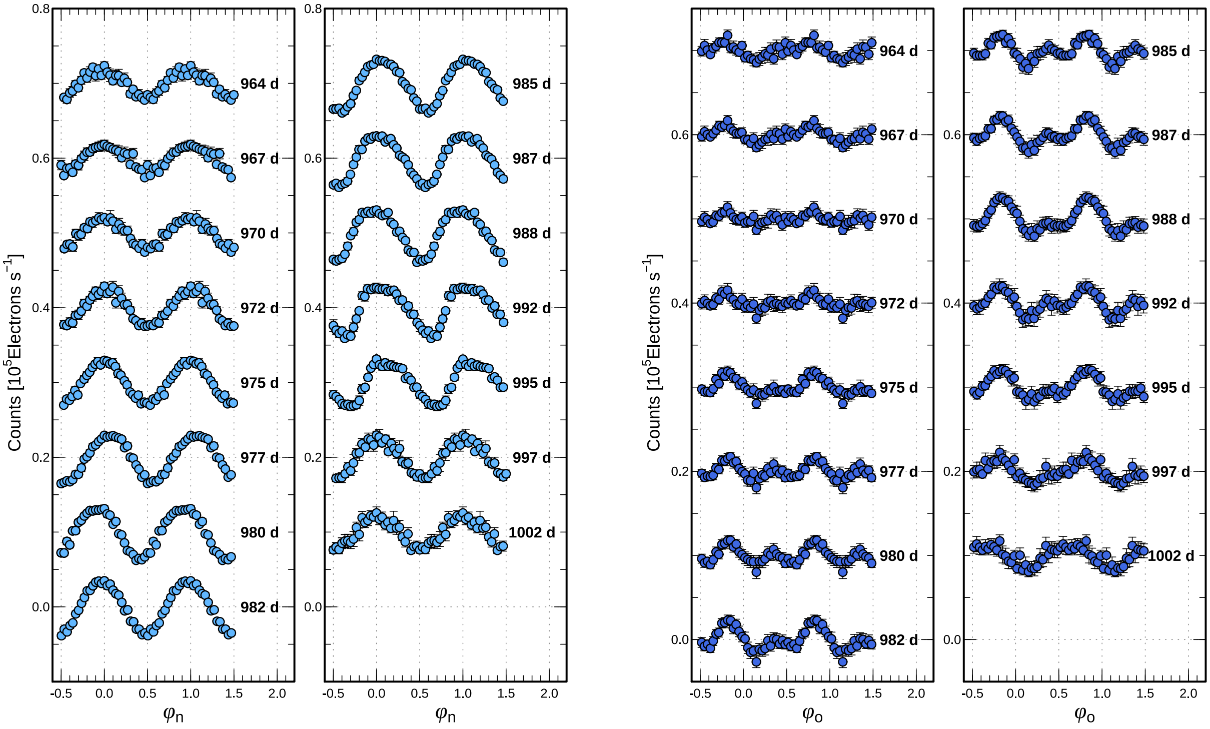


**Fig. E22.** As Fig. E1 but during interval 22 in Fig. 1.

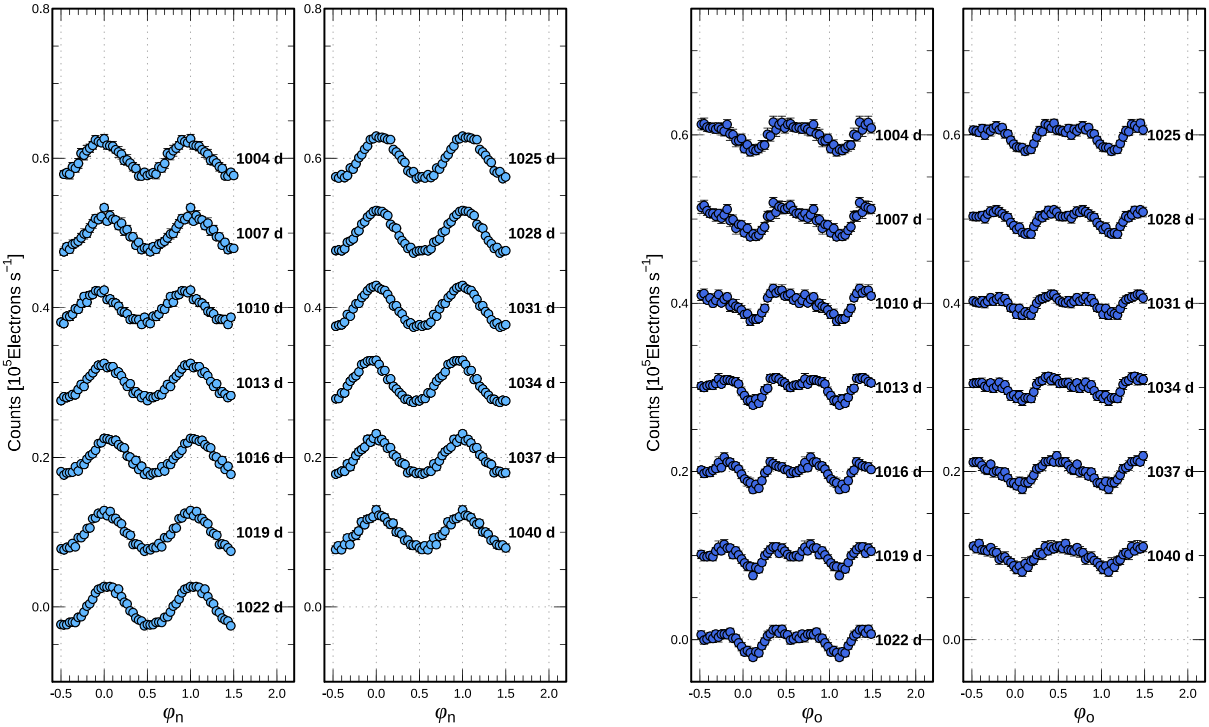


**Fig. E23.** As Fig. E1 but during interval 23 in Fig. 1.

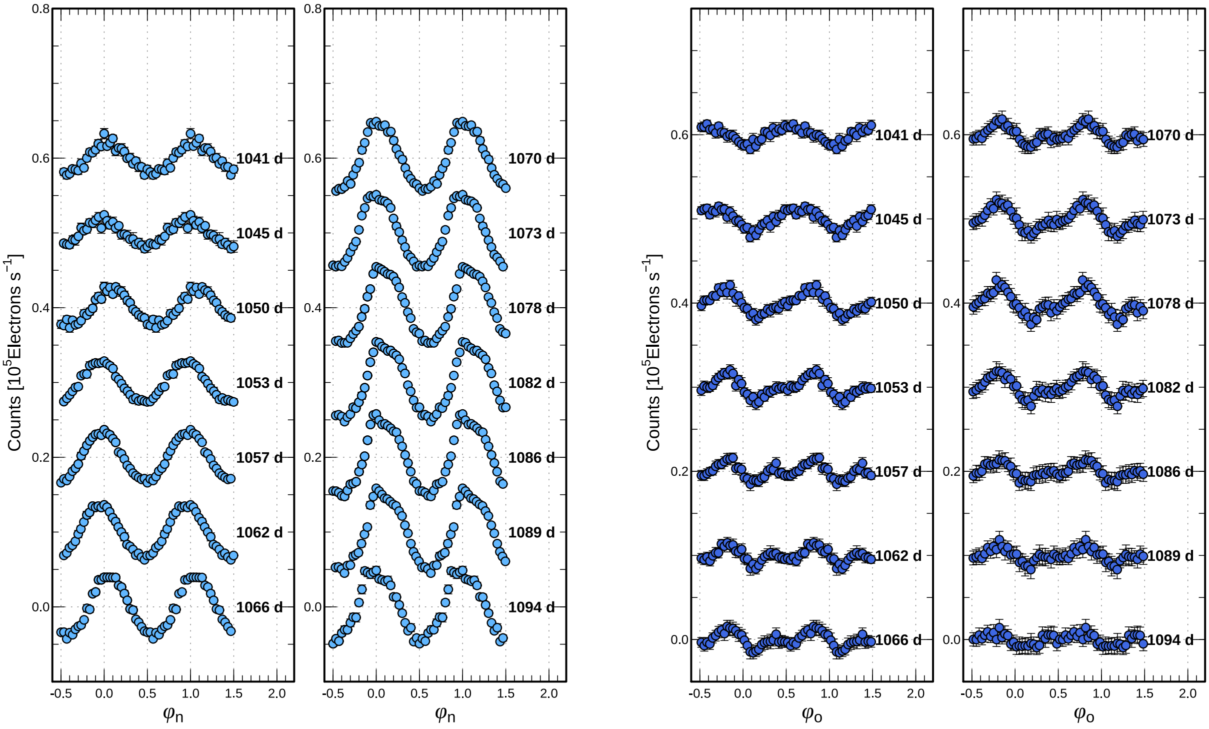


**Fig. E24.** As Fig. E1 but during interval 24 in Fig. 1.

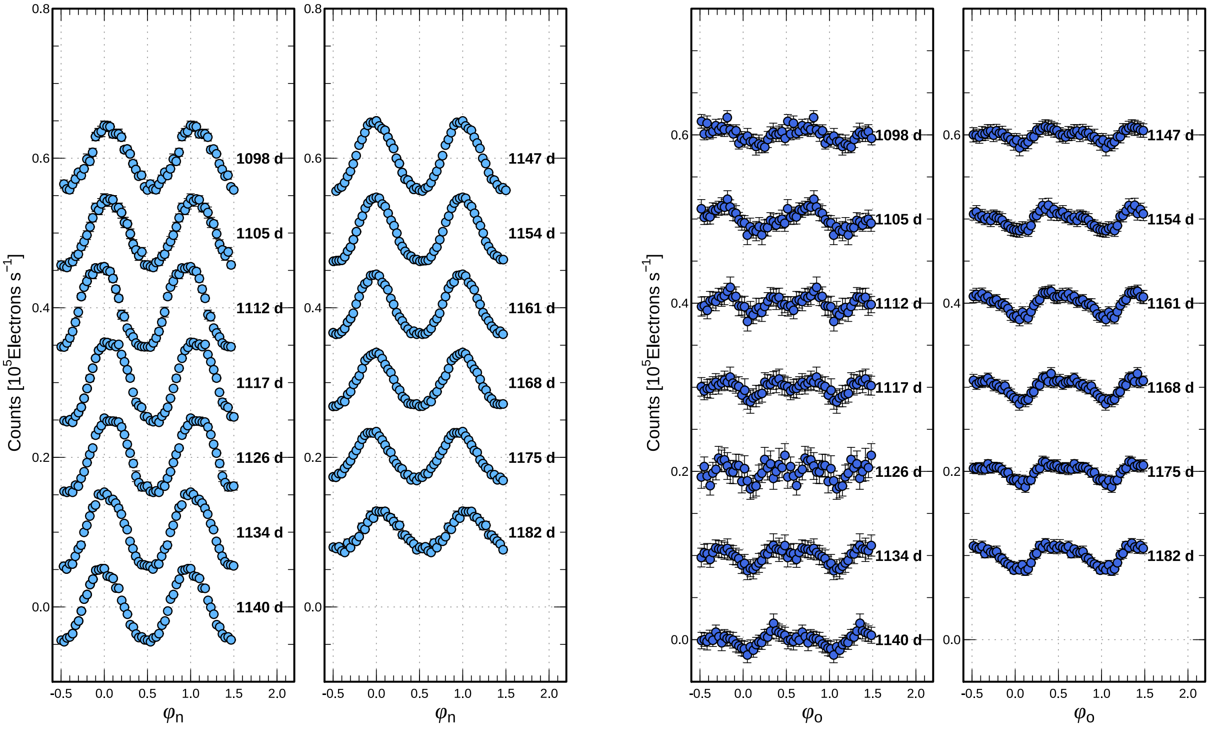


**Fig. E25.** As Fig. E1 but during interval 25 in Fig. 1.

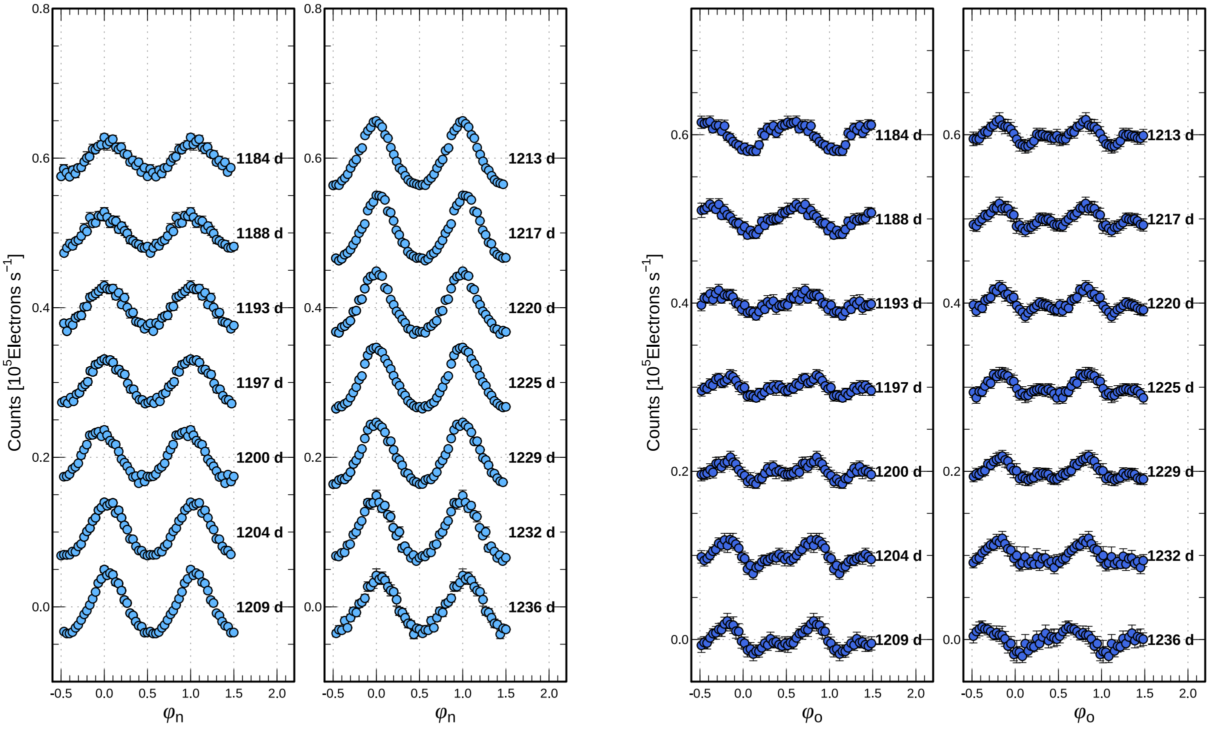


**Fig. E26.** As Fig. E1 but during interval 26 in Fig. 1.

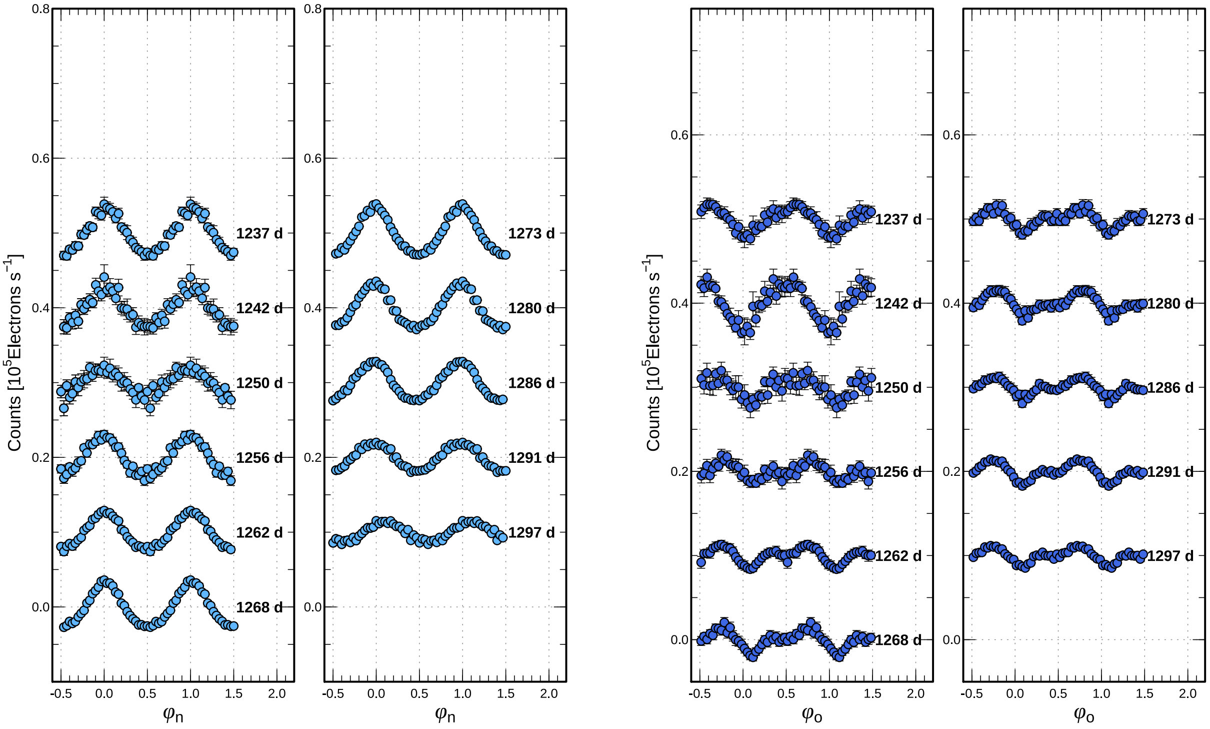


**Fig. E27.** As Fig. E1 but during interval 27 in Fig. 1.

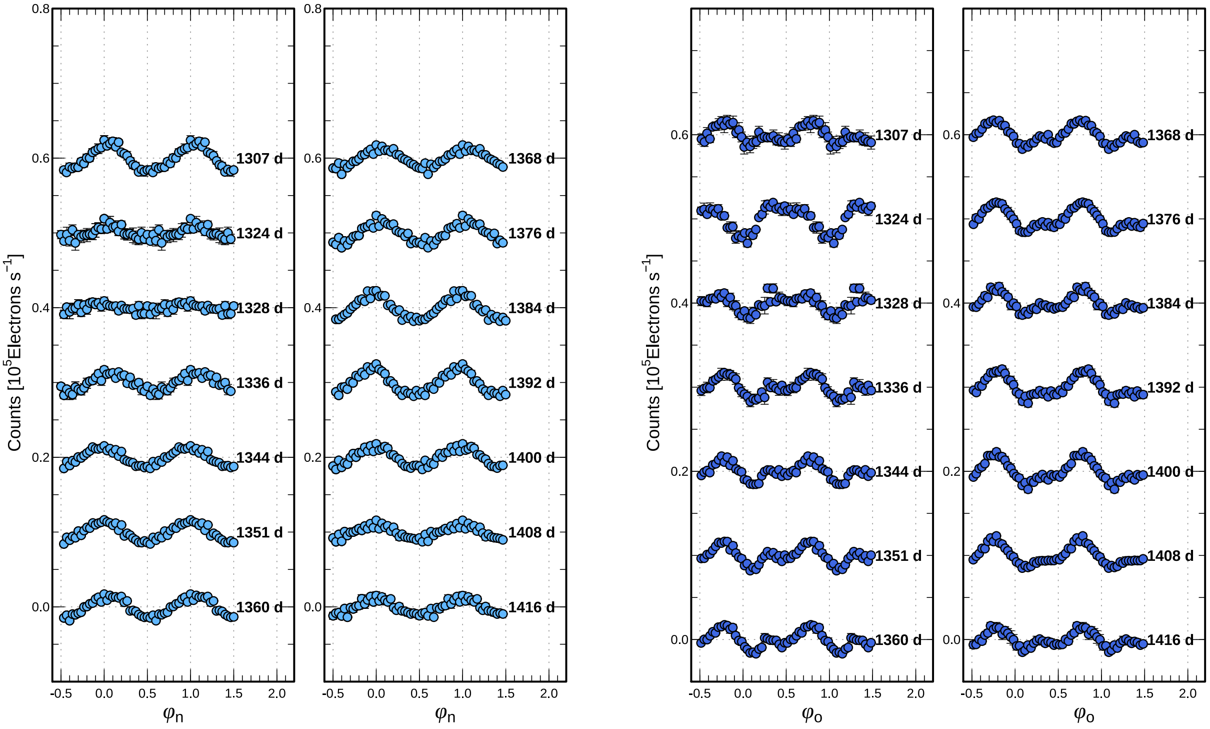


**Fig. E28.** As Fig. E1 but during interval 28 in Fig. 1.

**Table E1.** Times of negative-superhump maxima in KIC 9406652 during time interval 1 (BJD 2455296–2455553).

| $E^*$ | Max$^\dagger$ | Error | $O-C^\ddagger$ | $N^\S$ |
|---|---|---|---|---|
| 0 | 296.7599 | 0.0093 | 0.0375 | 9 |
| 2 | 297.1876 | 0.0147 | -0.0142 | 10 |
| 3 | 297.4414 | 0.0170 | -0.0001 | 9 |
| 4 | 297.6714 | 0.0093 | -0.0098 | 9 |
| 8 | 298.5707 | 0.0095 | -0.0693 | 9 |
| 9 | 298.8922 | 0.0136 | 0.0125 | 9 |
| 11 | 299.3568 | 0.0076 | -0.0023 | 9 |
| 12 | 299.5959 | 0.0134 | -0.0029 | 9 |
| 13 | 299.8291 | 0.0142 | -0.0094 | 10 |
| 16 | 300.5630 | 0.0182 | 0.0054 | 9 |
| 18 | 301.0127 | 0.0099 | -0.0243 | 9 |
| 19 | 301.2451 | 0.0124 | -0.0316 | 9 |
| 22 | 301.9840 | 0.0182 | -0.0118 | 9 |
| 23 | 302.2640 | 0.0130 | 0.0285 | 8 |
| 26 | 302.9566 | 0.0178 | 0.0020 | 9 |
| 30 | 303.8871 | 0.0066 | -0.0263 | 9 |
| 32 | 304.3822 | 0.0124 | -0.0106 | 10 |
| 38 | 305.8597 | 0.0087 | 0.0287 | 9 |
| 40 | 306.2866 | 0.0148 | -0.0238 | 10 |
| 42 | 306.7987 | 0.0057 | 0.0089 | 9 |
| 43 | 306.9872 | 0.0152 | -0.0423 | 10 |
| 45 | 307.5167 | 0.0064 | 0.0078 | 9 |
| 47 | 308.0514 | 0.0059 | 0.0631 | 6 |
| 53 | 309.4302 | 0.0176 | 0.0037 | 9 |
| 55 | 309.9118 | 0.0130 | 0.0059 | 9 |
| 56 | 310.1909 | 0.0144 | 0.0453 | 9 |
| 57 | 310.3676 | 0.0163 | -0.0177 | 9 |
| 58 | 310.6248 | 0.0045 | -0.0002 | 10 |
| 59 | 310.8507 | 0.0085 | -0.0140 | 8 |
| 60 | 311.1510 | 0.0099 | 0.0466 | 9 |
| 61 | 311.3467 | 0.0186 | 0.0026 | 9 |
| 62 | 311.5549 | 0.0066 | -0.0289 | 10 |
| 63 | 311.8006 | 0.0117 | -0.0229 | 9 |
| 64 | 312.0333 | 0.0068 | -0.0299 | 9 |
| 65 | 312.2984 | 0.0106 | -0.0045 | 10 |
| 66 | 312.5037 | 0.0113 | -0.0389 | 10 |
| 67 | 312.8080 | 0.0119 | 0.0257 | 9 |
| 68 | 313.0040 | 0.0078 | -0.0180 | 9 |
| 69 | 313.2976 | 0.0110 | 0.0359 | 10 |
| 70 | 313.4670 | 0.0130 | -0.0344 | 9 |
| 72 | 313.9484 | 0.0148 | -0.0324 | 10 |
| 73 | 314.2210 | 0.0103 | 0.0005 | 10 |
| 75 | 314.6868 | 0.0078 | -0.0131 | 9 |
| 77 | 315.1677 | 0.0046 | -0.0116 | 10 |
| 78 | 315.4204 | 0.0106 | 0.0014 | 9 |
| 79 | 315.6685 | 0.0111 | 0.0098 | 9 |
| 80 | 315.8887 | 0.0056 | -0.0097 | 10 |
| 81 | 316.1518 | 0.0124 | 0.0137 | 9 |
| 82 | 316.3841 | 0.0136 | 0.0063 | 9 |
| 83 | 316.5826 | 0.0116 | -0.0349 | 9 |
| 85 | 317.0656 | 0.0109 | -0.0313 | 9 |
| 86 | 317.3550 | 0.0048 | 0.0184 | 9 |

**Table E1.** Times of negative-superhump maxima in KIC 9406652 during time interval 1 (BJD 2455296–2455553) (continued).

| $E^*$ | Max$^\dagger$ | Error | $O-C^\ddagger$ | $N^\S$ |
|---|---|---|---|---|
| 88 | 317.7942 | 0.0062 | -0.0218 | 10 |
| 89 | 318.0401 | 0.0072 | -0.0156 | 9 |
| 90 | 318.2684 | 0.0061 | -0.0270 | 9 |
| 91 | 318.5165 | 0.0068 | -0.0186 | 10 |
| 92 | 318.7536 | 0.0190 | -0.0212 | 9 |
| 93 | 319.0114 | 0.0112 | -0.0031 | 9 |
| 94 | 319.2303 | 0.0127 | -0.0239 | 9 |
| 95 | 319.4638 | 0.0108 | -0.0301 | 10 |
| 96 | 319.7740 | 0.0185 | 0.0404 | 8 |
| 97 | 319.9626 | 0.0157 | -0.0107 | 8 |
| 98 | 320.1906 | 0.0097 | -0.0224 | 10 |
| 99 | 320.4188 | 0.0115 | -0.0339 | 10 |
| 100 | 320.6765 | 0.0055 | -0.0159 | 9 |
| 101 | 320.9504 | 0.0101 | 0.0183 | 9 |
| 102 | 321.1340 | 0.0081 | -0.0378 | 10 |
| 103 | 321.4180 | 0.0034 | 0.0065 | 10 |
| 104 | 321.6342 | 0.0101 | -0.0170 | 9 |
| 105 | 321.8949 | 0.0104 | 0.0040 | 9 |
| 106 | 322.1196 | 0.0060 | -0.0110 | 9 |
| 107 | 322.3740 | 0.0107 | 0.0037 | 9 |
| 109 | 322.8202 | 0.0047 | -0.0295 | 8 |
| 110 | 323.0701 | 0.0086 | -0.0193 | 10 |
| 111 | 323.2944 | 0.0052 | -0.0347 | 9 |
| 112 | 323.5521 | 0.0041 | -0.0167 | 9 |
| 113 | 323.7838 | 0.0045 | -0.0247 | 10 |
| 114 | 324.0366 | 0.0042 | -0.0116 | 10 |
| 115 | 324.2896 | 0.0072 | 0.0017 | 9 |
| 116 | 324.5193 | 0.0061 | -0.0083 | 9 |
| 117 | 324.7421 | 0.0060 | -0.0252 | 10 |
| 118 | 325.0073 | 0.0084 | 0.0003 | 9 |
| 119 | 325.2451 | 0.0055 | -0.0016 | 9 |
| 120 | 325.4877 | 0.0054 | 0.0013 | 9 |
| 121 | 325.7330 | 0.0028 | 0.0069 | 9 |
| 122 | 325.9802 | 0.0053 | 0.0144 | 9 |
| 124 | 326.4591 | 0.0096 | 0.0139 | 9 |
| 126 | 326.8916 | 0.0077 | -0.0330 | 9 |
| 127 | 327.1356 | 0.0100 | -0.0287 | 9 |
| 128 | 327.3862 | 0.0063 | -0.0178 | 10 |
| 129 | 327.6639 | 0.0041 | 0.0202 | 10 |
| 130 | 327.8637 | 0.0085 | -0.0197 | 9 |
| 131 | 328.1116 | 0.0034 | -0.0115 | 9 |
| 132 | 328.3678 | 0.0067 | 0.0050 | 10 |
| 133 | 328.5882 | 0.0065 | -0.0143 | 9 |
| 134 | 328.8208 | 0.0085 | -0.0214 | 9 |
| 135 | 329.0653 | 0.0173 | -0.0166 | 9 |
| 136 | 329.3153 | 0.0069 | -0.0063 | 10 |
| 137 | 329.5883 | 0.0186 | 0.0270 | 9 |
| 138 | 329.8098 | 0.0057 | 0.0088 | 9 |
| 139 | 330.0289 | 0.0094 | -0.0118 | 10 |
| 140 | 330.2477 | 0.0151 | -0.0327 | 10 |
| 141 | 330.4847 | 0.0092 | -0.0354 | 9 |
| 142 | 330.8114 | 0.0182 | 0.0516 | 9 |

**Table E1.** Times of negative-superhump maxima in KIC 9406652 during time interval 1 (BJD 2455296–2455553) (continued).

| $E^*$ | Max$^\dagger$ | Error | $O-C^\ddagger$ | $N^\S$ |
|---|---|---|---|---|
| 144 | 331.2243 | 0.0061 | -0.0149 | 9 |
| 146 | 331.6933 | 0.0180 | -0.0253 | 8 |
| 147 | 331.9886 | 0.0188 | 0.0303 | 10 |
| 148 | 332.1780 | 0.0109 | -0.0200 | 9 |
| 149 | 332.4045 | 0.0129 | -0.0332 | 9 |
| 150 | 332.6594 | 0.0071 | -0.0180 | 10 |
| 151 | 332.8975 | 0.0050 | -0.0196 | 10 |
| 153 | 333.4122 | 0.0059 | 0.0157 | 9 |
| 154 | 333.6118 | 0.0155 | -0.0244 | 10 |
| 155 | 333.8414 | 0.0087 | -0.0345 | 9 |
| 158 | 334.6048 | 0.0184 | 0.0098 | 10 |
| 161 | 335.2882 | 0.0095 | -0.0259 | 10 |
| 162 | 335.5535 | 0.0177 | -0.0003 | 10 |
| 164 | 336.0080 | 0.0097 | -0.0252 | 9 |
| 165 | 336.2398 | 0.0078 | -0.0331 | 10 |
| 166 | 336.4933 | 0.0083 | -0.0193 | 10 |
| 167 | 336.7310 | 0.0069 | -0.0213 | 8 |
| 171 | 337.6715 | 0.0172 | -0.0396 | 9 |
| 172 | 337.9471 | 0.0050 | -0.0037 | 9 |
| 173 | 338.1756 | 0.0065 | -0.0149 | 10 |
| 174 | 338.4065 | 0.0127 | -0.0237 | 9 |
| 175 | 338.6246 | 0.0121 | -0.0453 | 9 |
| 176 | 338.8775 | 0.0097 | -0.0321 | 10 |
| 177 | 339.1163 | 0.0088 | -0.0330 | 10 |
| 178 | 339.3628 | 0.0196 | -0.0262 | 9 |
| 179 | 339.5771 | 0.0085 | -0.0516 | 9 |
| 181 | 340.0566 | 0.0077 | -0.0515 | 9 |
| 182 | 340.3140 | 0.0082 | -0.0338 | 9 |
| 183 | 340.5433 | 0.0092 | -0.0442 | 9 |
| 184 | 340.8103 | 0.0077 | -0.0169 | 10 |
| 185 | 341.0289 | 0.0042 | -0.0380 | 9 |
| 186 | 341.3020 | 0.0058 | -0.0046 | 9 |
| 187 | 341.5314 | 0.0034 | -0.0149 | 10 |
| 188 | 341.7610 | 0.0073 | -0.0250 | 10 |
| 189 | 342.0164 | 0.0054 | -0.0093 | 9 |
| 190 | 342.2715 | 0.0047 | 0.0061 | 9 |
| 192 | 342.7285 | 0.0134 | -0.0163 | 9 |
| 193 | 342.9946 | 0.0139 | 0.0101 | 9 |
| 196 | 343.6938 | 0.0057 | -0.0098 | 9 |
| 202 | 345.0870 | 0.0080 | -0.0548 | 10 |
| 203 | 345.3278 | 0.0104 | -0.0537 | 10 |
| 204 | 345.5662 | 0.0126 | -0.0550 | 9 |
| 205 | 345.8218 | 0.0176 | -0.0391 | 8 |
| 206 | 346.0654 | 0.0050 | -0.0352 | 10 |
| 207 | 346.3372 | 0.0069 | -0.0031 | 9 |
| 208 | 346.5836 | 0.0058 | 0.0036 | 9 |
| 209 | 346.8298 | 0.0082 | 0.0101 | 9 |
| 210 | 347.0933 | 0.0160 | 0.0339 | 10 |
| 211 | 347.3357 | 0.0188 | 0.0366 | 9 |
| 213 | 347.7809 | 0.0135 | 0.0024 | 10 |
| 215 | 348.2469 | 0.0050 | -0.0110 | 9 |
| 216 | 348.4697 | 0.0183 | -0.0279 | 9 |

**Table E1.** Times of negative-superhump maxima in KIC 9406652 during time interval 1 (BJD 2455296–2455553) (continued).

| $E^*$ | Max$^\dagger$ | Error | $O-C^\ddagger$ | $N^\S$ |
|---|---|---|---|---|
| 218 | 348.9435 | 0.0147 | -0.0335 | 9 |
| 219 | 349.2335 | 0.0175 | 0.0168 | 9 |
| 220 | 349.4522 | 0.0062 | -0.0042 | 9 |
| 221 | 349.7150 | 0.0036 | 0.0189 | 10 |
| 222 | 349.9341 | 0.0095 | -0.0017 | 8 |
| 224 | 350.4462 | 0.0066 | 0.0310 | 10 |
| 225 | 350.6756 | 0.0104 | 0.0207 | 9 |
| 226 | 350.9135 | 0.0058 | 0.0189 | 9 |
| 227 | 351.1486 | 0.0122 | 0.0143 | 9 |
| 228 | 351.4173 | 0.0047 | 0.0433 | 10 |
| 229 | 351.6534 | 0.0060 | 0.0397 | 9 |
| 231 | 352.1183 | 0.0106 | 0.0252 | 9 |
| 232 | 352.3709 | 0.0069 | 0.0381 | 10 |
| 233 | 352.5941 | 0.0105 | 0.0216 | 9 |
| 234 | 352.8364 | 0.0050 | 0.0242 | 9 |
| 235 | 353.0829 | 0.0044 | 0.0310 | 7 |
| 236 | 353.3373 | 0.0045 | 0.0457 | 10 |
| 237 | 353.5734 | 0.0069 | 0.0421 | 9 |
| 238 | 353.7975 | 0.0084 | 0.0265 | 9 |
| 239 | 354.0620 | 0.0094 | 0.0513 | 10 |
| 240 | 354.2977 | 0.0063 | 0.0473 | 10 |
| 241 | 354.5036 | 0.0097 | 0.0135 | 9 |
| 242 | 354.7745 | 0.0052 | 0.0447 | 8 |
| 243 | 354.9992 | 0.0086 | 0.0297 | 10 |
| 244 | 355.2553 | 0.0066 | 0.0461 | 9 |
| 245 | 355.5003 | 0.0040 | 0.0514 | 9 |
| 246 | 355.7534 | 0.0059 | 0.0648 | 9 |
| 247 | 355.9752 | 0.0138 | 0.0469 | 10 |
| 248 | 356.2074 | 0.0173 | 0.0394 | 9 |
| 249 | 356.4554 | 0.0171 | 0.0477 | 9 |
| 250 | 356.6771 | 0.0094 | 0.0297 | 10 |
| 251 | 356.9242 | 0.0087 | 0.0371 | 10 |
| 253 | 357.3896 | 0.0027 | 0.0231 | 9 |
| 254 | 357.6461 | 0.0046 | 0.0399 | 10 |
| 255 | 357.8891 | 0.0097 | 0.0432 | 10 |
| 256 | 358.1178 | 0.0104 | 0.0322 | 9 |
| 257 | 358.3734 | 0.0095 | 0.0481 | 9 |
| 258 | 358.6114 | 0.0072 | 0.0464 | 10 |
| 259 | 358.8609 | 0.0069 | 0.0562 | 9 |
| 260 | 359.0861 | 0.0090 | 0.0417 | 9 |
| 261 | 359.3255 | 0.0030 | 0.0414 | 9 |
| 262 | 359.5627 | 0.0056 | 0.0389 | 10 |
| 264 | 360.0593 | 0.0097 | 0.0561 | 9 |
| 265 | 360.2899 | 0.0040 | 0.0470 | 10 |
| 266 | 360.5186 | 0.0074 | 0.0360 | 10 |
| 267 | 360.7501 | 0.0094 | 0.0278 | 8 |
| 268 | 360.9915 | 0.0059 | 0.0295 | 9 |
| 269 | 361.2480 | 0.0080 | 0.0463 | 10 |
| 270 | 361.4933 | 0.0066 | 0.0519 | 9 |
| 271 | 361.7377 | 0.0064 | 0.0566 | 9 |
| 272 | 361.9752 | 0.0052 | 0.0544 | 9 |
| 273 | 362.1993 | 0.0044 | 0.0388 | 10 |

**Table E1.** Times of negative-superhump maxima in KIC 9406652 during time interval 1 (BJD 2455296–2455553) (continued).

| $E^*$ | Max$^\dagger$ | Error | $O-C^\ddagger$ | $N^\S$ |
|---|---|---|---|---|
| 274 | 362.4316 | 0.0089 | 0.0314 | 9 |
| 275 | 362.6825 | 0.0050 | 0.0426 | 9 |
| 276 | 362.9273 | 0.0074 | 0.0477 | 10 |
| 277 | 363.1669 | 0.0066 | 0.0476 | 10 |
| 278 | 363.4038 | 0.0035 | 0.0448 | 9 |
| 279 | 363.6514 | 0.0178 | 0.0527 | 9 |
| 280 | 363.8752 | 0.0066 | 0.0368 | 10 |
| 281 | 364.1190 | 0.0061 | 0.0409 | 10 |
| 282 | 364.3721 | 0.0068 | 0.0543 | 9 |
| 283 | 364.6191 | 0.0051 | 0.0616 | 9 |
| 284 | 364.8393 | 0.0033 | 0.0421 | 10 |
| 285 | 365.0814 | 0.0073 | 0.0445 | 9 |
| 286 | 365.3278 | 0.0052 | 0.0512 | 8 |
| 287 | 365.5662 | 0.0032 | 0.0499 | 10 |
| 288 | 365.8170 | 0.0068 | 0.0610 | 10 |
| 289 | 366.0633 | 0.0100 | 0.0676 | 8 |
| 290 | 366.2900 | 0.0046 | 0.0546 | 9 |
| 292 | 366.7455 | 0.0054 | 0.0307 | 9 |
| 293 | 367.0005 | 0.0149 | 0.0460 | 9 |
| 294 | 367.2504 | 0.0038 | 0.0562 | 9 |
| 295 | 367.4765 | 0.0040 | 0.0426 | 10 |
| 296 | 367.7232 | 0.0056 | 0.0496 | 9 |
| 297 | 367.9685 | 0.0049 | 0.0552 | 9 |
| 299 | 368.4349 | 0.0055 | 0.0422 | 10 |
| 300 | 368.6823 | 0.0049 | 0.0499 | 9 |
| 301 | 368.9139 | 0.0084 | 0.0418 | 9 |
| 302 | 369.1618 | 0.0067 | 0.0500 | 10 |
| 303 | 369.4035 | 0.0045 | 0.0520 | 10 |
| 304 | 369.6053 | 0.0093 | 0.0141 | 8 |
| 306 | 370.1211 | 0.0038 | 0.0505 | 10 |
| 307 | 370.3706 | 0.0055 | 0.0603 | 9 |
| 308 | 370.6137 | 0.0031 | 0.0637 | 9 |
| 309 | 370.8667 | 0.0045 | 0.0770 | 9 |
| 310 | 371.0647 | 0.0072 | 0.0353 | 10 |
| 316 | 372.5358 | 0.0101 | 0.0682 | 5 |
| 317 | 372.7548 | 0.0129 | 0.0475 | 10 |
| 319 | 373.2411 | 0.0060 | 0.0544 | 9 |
| 320 | 373.4851 | 0.0040 | 0.0587 | 9 |
| 321 | 373.6972 | 0.0057 | 0.0311 | 10 |
| 322 | 373.9324 | 0.0103 | 0.0266 | 9 |
| 323 | 374.2071 | 0.0057 | 0.0616 | 8 |
| 324 | 374.4247 | 0.0082 | 0.0395 | 9 |
| 325 | 374.6507 | 0.0068 | 0.0258 | 10 |
| 326 | 374.8993 | 0.0076 | 0.0347 | 9 |
| 327 | 375.1426 | 0.0044 | 0.0383 | 9 |
| 328 | 375.3842 | 0.0062 | 0.0402 | 10 |
| 329 | 375.6245 | 0.0040 | 0.0408 | 10 |
| 330 | 375.8661 | 0.0022 | 0.0427 | 9 |
| 331 | 376.1071 | 0.0058 | 0.0440 | 9 |
| 332 | 376.3332 | 0.0023 | 0.0304 | 10 |
| 333 | 376.5751 | 0.0032 | 0.0326 | 9 |
| 334 | 376.8317 | 0.0063 | 0.0495 | 9 |
| 335 | 377.0487 | 0.0060 | 0.0268 | 8 |
| 336 | 377.2982 | 0.0026 | 0.0366 | 10 |
| 337 | 377.5536 | 0.0072 | 0.0523 | 9 |
| 338 | 377.7694 | 0.0032 | 0.0284 | 9 |
| 339 | 378.0193 | 0.0017 | 0.0386 | 10 |
| 340 | 378.2638 | 0.0083 | 0.0434 | 10 |
| 341 | 378.4998 | 0.0061 | 0.0397 | 9 |
| 342 | 378.7359 | 0.0038 | 0.0361 | 9 |
| 343 | 378.9785 | 0.0057 | 0.0390 | 10 |
| 344 | 379.2011 | 0.0018 | 0.0219 | 10 |
| 345 | 379.4593 | 0.0057 | 0.0404 | 9 |
| 346 | 379.6913 | 0.0031 | 0.0327 | 9 |
| 347 | 379.9335 | 0.0047 | 0.0352 | 10 |
| 348 | 380.1781 | 0.0041 | 0.0401 | 7 |
| 349 | 380.4157 | 0.0064 | 0.0380 | 9 |
| 350 | 380.6450 | 0.0054 | 0.0276 | 9 |
| 351 | 380.8978 | 0.0048 | 0.0407 | 10 |
| 352 | 381.1402 | 0.0059 | 0.0434 | 9 |
| 353 | 381.3645 | 0.0065 | 0.0280 | 9 |
| 354 | 381.6066 | 0.0069 | 0.0304 | 10 |
| 355 | 381.8454 | 0.0041 | 0.0295 | 10 |
| 356 | 382.0726 | 0.0062 | 0.0170 | 9 |
| 357 | 382.3240 | 0.0052 | 0.0287 | 9 |
| 358 | 382.5563 | 0.0103 | 0.0213 | 10 |
| 359 | 382.8081 | 0.0056 | 0.0334 | 9 |
| 360 | 383.0283 | 0.0029 | 0.0139 | 8 |
| 361 | 383.2734 | 0.0063 | 0.0193 | 9 |
| 362 | 383.5099 | 0.0049 | 0.0161 | 10 |
| 363 | 383.7670 | 0.0107 | 0.0335 | 9 |
| 364 | 383.9944 | 0.0028 | 0.0212 | 9 |
| 365 | 384.2434 | 0.0073 | 0.0305 | 10 |
| 366 | 384.4689 | 0.0071 | 0.0163 | 10 |
| 367 | 384.7169 | 0.0108 | 0.0246 | 9 |
| 368 | 384.9705 | 0.0074 | 0.0385 | 9 |
| 369 | 385.1771 | 0.0077 | 0.0054 | 10 |
| 370 | 385.4078 | 0.0034 | -0.0036 | 10 |
| 371 | 385.6632 | 0.0043 | 0.0121 | 9 |
| 372 | 385.9013 | 0.0028 | 0.0105 | 9 |
| 373 | 386.1362 | 0.0045 | 0.0057 | 9 |
| 374 | 386.3794 | 0.0022 | 0.0092 | 9 |
| 375 | 386.6188 | 0.0042 | 0.0089 | 9 |
| 376 | 386.8661 | 0.0069 | 0.0165 | 9 |
| 377 | 387.0918 | 0.0057 | 0.0025 | 10 |
| 378 | 387.3589 | 0.0073 | 0.0299 | 9 |
| 379 | 387.5785 | 0.0024 | 0.0098 | 9 |
| 380 | 387.8295 | 0.0039 | 0.0211 | 10 |
| 381 | 388.0651 | 0.0053 | 0.0170 | 10 |
| 382 | 388.2978 | 0.0051 | 0.0100 | 9 |
| 383 | 388.5298 | 0.0035 | 0.0023 | 9 |
| 384 | 388.7693 | 0.0027 | 0.0021 | 10 |
| 385 | 389.0133 | 0.0163 | 0.0064 | 8 |
| 386 | 389.2526 | 0.0056 | 0.0060 | 9 |

**Table E1.** Times of negative-superhump maxima in KIC 9406652 during time interval 1 (BJD 2455296–2455553) (continued).

| $E^*$ | Max$^\dagger$ | Error | $O-C^\ddagger$ | $N^\S$ |
|---|---|---|---|---|
| 387 | 389.4899 | 0.0087 | 0.0036 | 9 |
| 388 | 389.7237 | 0.0068 | -0.0023 | 10 |
| 389 | 389.9753 | 0.0071 | 0.0096 | 9 |
| 390 | 390.2047 | 0.0044 | -0.0007 | 9 |
| 391 | 390.4396 | 0.0034 | -0.0055 | 10 |
| 393 | 390.9292 | 0.0042 | 0.0047 | 9 |
| 394 | 391.1631 | 0.0029 | -0.0011 | 9 |
| 395 | 391.4177 | 0.0049 | 0.0138 | 10 |
| 396 | 391.6402 | 0.0028 | -0.0034 | 9 |
| 397 | 391.8869 | 0.0033 | 0.0036 | 9 |
| 398 | 392.1178 | 0.0059 | -0.0052 | 9 |
| 399 | 392.3654 | 0.0063 | 0.0027 | 10 |
| 400 | 392.6029 | 0.0046 | 0.0005 | 9 |
| 401 | 392.8371 | 0.0068 | -0.0050 | 9 |
| 402 | 393.0936 | 0.0104 | 0.0118 | 10 |
| 403 | 393.3057 | 0.0048 | -0.0158 | 10 |
| 404 | 393.5394 | 0.0024 | -0.0218 | 9 |
| 405 | 393.7870 | 0.0047 | -0.0139 | 9 |
| 406 | 394.0030 | 0.0052 | -0.0376 | 10 |
| 407 | 394.2658 | 0.0090 | -0.0145 | 10 |
| 408 | 394.4977 | 0.0042 | -0.0223 | 9 |
| 409 | 394.7375 | 0.0037 | -0.0222 | 9 |
| 410 | 394.9609 | 0.0054 | -0.0385 | 9 |
| 411 | 395.2299 | 0.0036 | -0.0092 | 9 |
| 412 | 395.4643 | 0.0020 | -0.0145 | 9 |
| 413 | 395.7162 | 0.0044 | -0.0023 | 9 |
| 414 | 395.9242 | 0.0096 | -0.0340 | 10 |
| 415 | 396.1896 | 0.0052 | -0.0083 | 9 |
| 416 | 396.4324 | 0.0128 | -0.0052 | 9 |
| 417 | 396.6604 | 0.0074 | -0.0169 | 10 |
| 418 | 396.8757 | 0.0160 | -0.0413 | 10 |
| 419 | 397.1241 | 0.0060 | -0.0326 | 9 |
| 420 | 397.3378 | 0.0179 | -0.0586 | 9 |
| 421 | 397.5880 | 0.0041 | -0.0481 | 10 |
| 422 | 397.8546 | 0.0111 | -0.0212 | 9 |
| 423 | 398.0725 | 0.0133 | -0.0430 | 9 |
| 424 | 398.3122 | 0.0171 | -0.0430 | 9 |
| 425 | 398.5510 | 0.0067 | -0.0439 | 10 |
| 426 | 398.7882 | 0.0105 | -0.0464 | 9 |
| 427 | 399.0215 | 0.0091 | -0.0528 | 9 |
| 433 | 400.4908 | 0.0082 | -0.0217 | 10 |
| 434 | 400.7099 | 0.0075 | -0.0423 | 9 |
| 436 | 401.1798 | 0.0073 | -0.0518 | 10 |
| 438 | 401.6562 | 0.0074 | -0.0548 | 9 |
| 439 | 401.8932 | 0.0117 | -0.0575 | 9 |
| 441 | 402.3850 | 0.0111 | -0.0451 | 8 |
| 442 | 402.6139 | 0.0099 | -0.0559 | 9 |
| 443 | 402.8662 | 0.0081 | -0.0433 | 10 |
| 444 | 403.1113 | 0.0062 | -0.0379 | 10 |
| 445 | 403.3769 | 0.0061 | -0.0120 | 9 |
| 446 | 403.5967 | 0.0104 | -0.0319 | 9 |
| 447 | 403.8433 | 0.0084 | -0.0250 | 10 |

**Table E1.** Times of negative-superhump maxima in KIC 9406652 during time interval 1 (BJD 2455296–2455553) (continued).

| $E^*$ | Max$^\dagger$ | Error | $O-C^\ddagger$ | $N^\S$ |
|---|---|---|---|---|
| 449 | 404.2965 | 0.0199 | -0.0512 | 9 |
| 454 | 405.5142 | 0.0035 | -0.0320 | 9 |
| 457 | 406.2150 | 0.0117 | -0.0503 | 9 |
| 458 | 406.4614 | 0.0170 | -0.0436 | 10 |
| 459 | 406.6840 | 0.0186 | -0.0607 | 10 |
| 461 | 407.1812 | 0.0125 | -0.0429 | 9 |
| 462 | 407.4192 | 0.0146 | -0.0446 | 10 |
| 463 | 407.6864 | 0.0095 | -0.0171 | 9 |
| 464 | 407.9025 | 0.0087 | -0.0407 | 9 |
| 466 | 408.3991 | 0.0114 | -0.0235 | 9 |
| 468 | 408.8719 | 0.0157 | -0.0301 | 9 |
| 469 | 409.1028 | 0.0199 | -0.0389 | 10 |
| 472 | 409.8113 | 0.0089 | -0.0495 | 9 |
| 473 | 410.0565 | 0.0057 | -0.0440 | 10 |
| 475 | 410.5342 | 0.0074 | -0.0457 | 9 |
| 476 | 410.7960 | 0.0079 | -0.0236 | 9 |
| 477 | 411.0181 | 0.0028 | -0.0412 | 10 |
| 478 | 411.2553 | 0.0115 | -0.0437 | 9 |
| 479 | 411.5050 | 0.0039 | -0.0337 | 9 |
| 480 | 411.7687 | 0.0121 | -0.0097 | 10 |
| 482 | 412.2522 | 0.0114 | -0.0056 | 9 |
| 484 | 412.6960 | 0.0175 | -0.0412 | 10 |
| 486 | 413.1824 | 0.0164 | -0.0342 | 9 |
| 488 | 413.6621 | 0.0118 | -0.0339 | 10 |
| 490 | 414.1485 | 0.0017 | -0.0269 | 9 |
| 492 | 414.6347 | 0.0085 | -0.0201 | 10 |
| 493 | 414.8885 | 0.0086 | -0.0060 | 9 |
| 494 | 415.1052 | 0.0109 | -0.0290 | 9 |
| 495 | 415.3425 | 0.0068 | -0.0314 | 10 |
| 496 | 415.6095 | 0.0113 | -0.0041 | 10 |
| 497 | 415.8591 | 0.0103 | 0.0057 | 9 |
| 498 | 416.0870 | 0.0042 | -0.0060 | 9 |
| 500 | 416.5855 | 0.0043 | 0.0131 | 9 |
| 501 | 416.7810 | 0.0125 | -0.0311 | 9 |
| 505 | 417.7425 | 0.0138 | -0.0284 | 9 |
| 506 | 417.9513 | 0.0060 | -0.0593 | 5 |
| 507 | 418.2348 | 0.0150 | -0.0155 | 10 |
| 508 | 418.4535 | 0.0125 | -0.0365 | 9 |
| 510 | 418.9663 | 0.0088 | -0.0031 | 10 |
| 511 | 419.2004 | 0.0071 | -0.0087 | 10 |
| 512 | 419.4223 | 0.0096 | -0.0265 | 9 |
| 514 | 419.9406 | 0.0052 | 0.0124 | 10 |
| 515 | 420.1670 | 0.0139 | -0.0009 | 9 |
| 516 | 420.3962 | 0.0089 | -0.0114 | 8 |
| 517 | 420.6548 | 0.0079 | 0.0075 | 9 |
| 518 | 420.9052 | 0.0097 | 0.0182 | 10 |
| 519 | 421.1373 | 0.0182 | 0.0106 | 9 |
| 520 | 421.3865 | 0.0173 | 0.0201 | 7 |
| 521 | 421.5606 | 0.0054 | -0.0455 | 10 |
| 522 | 421.8090 | 0.0089 | -0.0368 | 10 |
| 523 | 422.0465 | 0.0066 | -0.0390 | 9 |
| 524 | 422.2718 | 0.0102 | -0.0534 | 9 |

**Table E1.** Times of negative-superhump maxima in KIC 9406652 during time interval 1 (BJD 2455296–2455553) (continued).

| $E^*$ | Max$^\dagger$ | Error | $O-C^\ddagger$ | $N^\S$ |
|---|---|---|---|---|
| 525 | 422.5519 | 0.0045 | -0.0130 | 10 |
| 526 | 422.7967 | 0.0034 | -0.0079 | 9 |
| 527 | 423.0308 | 0.0062 | -0.0135 | 9 |
| 528 | 423.2742 | 0.0058 | -0.0098 | 8 |
| 529 | 423.5130 | 0.0038 | -0.0107 | 10 |
| 530 | 423.7626 | 0.0029 | -0.0008 | 9 |
| 531 | 423.9973 | 0.0063 | -0.0058 | 9 |
| 532 | 424.2581 | 0.0039 | 0.0152 | 10 |
| 533 | 424.4765 | 0.0068 | -0.0060 | 9 |
| 534 | 424.7206 | 0.0092 | -0.0016 | 9 |
| 535 | 424.9650 | 0.0055 | 0.0031 | 9 |
| 536 | 425.1966 | 0.0149 | -0.0050 | 10 |
| 537 | 425.4224 | 0.0095 | -0.0189 | 10 |
| 538 | 425.6597 | 0.0095 | -0.0213 | 9 |
| 539 | 425.8831 | 0.0145 | -0.0376 | 9 |
| 540 | 426.1257 | 0.0059 | -0.0347 | 10 |
| 541 | 426.3840 | 0.0041 | -0.0161 | 8 |
| 542 | 426.6119 | 0.0058 | -0.0279 | 9 |
| 543 | 426.8600 | 0.0118 | -0.0195 | 9 |
| 544 | 427.0820 | 0.0080 | -0.0372 | 10 |
| 545 | 427.3403 | 0.0051 | -0.0186 | 9 |
| 546 | 427.5893 | 0.0041 | -0.0093 | 9 |
| 547 | 427.8190 | 0.0051 | -0.0193 | 10 |
| 548 | 428.0638 | 0.0043 | -0.0142 | 10 |
| 549 | 428.2950 | 0.0112 | -0.0227 | 9 |
| 550 | 428.5550 | 0.0041 | -0.0024 | 9 |
| 551 | 428.7979 | 0.0027 | 0.0008 | 10 |
| 552 | 429.0029 | 0.0169 | -0.0339 | 9 |
| 553 | 429.2777 | 0.0050 | 0.0012 | 8 |
| 554 | 429.5054 | 0.0106 | -0.0108 | 9 |
| 555 | 429.7407 | 0.0052 | -0.0152 | 10 |
| 556 | 429.9555 | 0.0062 | -0.0401 | 9 |
| 557 | 430.2136 | 0.0028 | -0.0217 | 9 |
| 560 | 430.9238 | 0.0149 | -0.0306 | 8 |
| 561 | 431.1853 | 0.0167 | -0.0088 | 8 |
| 566 | 432.3721 | 0.0163 | -0.0205 | 10 |
| 567 | 432.6345 | 0.0069 | 0.0022 | 9 |
| 570 | 433.3185 | 0.0111 | -0.0329 | 10 |
| 573 | 434.0217 | 0.0074 | -0.0488 | 10 |
| 574 | 434.2812 | 0.0098 | -0.0290 | 9 |
| 577 | 435.0212 | 0.0141 | -0.0081 | 10 |
| 578 | 435.2371 | 0.0200 | -0.0319 | 9 |
| 579 | 435.4808 | 0.0069 | -0.0279 | 9 |
| 580 | 435.7428 | 0.0032 | -0.0056 | 9 |
| 582 | 436.2090 | 0.0142 | -0.0188 | 9 |
| 584 | 436.7602 | 0.0177 | 0.0530 | 10 |
| 585 | 436.9649 | 0.0136 | 0.0180 | 10 |
| 590 | 438.0829 | 0.0132 | -0.0625 | 9 |
| 592 | 438.5688 | 0.0047 | -0.0560 | 10 |
| 593 | 438.8373 | 0.0174 | -0.0272 | 9 |
| 595 | 439.3181 | 0.0062 | -0.0258 | 9 |
| 596 | 439.5660 | 0.0069 | -0.0176 | 10 |

**Table E1.** Times of negative-superhump maxima in KIC 9406652 during time interval 1 (BJD 2455296–2455553) (continued).

| $E^*$ | Max$^\dagger$ | Error | $O-C^\ddagger$ | $N^\S$ |
|---|---|---|---|---|
| 597 | 439.8192 | 0.0054 | -0.0041 | 9 |
| 598 | 440.0432 | 0.0112 | -0.0198 | 9 |
| 599 | 440.2842 | 0.0063 | -0.0185 | 9 |
| 601 | 440.7635 | 0.0090 | -0.0186 | 9 |
| 602 | 441.0257 | 0.0118 | 0.0039 | 9 |
| 604 | 441.5008 | 0.0108 | -0.0004 | 9 |
| 606 | 441.9550 | 0.0063 | -0.0256 | 8 |
| 607 | 442.1937 | 0.0067 | -0.0266 | 10 |
| 608 | 442.4336 | 0.0099 | -0.0264 | 9 |
| 609 | 442.6532 | 0.0065 | -0.0465 | 9 |
| 610 | 442.8971 | 0.0068 | -0.0423 | 10 |
| 611 | 443.1524 | 0.0065 | -0.0267 | 9 |
| 612 | 443.3849 | 0.0061 | -0.0339 | 9 |
| 613 | 443.6285 | 0.0067 | -0.0300 | 9 |
| 614 | 443.8690 | 0.0064 | -0.0292 | 10 |
| 615 | 444.1078 | 0.0071 | -0.0301 | 10 |
| 616 | 444.3589 | 0.0056 | -0.0187 | 9 |
| 617 | 444.6132 | 0.0090 | -0.0041 | 9 |
| 618 | 444.8098 | 0.0121 | -0.0472 | 10 |
| 619 | 445.0929 | 0.0132 | -0.0038 | 9 |
| 622 | 445.7965 | 0.0149 | -0.0193 | 10 |
| 624 | 446.2333 | 0.0110 | -0.0619 | 9 |
| 628 | 447.2257 | 0.0152 | -0.0283 | 9 |
| 629 | 447.4846 | 0.0064 | -0.0091 | 10 |
| 631 | 447.9251 | 0.0063 | -0.0480 | 9 |
| 632 | 448.1855 | 0.0140 | -0.0273 | 9 |
| 633 | 448.3953 | 0.0037 | -0.0572 | 10 |
| 634 | 448.6650 | 0.0106 | -0.0272 | 9 |
| 635 | 448.9217 | 0.0082 | -0.0102 | 9 |
| 636 | 449.1601 | 0.0075 | -0.0115 | 9 |
| 637 | 449.4009 | 0.0072 | -0.0104 | 10 |
| 639 | 449.9072 | 0.0125 | 0.0165 | 9 |
| 640 | 450.0763 | 0.0085 | -0.0541 | 10 |
| 642 | 450.6116 | 0.0100 | 0.0018 | 9 |
| 643 | 450.8352 | 0.0053 | -0.0143 | 9 |
| 646 | 451.5569 | 0.0050 | -0.0117 | 9 |
| 647 | 451.7790 | 0.0091 | -0.0293 | 9 |
| 648 | 451.9939 | 0.0147 | -0.0541 | 9 |
| 649 | 452.2839 | 0.0044 | -0.0038 | 9 |
| 650 | 452.5152 | 0.0031 | -0.0122 | 9 |
| 652 | 453.0312 | 0.0126 | 0.0244 | 10 |
| 653 | 453.2483 | 0.0013 | 0.0018 | 9 |
| 654 | 453.4705 | 0.0070 | -0.0157 | 9 |
| 655 | 453.7648 | 0.0063 | 0.0389 | 10 |
| 656 | 453.9766 | 0.0054 | 0.0110 | 9 |
| 657 | 454.2066 | 0.0038 | 0.0013 | 9 |
| 658 | 454.4531 | 0.0054 | 0.0081 | 9 |
| 659 | 454.6820 | 0.0043 | -0.0027 | 10 |
| 660 | 454.9378 | 0.0144 | 0.0134 | 8 |
| 661 | 455.1914 | 0.0109 | 0.0273 | 8 |
| 662 | 455.4083 | 0.0072 | 0.0045 | 10 |
| 663 | 455.6634 | 0.0040 | 0.0199 | 10 |

**Table E1.** Times of negative-superhump maxima in KIC 9406652 during time interval 1 (BJD 2455296–2455553) (continued).

| $E^*$ | Max$^\dagger$ | Error | $O-C^\ddagger$ | $N^\S$ |
|---|---|---|---|---|
| 664 | 455.8993 | 0.0196 | 0.0161 | 9 |
| 666 | 456.3700 | 0.0027 | 0.0074 | 10 |
| 667 | 456.5903 | 0.0043 | -0.0120 | 10 |
| 668 | 456.8410 | 0.0061 | -0.0010 | 9 |
| 669 | 457.0819 | 0.0068 | 0.0002 | 9 |
| 670 | 457.3175 | 0.0066 | -0.0039 | 10 |
| 671 | 457.5300 | 0.0092 | -0.0311 | 9 |
| 672 | 457.7848 | 0.0125 | -0.0160 | 9 |
| 673 | 458.0400 | 0.0043 | -0.0005 | 8 |
| 674 | 458.2816 | 0.0068 | 0.0014 | 10 |
| 675 | 458.5131 | 0.0036 | -0.0068 | 9 |
| 676 | 458.7545 | 0.0027 | -0.0051 | 9 |
| 677 | 458.9985 | 0.0070 | -0.0008 | 10 |
| 678 | 459.2419 | 0.0082 | 0.0029 | 10 |
| 679 | 459.4855 | 0.0062 | 0.0068 | 9 |
| 680 | 459.7138 | 0.0042 | -0.0046 | 9 |
| 681 | 459.9339 | 0.0047 | -0.0242 | 10 |
| 682 | 460.2209 | 0.0062 | 0.0231 | 9 |
| 683 | 460.4375 | 0.0071 | 0.0000 | 9 |
| 684 | 460.6559 | 0.0047 | -0.0213 | 9 |
| 685 | 460.9041 | 0.0079 | -0.0128 | 10 |
| 686 | 461.1350 | 0.0099 | -0.0216 | 8 |
| 687 | 461.3583 | 0.0089 | -0.0380 | 9 |
| 688 | 461.6328 | 0.0044 | -0.0032 | 10 |
| 689 | 461.8504 | 0.0040 | -0.0253 | 10 |
| 690 | 462.0962 | 0.0063 | -0.0192 | 9 |
| 695 | 463.3148 | 0.0025 | 0.0009 | 9 |
| 696 | 463.5378 | 0.0054 | -0.0158 | 10 |
| 697 | 463.7980 | 0.0056 | 0.0047 | 9 |
| 698 | 464.0270 | 0.0032 | -0.0060 | 9 |
| 699 | 464.2666 | 0.0031 | -0.0061 | 9 |
| 700 | 464.5048 | 0.0037 | -0.0076 | 10 |
| 701 | 464.7436 | 0.0032 | -0.0085 | 9 |
| 702 | 464.9942 | 0.0039 | 0.0024 | 9 |
| 703 | 465.2364 | 0.0033 | 0.0049 | 9 |
| 704 | 465.4621 | 0.0039 | -0.0091 | 10 |
| 705 | 465.7065 | 0.0029 | -0.0044 | 9 |
| 706 | 465.9381 | 0.0054 | -0.0125 | 9 |
| 707 | 466.1775 | 0.0063 | -0.0128 | 10 |
| 708 | 466.4049 | 0.0074 | -0.0251 | 9 |
| 709 | 466.6338 | 0.0075 | -0.0359 | 9 |
| 710 | 466.8943 | 0.0061 | -0.0151 | 9 |
| 711 | 467.1217 | 0.0052 | -0.0274 | 10 |
| 712 | 467.3661 | 0.0041 | -0.0227 | 9 |
| 713 | 467.6075 | 0.0068 | -0.0210 | 9 |
| 714 | 467.8494 | 0.0028 | -0.0188 | 10 |
| 715 | 468.0923 | 0.0038 | -0.0156 | 10 |
| 716 | 468.3271 | 0.0041 | -0.0205 | 9 |
| 717 | 468.5565 | 0.0034 | -0.0308 | 9 |
| 718 | 468.7978 | 0.0043 | -0.0292 | 10 |
| 719 | 469.0423 | 0.0044 | -0.0244 | 10 |
| 720 | 469.2964 | 0.0050 | -0.0100 | 9 |

**Table E1.** Times of negative-superhump maxima in KIC 9406652 during time interval 1 (BJD 2455296–2455553) (continued).

| $E^*$ | Max$^\dagger$ | Error | $O-C^\ddagger$ | $N^\S$ |
|---|---|---|---|---|
| 721 | 469.5145 | 0.0054 | -0.0316 | 9 |
| 722 | 469.7541 | 0.0033 | -0.0317 | 10 |
| 723 | 470.0078 | 0.0039 | -0.0177 | 9 |
| 724 | 470.2360 | 0.0037 | -0.0292 | 9 |
| 725 | 470.4844 | 0.0037 | -0.0205 | 9 |
| 726 | 470.7224 | 0.0062 | -0.0222 | 10 |
| 727 | 470.9601 | 0.0050 | -0.0242 | 9 |
| 728 | 471.1942 | 0.0045 | -0.0298 | 8 |
| 729 | 471.4331 | 0.0040 | -0.0306 | 10 |
| 730 | 471.6748 | 0.0036 | -0.0286 | 10 |
| 731 | 471.9046 | 0.0040 | -0.0385 | 9 |
| 732 | 472.1568 | 0.0026 | -0.0260 | 9 |
| 733 | 472.4017 | 0.0037 | -0.0208 | 10 |
| 734 | 472.6311 | 0.0045 | -0.0311 | 9 |
| 736 | 473.0793 | 0.0067 | -0.0623 | 9 |
| 737 | 473.3407 | 0.0104 | -0.0406 | 10 |
| 738 | 473.5670 | 0.0058 | -0.0540 | 9 |
| 739 | 473.8193 | 0.0067 | -0.0414 | 9 |
| 740 | 474.0656 | 0.0042 | -0.0348 | 9 |
| 741 | 474.3005 | 0.0059 | -0.0396 | 10 |
| 742 | 474.5473 | 0.0058 | -0.0325 | 9 |
| 743 | 474.7999 | 0.0027 | -0.0196 | 9 |
| 744 | 475.0382 | 0.0055 | -0.0210 | 10 |
| 745 | 475.2844 | 0.0057 | -0.0145 | 10 |
| 746 | 475.5312 | 0.0054 | -0.0074 | 9 |
| 747 | 475.7617 | 0.0091 | -0.0166 | 9 |
| 748 | 475.9938 | 0.0062 | -0.0242 | 10 |
| 749 | 476.2218 | 0.0096 | -0.0359 | 9 |
| 750 | 476.4713 | 0.0072 | -0.0261 | 9 |
| 751 | 476.7197 | 0.0101 | -0.0174 | 9 |
| 755 | 477.6517 | 0.0039 | -0.0442 | 10 |
| 756 | 477.8834 | 0.0044 | -0.0522 | 10 |
| 757 | 478.1308 | 0.0032 | -0.0445 | 9 |
| 758 | 478.3855 | 0.0058 | -0.0295 | 9 |
| 759 | 478.6292 | 0.0054 | -0.0255 | 10 |
| 760 | 478.8725 | 0.0051 | -0.0219 | 9 |
| 761 | 479.1215 | 0.0024 | -0.0126 | 9 |
| 762 | 479.3513 | 0.0021 | -0.0225 | 9 |
| 763 | 479.5937 | 0.0045 | -0.0198 | 10 |
| 764 | 479.8353 | 0.0037 | -0.0179 | 9 |
| 765 | 480.0755 | 0.0043 | -0.0174 | 8 |
| 766 | 480.3178 | 0.0057 | -0.0148 | 9 |
| 767 | 480.5464 | 0.0064 | -0.0259 | 10 |
| 768 | 480.7986 | 0.0062 | -0.0134 | 9 |
| 769 | 481.0153 | 0.0069 | -0.0364 | 9 |
| 771 | 481.4904 | 0.0052 | -0.0407 | 9 |
| 772 | 481.7309 | 0.0049 | -0.0399 | 8 |
| 773 | 481.9625 | 0.0042 | -0.0480 | 9 |
| 774 | 482.2186 | 0.0024 | -0.0316 | 10 |
| 775 | 482.4524 | 0.0070 | -0.0375 | 9 |
| 776 | 482.6781 | 0.0088 | -0.0515 | 9 |
| 777 | 482.9317 | 0.0094 | -0.0376 | 9 |

**Table E1.** Times of negative-superhump maxima in KIC 9406652 during time interval 1 (BJD 2455296–2455553) (continued).

| $E^*$ | Max[†] | Error | $O-C$[‡] | $N$[§] |
|---|---|---|---|---|
| 778 | 483.1847 | 0.0059 | -0.0243 | 9 |
| 779 | 483.3985 | 0.0075 | -0.0502 | 9 |
| 780 | 483.6569 | 0.0047 | -0.0315 | 9 |
| 781 | 483.9014 | 0.0043 | -0.0267 | 10 |
| 782 | 484.1247 | 0.0056 | -0.0431 | 10 |
| 783 | 484.3702 | 0.0049 | -0.0373 | 9 |
| 784 | 484.6114 | 0.0048 | -0.0358 | 9 |
| 785 | 484.8565 | 0.0048 | -0.0304 | 10 |
| 786 | 485.0957 | 0.0059 | -0.0309 | 10 |
| 787 | 485.3568 | 0.0052 | -0.0095 | 9 |
| 788 | 485.5775 | 0.0077 | -0.0285 | 9 |
| 789 | 485.8452 | 0.0053 | -0.0005 | 10 |
| 790 | 486.0896 | 0.0072 | 0.0042 | 8 |
| 791 | 486.3245 | 0.0030 | -0.0006 | 9 |
| 793 | 486.7834 | 0.0122 | -0.0211 | 10 |
| 795 | 487.2632 | 0.0089 | -0.0207 | 9 |
| 796 | 487.5058 | 0.0038 | -0.0178 | 10 |
| 797 | 487.7303 | 0.0039 | -0.0330 | 10 |
| 798 | 487.9774 | 0.0048 | -0.0256 | 8 |
| 799 | 488.2198 | 0.0029 | -0.0229 | 9 |
| 800 | 488.4634 | 0.0063 | -0.0190 | 10 |
| 801 | 488.7028 | 0.0039 | -0.0193 | 9 |
| 802 | 488.9546 | 0.0038 | -0.0072 | 9 |
| 803 | 489.1981 | 0.0039 | -0.0034 | 9 |
| 804 | 489.4434 | 0.0042 | 0.0022 | 10 |
| 805 | 489.6782 | 0.0116 | -0.0027 | 9 |
| 806 | 489.9297 | 0.0041 | 0.0091 | 9 |
| 807 | 490.1721 | 0.0046 | 0.0118 | 10 |
| 808 | 490.4050 | 0.0022 | 0.0050 | 10 |
| 809 | 490.6262 | 0.0088 | -0.0135 | 9 |
| 810 | 490.8938 | 0.0041 | 0.0144 | 9 |
| 811 | 491.1186 | 0.0047 | -0.0005 | 10 |
| 812 | 491.3477 | 0.0071 | -0.0111 | 10 |
| 813 | 491.5888 | 0.0048 | -0.0097 | 9 |
| 814 | 491.8330 | 0.0069 | -0.0052 | 9 |
| 815 | 492.0704 | 0.0034 | -0.0075 | 9 |
| 816 | 492.3058 | 0.0041 | -0.0118 | 9 |
| 817 | 492.5872 | 0.0170 | 0.0299 | 9 |
| 818 | 492.8037 | 0.0039 | 0.0067 | 9 |
| 819 | 493.0600 | 0.0062 | 0.0233 | 7 |
| 824 | 494.2326 | 0.0047 | -0.0026 | 9 |
| 825 | 494.4773 | 0.0020 | 0.0024 | 9 |
| 826 | 494.7165 | 0.0045 | 0.0019 | 10 |
| 827 | 494.9559 | 0.0059 | 0.0016 | 9 |
| 828 | 495.1942 | 0.0028 | 0.0002 | 9 |
| 829 | 495.4427 | 0.0023 | 0.0090 | 9 |
| 830 | 495.6810 | 0.0036 | 0.0076 | 10 |
| 831 | 495.9173 | 0.0043 | 0.0042 | 9 |
| 832 | 496.1677 | 0.0029 | 0.0149 | 8 |
| 833 | 496.4036 | 0.0063 | 0.0111 | 10 |
| 834 | 496.6450 | 0.0042 | 0.0128 | 10 |
| 835 | 496.8861 | 0.0058 | 0.0142 | 9 |

**Table E1.** Times of negative-superhump maxima in KIC 9406652 during time interval 1 (BJD 2455296–2455553) (continued).

| $E^*$ | Max[†] | Error | $O-C$[‡] | $N$[§] |
|---|---|---|---|---|
| 836 | 497.1171 | 0.0051 | 0.0055 | 9 |
| 837 | 497.3675 | 0.0050 | 0.0162 | 10 |
| 838 | 497.6029 | 0.0030 | 0.0119 | 10 |
| 839 | 497.8444 | 0.0058 | 0.0137 | 9 |
| 840 | 498.0846 | 0.0037 | 0.0142 | 9 |
| 841 | 498.3184 | 0.0021 | 0.0083 | 10 |
| 842 | 498.5628 | 0.0042 | 0.0130 | 9 |
| 843 | 498.8031 | 0.0036 | 0.0136 | 9 |
| 844 | 499.0273 | 0.0067 | -0.0019 | 9 |
| 845 | 499.2818 | 0.0042 | 0.0129 | 9 |
| 846 | 499.5173 | 0.0027 | 0.0087 | 9 |
| 847 | 499.7595 | 0.0021 | 0.0112 | 9 |
| 848 | 500.0018 | 0.0023 | 0.0138 | 10 |
| 849 | 500.2397 | 0.0028 | 0.0120 | 10 |
| 850 | 500.4872 | 0.0050 | 0.0198 | 9 |
| 851 | 500.7264 | 0.0027 | 0.0193 | 9 |
| 852 | 500.9772 | 0.0050 | 0.0304 | 10 |
| 853 | 501.2071 | 0.0037 | 0.0206 | 9 |
| 854 | 501.4571 | 0.0045 | 0.0309 | 9 |
| 855 | 501.6814 | 0.0054 | 0.0155 | 9 |
| 856 | 501.9153 | 0.0054 | 0.0097 | 10 |
| 857 | 502.1474 | 0.0063 | 0.0021 | 8 |
| 858 | 502.3886 | 0.0045 | 0.0036 | 9 |
| 859 | 502.6351 | 0.0030 | 0.0104 | 9 |
| 860 | 502.8722 | 0.0028 | 0.0078 | 10 |
| 861 | 503.1117 | 0.0043 | 0.0076 | 9 |
| 862 | 503.3573 | 0.0013 | 0.0135 | 9 |
| 863 | 503.6052 | 0.0027 | 0.0217 | 10 |
| 864 | 503.8410 | 0.0030 | 0.0178 | 10 |
| 865 | 504.0802 | 0.0010 | 0.0173 | 9 |
| 866 | 504.3309 | 0.0036 | 0.0283 | 9 |
| 867 | 504.5619 | 0.0030 | 0.0196 | 10 |
| 868 | 504.8104 | 0.0044 | 0.0284 | 9 |
| 869 | 505.0464 | 0.0074 | 0.0247 | 9 |
| 870 | 505.2929 | 0.0055 | 0.0315 | 9 |
| 871 | 505.5273 | 0.0048 | 0.0262 | 10 |
| 872 | 505.7628 | 0.0144 | 0.0220 | 9 |
| 873 | 506.0088 | 0.0056 | 0.0283 | 9 |
| 874 | 506.2327 | 0.0054 | 0.0125 | 10 |
| 875 | 506.4666 | 0.0025 | 0.0067 | 10 |
| 876 | 506.7103 | 0.0026 | 0.0107 | 9 |
| 877 | 506.9591 | 0.0071 | 0.0198 | 9 |
| 878 | 507.1993 | 0.0053 | 0.0203 | 10 |
| 879 | 507.4337 | 0.0040 | 0.0150 | 10 |
| 880 | 507.6684 | 0.0016 | 0.0100 | 9 |
| 881 | 507.9025 | 0.0046 | 0.0044 | 9 |
| 882 | 508.1553 | 0.0037 | 0.0175 | 9 |
| 883 | 508.3946 | 0.0035 | 0.0171 | 9 |
| 884 | 508.6384 | 0.0017 | 0.0212 | 9 |
| 885 | 508.8733 | 0.0020 | 0.0164 | 9 |
| 886 | 509.1159 | 0.0039 | 0.0193 | 10 |
| 887 | 509.3639 | 0.0048 | 0.0276 | 9 |

**Table E1.** Times of negative-superhump maxima in KIC 9406652 during time interval 1 (BJD 2455296–2455553) (continued).

| $E^*$ | Max$^\dagger$ | Error | $O-C^\ddagger$ | $N^\S$ |
|---|---|---|---|---|
| 888 | 509.6191 | 0.0045 | 0.0431 | 9 |
| 889 | 509.8255 | 0.0059 | 0.0097 | 10 |
| 890 | 510.0632 | 0.0076 | 0.0078 | 10 |
| 891 | 510.2930 | 0.0064 | -0.0021 | 9 |
| 892 | 510.5546 | 0.0054 | 0.0198 | 9 |
| 893 | 510.7930 | 0.0032 | 0.0185 | 10 |
| 894 | 511.0181 | 0.0052 | 0.0039 | 9 |
| 895 | 511.2634 | 0.0051 | 0.0095 | 9 |
| 896 | 511.5027 | 0.0053 | 0.0091 | 9 |
| 897 | 511.7436 | 0.0020 | 0.0103 | 10 |
| 898 | 511.9895 | 0.0020 | 0.0165 | 9 |
| 899 | 512.2311 | 0.0029 | 0.0184 | 9 |
| 900 | 512.4710 | 0.0029 | 0.0186 | 10 |
| 901 | 512.7048 | 0.0020 | 0.0127 | 10 |
| 902 | 512.9624 | 0.0060 | 0.0306 | 9 |
| 903 | 513.1878 | 0.0036 | 0.0163 | 9 |
| 904 | 513.4437 | 0.0041 | 0.0325 | 10 |
| 905 | 513.6790 | 0.0036 | 0.0281 | 10 |
| 906 | 513.9382 | 0.0042 | 0.0476 | 9 |
| 907 | 514.1511 | 0.0059 | 0.0208 | 8 |
| 908 | 514.3884 | 0.0041 | 0.0184 | 10 |
| 909 | 514.6148 | 0.0073 | 0.0051 | 9 |
| 910 | 514.8644 | 0.0022 | 0.0150 | 9 |
| 911 | 515.1004 | 0.0053 | 0.0113 | 9 |
| 912 | 515.3330 | 0.0038 | 0.0042 | 10 |
| 913 | 515.5796 | 0.0054 | 0.0111 | 9 |
| 914 | 515.8204 | 0.0044 | 0.0122 | 9 |
| 915 | 516.0553 | 0.0028 | 0.0074 | 10 |
| 916 | 516.2952 | 0.0022 | 0.0076 | 10 |
| 917 | 516.5354 | 0.0011 | 0.0081 | 9 |
| 918 | 516.7887 | 0.0028 | 0.0217 | 9 |
| 919 | 517.0229 | 0.0070 | 0.0162 | 9 |
| 920 | 517.2690 | 0.0034 | 0.0226 | 9 |
| 921 | 517.5231 | 0.0064 | 0.0370 | 9 |
| 922 | 517.7556 | 0.0064 | 0.0298 | 9 |
| 923 | 517.9910 | 0.0123 | 0.0255 | 10 |
| 924 | 518.2273 | 0.0109 | 0.0221 | 9 |
| 925 | 518.4467 | 0.0053 | 0.0018 | 9 |
| 926 | 518.7005 | 0.0050 | 0.0159 | 10 |
| 927 | 518.9330 | 0.0071 | 0.0087 | 10 |
| 928 | 519.1645 | 0.0059 | 0.0005 | 9 |
| 929 | 519.3998 | 0.0044 | -0.0039 | 9 |
| 930 | 519.6408 | 0.0032 | -0.0026 | 10 |
| 931 | 519.8854 | 0.0026 | 0.0023 | 10 |
| 932 | 520.1307 | 0.0023 | 0.0079 | 8 |
| 933 | 520.3762 | 0.0029 | 0.0137 | 9 |
| 934 | 520.6208 | 0.0031 | 0.0186 | 10 |
| 935 | 520.8596 | 0.0032 | 0.0177 | 9 |
| 936 | 521.0984 | 0.0042 | 0.0168 | 9 |
| 937 | 521.3400 | 0.0043 | 0.0187 | 9 |
| 938 | 521.5866 | 0.0028 | 0.0256 | 10 |
| 939 | 521.8432 | 0.0089 | 0.0425 | 8 |

**Table E1.** Times of negative-superhump maxima in KIC 9406652 during time interval 1 (BJD 2455296–2455553) (continued).

| $E^*$ | Max$^\dagger$ | Error | $O-C^\ddagger$ | $N^\S$ |
|---|---|---|---|---|
| 940 | 522.0616 | 0.0066 | 0.0211 | 9 |
| 941 | 522.3021 | 0.0072 | 0.0220 | 10 |
| 942 | 522.5378 | 0.0053 | 0.0180 | 10 |
| 943 | 522.7594 | 0.0047 | -0.0001 | 9 |
| 944 | 523.0045 | 0.0057 | 0.0053 | 8 |
| 945 | 523.2811 | 0.0039 | 0.0422 | 5 |
| 949 | 524.2106 | 0.0044 | 0.0129 | 8 |
| 950 | 524.4408 | 0.0020 | 0.0034 | 9 |
| 951 | 524.6883 | 0.0021 | 0.0112 | 9 |
| 952 | 524.9392 | 0.0067 | 0.0224 | 10 |
| 953 | 525.1872 | 0.0032 | 0.0307 | 10 |
| 954 | 525.4339 | 0.0079 | 0.0377 | 9 |
| 955 | 525.6585 | 0.0073 | 0.0226 | 9 |
| 956 | 525.8993 | 0.0114 | 0.0237 | 10 |
| 958 | 526.3773 | 0.0125 | 0.0223 | 9 |
| 959 | 526.6094 | 0.0076 | 0.0147 | 9 |
| 960 | 526.8238 | 0.0099 | -0.0106 | 10 |
| 961 | 527.0455 | 0.0034 | -0.0286 | 9 |
| 962 | 527.3158 | 0.0039 | 0.0020 | 9 |
| 963 | 527.5437 | 0.0054 | -0.0098 | 9 |
| 964 | 527.7909 | 0.0038 | -0.0023 | 10 |
| 965 | 528.0317 | 0.0060 | -0.0012 | 9 |
| 966 | 528.2761 | 0.0035 | 0.0035 | 9 |
| 967 | 528.5190 | 0.0039 | 0.0067 | 10 |
| 968 | 528.7591 | 0.0041 | 0.0071 | 10 |
| 969 | 528.9949 | 0.0039 | 0.0032 | 8 |
| 970 | 529.2493 | 0.0031 | 0.0179 | 9 |
| 971 | 529.4808 | 0.0111 | 0.0097 | 10 |
| 972 | 529.7311 | 0.0068 | 0.0203 | 9 |
| 973 | 529.9604 | 0.0111 | 0.0099 | 9 |
| 974 | 530.1715 | 0.0073 | -0.0187 | 9 |
| 975 | 530.4261 | 0.0028 | -0.0038 | 10 |
| 976 | 530.6608 | 0.0037 | -0.0088 | 9 |
| 977 | 530.9001 | 0.0049 | -0.0092 | 9 |
| 978 | 531.1402 | 0.0029 | -0.0088 | 9 |
| 979 | 531.3794 | 0.0034 | -0.0093 | 10 |
| 980 | 531.6244 | 0.0070 | -0.0040 | 9 |
| 982 | 532.0881 | 0.0031 | -0.0197 | 10 |
| 983 | 532.3284 | 0.0050 | -0.0191 | 10 |
| 984 | 532.5719 | 0.0053 | -0.0153 | 9 |
| 985 | 532.7978 | 0.0076 | -0.0291 | 9 |
| 986 | 533.0492 | 0.0048 | -0.0174 | 10 |
| 987 | 533.2935 | 0.0072 | -0.0128 | 9 |
| 988 | 533.5370 | 0.0027 | -0.0090 | 9 |
| 989 | 533.7642 | 0.0085 | -0.0215 | 9 |
| 990 | 534.0206 | 0.0029 | -0.0048 | 10 |
| 991 | 534.2559 | 0.0028 | -0.0092 | 9 |
| 992 | 534.4872 | 0.0031 | -0.0176 | 9 |
| 993 | 534.7294 | 0.0030 | -0.0151 | 10 |
| 994 | 534.9694 | 0.0058 | -0.0148 | 9 |
| 995 | 535.2081 | 0.0035 | -0.0158 | 8 |
| 996 | 535.4557 | 0.0022 | -0.0079 | 9 |

**Table E1.** Times of negative-superhump maxima in KIC 9406652 during time interval 1 (BJD 2455296–2455553) (continued).

| $E^*$ | Max[†] | Error | $O-C^‡$ | $N^§$ |
|---|---|---|---|---|
| 997 | 535.6887 | 0.0021 | -0.0146 | 10 |
| 998 | 535.9430 | 0.0038 | -0.0000 | 10 |
| 999 | 536.1751 | 0.0040 | -0.0076 | 9 |
| 1000 | 536.4129 | 0.0049 | -0.0095 | 8 |
| 1001 | 536.6476 | 0.0054 | -0.0145 | 10 |
| 1002 | 536.8917 | 0.0065 | -0.0101 | 9 |
| 1003 | 537.1341 | 0.0038 | -0.0073 | 9 |
| 1004 | 537.3621 | 0.0043 | -0.0191 | 9 |
| 1005 | 537.5976 | 0.0039 | -0.0233 | 10 |
| 1006 | 537.8376 | 0.0025 | -0.0230 | 9 |
| 1007 | 538.0831 | 0.0012 | -0.0172 | 9 |
| 1008 | 538.3286 | 0.0020 | -0.0114 | 10 |
| 1009 | 538.5626 | 0.0039 | -0.0171 | 10 |
| 1010 | 538.7994 | 0.0041 | -0.0200 | 9 |
| 1011 | 539.0286 | 0.0033 | -0.0305 | 9 |
| 1012 | 539.2811 | 0.0036 | -0.0177 | 10 |
| 1013 | 539.5240 | 0.0018 | -0.0144 | 9 |
| 1014 | 539.7636 | 0.0031 | -0.0146 | 9 |
| 1015 | 539.9964 | 0.0058 | -0.0215 | 9 |
| 1016 | 540.2381 | 0.0054 | -0.0195 | 10 |
| 1017 | 540.4711 | 0.0074 | -0.0262 | 9 |
| 1018 | 540.7254 | 0.0038 | -0.0116 | 9 |
| 1019 | 540.9588 | 0.0043 | -0.0179 | 9 |
| 1020 | 541.2331 | 0.0074 | 0.0167 | 10 |
| 1021 | 541.4451 | 0.0130 | -0.0110 | 9 |
| 1022 | 541.6939 | 0.0064 | -0.0019 | 9 |
| 1023 | 541.9539 | 0.0139 | 0.0184 | 10 |
| 1024 | 542.1690 | 0.0119 | -0.0062 | 10 |
| 1025 | 542.3848 | 0.0033 | -0.0301 | 9 |
| 1026 | 542.6378 | 0.0141 | -0.0168 | 9 |
| 1027 | 542.8716 | 0.0045 | -0.0227 | 10 |
| 1028 | 543.1216 | 0.0045 | -0.0124 | 9 |
| 1029 | 543.3531 | 0.0042 | -0.0206 | 9 |
| 1031 | 543.8507 | 0.0080 | -0.0024 | 8 |
| 1034 | 544.5895 | 0.0063 | 0.0173 | 10 |
| 1035 | 544.8267 | 0.0047 | 0.0148 | 10 |
| 1037 | 545.2731 | 0.0066 | -0.0182 | 9 |
| 1038 | 545.5277 | 0.0082 | -0.0033 | 10 |
| 1039 | 545.7629 | 0.0038 | -0.0078 | 9 |
| 1040 | 546.0121 | 0.0126 | 0.0017 | 9 |
| 1041 | 546.2589 | 0.0048 | 0.0088 | 9 |
| 1042 | 546.4987 | 0.0086 | 0.0089 | 10 |
| 1043 | 546.7434 | 0.0094 | 0.0139 | 9 |
| 1045 | 547.2273 | 0.0134 | 0.0184 | 7 |
| 1046 | 547.4232 | 0.0199 | -0.0254 | 10 |
| 1047 | 547.6680 | 0.0087 | -0.0203 | 9 |
| 1048 | 547.9098 | 0.0040 | -0.0182 | 9 |
| 1049 | 548.1514 | 0.0032 | -0.0163 | 10 |
| 1050 | 548.3712 | 0.0045 | -0.0362 | 10 |
| 1051 | 548.6021 | 0.0143 | -0.0450 | 9 |
| 1052 | 548.8744 | 0.0032 | -0.0124 | 9 |
| 1053 | 549.1091 | 0.0046 | -0.0174 | 10 |

**Table E1.** Times of negative-superhump maxima in KIC 9406652 during time interval 1 (BJD 2455296–2455553) (continued).

| $E^*$ | Max[†] | Error | $O-C^‡$ | $N^§$ |
|---|---|---|---|---|
| 1054 | 549.3632 | 0.0040 | -0.0030 | 9 |
| 1055 | 549.6210 | 0.0043 | 0.0151 | 9 |
| 1056 | 549.8471 | 0.0025 | 0.0015 | 9 |
| 1057 | 550.0946 | 0.0035 | 0.0093 | 10 |
| 1058 | 550.3553 | 0.0103 | 0.0303 | 8 |
| 1059 | 550.5971 | 0.0100 | 0.0324 | 9 |
| 1060 | 550.8448 | 0.0096 | 0.0404 | 10 |
| 1061 | 551.0530 | 0.0067 | 0.0089 | 10 |
| 1062 | 551.3087 | 0.0121 | 0.0249 | 9 |
| 1063 | 551.5281 | 0.0062 | 0.0046 | 9 |
| 1064 | 551.7761 | 0.0057 | 0.0129 | 10 |
| 1065 | 552.0132 | 0.0032 | 0.0103 | 9 |
| 1066 | 552.2421 | 0.0037 | -0.0005 | 9 |
| 1067 | 552.4707 | 0.0045 | -0.0116 | 7 |

[*] Cycle counts.
[†] BJD−2455000.0.
[‡] C = 2455296.7599+0.23970 E.
[§] Number of points used for determining the maximum.

**Table E2.** Times of negative-superhump maxima in KIC 9406652 during time interval 2 (BJD 2455568–2455643).

| $E^*$ | Max[†] | Error | $O-C$[‡] | $N$[§] |
|---|---|---|---|---|
| 0 | 568.5626 | 0.0085 | -0.0248 | 9 |
| 1 | 568.8204 | 0.0067 | -0.0068 | 10 |
| 2 | 569.0681 | 0.0118 | 0.0010 | 10 |
| 3 | 569.3158 | 0.0112 | 0.0088 | 9 |
| 4 | 569.5647 | 0.0081 | 0.0178 | 9 |
| 6 | 570.0264 | 0.0167 | -0.0002 | 10 |
| 7 | 570.2488 | 0.0068 | -0.0177 | 8 |
| 8 | 570.4523 | 0.0077 | -0.0541 | 9 |
| 9 | 570.7076 | 0.0068 | -0.0387 | 10 |
| 10 | 570.9531 | 0.0118 | -0.0330 | 10 |
| 11 | 571.1782 | 0.0027 | -0.0479 | 9 |
| 12 | 571.4433 | 0.0081 | -0.0226 | 9 |
| 13 | 571.6734 | 0.0028 | -0.0324 | 10 |
| 14 | 571.9232 | 0.0046 | -0.0225 | 10 |
| 15 | 572.1924 | 0.0119 | 0.0068 | 9 |
| 16 | 572.4193 | 0.0082 | -0.0062 | 9 |
| 17 | 572.6461 | 0.0125 | -0.0192 | 10 |
| 18 | 572.8870 | 0.0122 | -0.0182 | 9 |
| 19 | 573.1214 | 0.0031 | -0.0237 | 9 |
| 20 | 573.3567 | 0.0060 | -0.0282 | 9 |
| 21 | 573.6049 | 0.0063 | -0.0199 | 10 |
| 22 | 573.8439 | 0.0035 | -0.0209 | 9 |
| 23 | 574.0802 | 0.0053 | -0.0244 | 9 |
| 24 | 574.2967 | 0.0091 | -0.0477 | 9 |
| 25 | 574.5544 | 0.0046 | -0.0300 | 10 |
| 26 | 574.7985 | 0.0063 | -0.0257 | 9 |
| 27 | 575.0400 | 0.0056 | -0.0241 | 9 |
| 28 | 575.2615 | 0.0051 | -0.0425 | 10 |
| 29 | 575.5019 | 0.0057 | -0.0420 | 10 |
| 30 | 575.7518 | 0.0043 | -0.0319 | 9 |
| 31 | 575.9824 | 0.0057 | -0.0413 | 9 |
| 32 | 576.2358 | 0.0030 | -0.0277 | 9 |
| 33 | 576.4727 | 0.0079 | -0.0307 | 10 |
| 34 | 576.7112 | 0.0055 | -0.0321 | 9 |
| 35 | 576.9501 | 0.0097 | -0.0331 | 9 |
| 36 | 577.1937 | 0.0049 | -0.0294 | 10 |
| 37 | 577.4127 | 0.0086 | -0.0502 | 10 |
| 38 | 577.6632 | 0.0126 | -0.0396 | 9 |
| 40 | 578.2122 | 0.0169 | 0.0296 | 10 |
| 41 | 578.4007 | 0.0094 | -0.0217 | 9 |
| 45 | 579.4331 | 0.0199 | 0.0511 | 9 |
| 46 | 579.6456 | 0.0121 | 0.0237 | 9 |
| 47 | 579.8757 | 0.0154 | 0.0140 | 9 |
| 52 | 581.0195 | 0.0158 | -0.0416 | 10 |
| 53 | 581.2638 | 0.0059 | -0.0372 | 9 |
| 54 | 581.5354 | 0.0081 | -0.0055 | 9 |
| 55 | 581.8082 | 0.0104 | 0.0275 | 10 |
| 56 | 582.0123 | 0.0053 | -0.0084 | 10 |
| 57 | 582.2936 | 0.0098 | 0.0331 | 8 |
| 58 | 582.5463 | 0.0105 | 0.0459 | 9 |
| 59 | 582.7621 | 0.0108 | 0.0218 | 10 |
| 61 | 583.2528 | 0.0044 | 0.0328 | 8 |

**Table E2.** Times of negative-superhump maxima in KIC 9406652 during time interval 2 (BJD 2455568–2455643) (continued).

| $E^*$ | Max[†] | Error | $O-C$[‡] | $N$[§] |
|---|---|---|---|---|
| 62 | 583.4530 | 0.0060 | -0.0069 | 9 |
| 63 | 583.6982 | 0.0042 | -0.0016 | 10 |
| 64 | 583.9639 | 0.0051 | 0.0242 | 9 |
| 65 | 584.1932 | 0.0074 | 0.0136 | 9 |
| 66 | 584.4058 | 0.0039 | -0.0136 | 9 |
| 67 | 584.6328 | 0.0065 | -0.0265 | 10 |
| 68 | 584.9005 | 0.0139 | 0.0013 | 9 |
| 69 | 585.1412 | 0.0110 | 0.0021 | 8 |
| 70 | 585.3714 | 0.0035 | -0.0075 | 9 |
| 71 | 585.6207 | 0.0040 | 0.0018 | 10 |
| 72 | 585.8741 | 0.0030 | 0.0154 | 9 |
| 73 | 586.1219 | 0.0143 | 0.0233 | 6 |
| 74 | 586.3487 | 0.0039 | 0.0102 | 10 |
| 75 | 586.6000 | 0.0022 | 0.0217 | 10 |
| 76 | 586.8287 | 0.0036 | 0.0105 | 9 |
| 77 | 587.0738 | 0.0063 | 0.0157 | 9 |
| 78 | 587.3055 | 0.0068 | 0.0075 | 10 |
| 79 | 587.5296 | 0.0059 | -0.0082 | 10 |
| 80 | 587.7895 | 0.0087 | 0.0117 | 9 |
| 81 | 587.9925 | 0.0062 | -0.0251 | 9 |
| 82 | 588.2443 | 0.0060 | -0.0132 | 9 |
| 83 | 588.4808 | 0.0038 | -0.0166 | 10 |
| 84 | 588.7349 | 0.0033 | -0.0024 | 9 |
| 85 | 588.9756 | 0.0052 | -0.0016 | 9 |
| 86 | 589.2293 | 0.0051 | 0.0122 | 10 |
| 87 | 589.4653 | 0.0051 | 0.0084 | 10 |
| 88 | 589.7130 | 0.0049 | 0.0162 | 9 |
| 89 | 589.9505 | 0.0065 | 0.0139 | 9 |
| 90 | 590.1898 | 0.0057 | 0.0133 | 10 |
| 91 | 590.4502 | 0.0034 | 0.0337 | 9 |
| 92 | 590.6825 | 0.0057 | 0.0261 | 9 |
| 93 | 590.9173 | 0.0068 | 0.0211 | 9 |
| 94 | 591.1692 | 0.0096 | 0.0331 | 9 |
| 95 | 591.4132 | 0.0117 | 0.0373 | 9 |
| 96 | 591.6432 | 0.0083 | 0.0274 | 9 |
| 97 | 591.8688 | 0.0059 | 0.0131 | 9 |
| 98 | 592.1036 | 0.0048 | 0.0080 | 10 |
| 99 | 592.3371 | 0.0042 | 0.0017 | 9 |
| 100 | 592.5744 | 0.0058 | -0.0010 | 9 |
| 101 | 592.8204 | 0.0037 | 0.0052 | 10 |
| 102 | 593.0603 | 0.0066 | 0.0052 | 10 |
| 103 | 593.2990 | 0.0041 | 0.0040 | 9 |
| 104 | 593.5356 | 0.0022 | 0.0007 | 9 |
| 105 | 593.7763 | 0.0019 | 0.0015 | 9 |
| 106 | 594.0711 | 0.0051 | 0.0565 | 7 |
| 118 | 596.8946 | 0.0136 | 0.0014 | 9 |
| 119 | 597.1367 | 0.0024 | 0.0036 | 9 |
| 120 | 597.3933 | 0.0031 | 0.0203 | 9 |
| 121 | 597.6185 | 0.0082 | 0.0056 | 10 |
| 122 | 597.8628 | 0.0071 | 0.0100 | 9 |
| 123 | 598.1140 | 0.0029 | 0.0214 | 9 |
| 124 | 598.3352 | 0.0074 | 0.0028 | 10 |

**Table E2.** Times of negative-superhump maxima in KIC 9406652 during time interval 2 (BJD 2455568–2455643) (continued).

| $E^*$ | Max$^\dagger$ | Error | $O-C^\ddagger$ | $N^\S$ |
|---|---|---|---|---|
| 125 | 598.6001 | 0.0035 | 0.0278 | 10 |
| 126 | 598.8344 | 0.0048 | 0.0222 | 9 |
| 127 | 599.0734 | 0.0070 | 0.0212 | 9 |
| 128 | 599.3295 | 0.0072 | 0.0375 | 10 |
| 129 | 599.5583 | 0.0071 | 0.0265 | 10 |
| 130 | 599.8001 | 0.0094 | 0.0283 | 9 |
| 131 | 600.0332 | 0.0125 | 0.0215 | 9 |
| 132 | 600.2689 | 0.0109 | 0.0173 | 10 |
| 133 | 600.4941 | 0.0078 | 0.0027 | 10 |
| 134 | 600.7442 | 0.0034 | 0.0129 | 9 |
| 135 | 600.9822 | 0.0048 | 0.0111 | 9 |
| 136 | 601.2218 | 0.0047 | 0.0108 | 10 |
| 137 | 601.4519 | 0.0048 | 0.0010 | 9 |
| 138 | 601.7044 | 0.0037 | 0.0136 | 9 |
| 139 | 601.9275 | 0.0036 | -0.0032 | 8 |
| 140 | 602.1931 | 0.0016 | 0.0225 | 10 |
| 141 | 602.4279 | 0.0059 | 0.0175 | 9 |
| 142 | 602.6763 | 0.0056 | 0.0260 | 9 |
| 143 | 602.9050 | 0.0034 | 0.0148 | 9 |
| 144 | 603.1395 | 0.0049 | 0.0094 | 10 |
| 145 | 603.3879 | 0.0071 | 0.0179 | 9 |
| 146 | 603.6267 | 0.0082 | 0.0169 | 9 |
| 147 | 603.8732 | 0.0070 | 0.0235 | 10 |
| 148 | 604.1100 | 0.0066 | 0.0204 | 10 |
| 149 | 604.3387 | 0.0096 | 0.0093 | 9 |
| 150 | 604.5797 | 0.0069 | 0.0103 | 9 |
| 151 | 604.8080 | 0.0050 | -0.0012 | 9 |
| 152 | 605.0756 | 0.0075 | 0.0265 | 10 |
| 153 | 605.2665 | 0.0053 | -0.0225 | 9 |
| 154 | 605.5151 | 0.0021 | -0.0138 | 9 |
| 155 | 605.7698 | 0.0033 | 0.0011 | 9 |
| 156 | 606.0109 | 0.0051 | 0.0023 | 10 |
| 157 | 606.2667 | 0.0029 | 0.0182 | 9 |
| 158 | 606.5053 | 0.0012 | 0.0169 | 9 |
| 159 | 606.7392 | 0.0036 | 0.0109 | 10 |
| 160 | 606.9774 | 0.0010 | 0.0093 | 9 |
| 161 | 607.2306 | 0.0042 | 0.0226 | 9 |
| 162 | 607.4735 | 0.0031 | 0.0256 | 9 |
| 163 | 607.7046 | 0.0044 | 0.0168 | 10 |
| 164 | 607.9545 | 0.0095 | 0.0268 | 8 |
| 165 | 608.1710 | 0.0045 | 0.0034 | 9 |
| 166 | 608.4186 | 0.0069 | 0.0112 | 9 |
| 167 | 608.6431 | 0.0043 | -0.0042 | 10 |
| 168 | 608.8753 | 0.0032 | -0.0119 | 9 |
| 169 | 609.1109 | 0.0069 | -0.0162 | 9 |
| 170 | 609.3548 | 0.0031 | -0.0122 | 10 |
| 171 | 609.6006 | 0.0032 | -0.0063 | 10 |
| 172 | 609.8424 | 0.0015 | -0.0043 | 9 |
| 173 | 610.0918 | 0.0031 | 0.0052 | 9 |
| 174 | 610.3242 | 0.0028 | -0.0023 | 10 |
| 175 | 610.5609 | 0.0029 | -0.0054 | 10 |
| 176 | 610.8146 | 0.0057 | 0.0084 | 8 |

**Table E2.** Times of negative-superhump maxima in KIC 9406652 during time interval 2 (BJD 2455568–2455643) (continued).

| $E^*$ | Max$^\dagger$ | Error | $O-C^\ddagger$ | $N^\S$ |
|---|---|---|---|---|
| 177 | 611.0383 | 0.0026 | -0.0078 | 9 |
| 178 | 611.3065 | 0.0026 | 0.0205 | 10 |
| 179 | 611.5343 | 0.0022 | 0.0085 | 10 |
| 180 | 611.7737 | 0.0040 | 0.0080 | 9 |
| 181 | 612.0096 | 0.0039 | 0.0039 | 9 |
| 182 | 612.2526 | 0.0042 | 0.0070 | 10 |
| 183 | 612.4711 | 0.0027 | -0.0143 | 9 |
| 184 | 612.7018 | 0.0062 | -0.0234 | 9 |
| 185 | 612.9546 | 0.0054 | -0.0106 | 9 |
| 186 | 613.1822 | 0.0039 | -0.0229 | 10 |
| 187 | 613.4190 | 0.0056 | -0.0259 | 9 |
| 188 | 613.6699 | 0.0028 | -0.0149 | 9 |
| 189 | 613.9086 | 0.0073 | -0.0161 | 7 |
| 190 | 614.1529 | 0.0033 | -0.0117 | 10 |
| 191 | 614.3994 | 0.0047 | -0.0050 | 9 |
| 192 | 614.6282 | 0.0032 | -0.0161 | 9 |
| 193 | 614.8767 | 0.0023 | -0.0075 | 10 |
| 194 | 615.1119 | 0.0011 | -0.0122 | 9 |
| 195 | 615.3634 | 0.0044 | -0.0006 | 9 |
| 196 | 615.6101 | 0.0040 | 0.0063 | 9 |
| 197 | 615.8446 | 0.0061 | 0.0009 | 10 |
| 198 | 616.0862 | 0.0024 | 0.0026 | 10 |
| 199 | 616.3048 | 0.0066 | -0.0187 | 9 |
| 200 | 616.5473 | 0.0055 | -0.0160 | 9 |
| 201 | 616.7890 | 0.0033 | -0.0143 | 9 |
| 202 | 617.0122 | 0.0063 | -0.0309 | 10 |
| 203 | 617.2688 | 0.0050 | -0.0142 | 9 |
| 204 | 617.5037 | 0.0032 | -0.0192 | 9 |
| 205 | 617.7401 | 0.0045 | -0.0226 | 10 |
| 206 | 617.9942 | 0.0029 | -0.0085 | 10 |
| 207 | 618.2257 | 0.0034 | -0.0168 | 9 |
| 208 | 618.4688 | 0.0035 | -0.0136 | 9 |
| 209 | 618.7047 | 0.0038 | -0.0176 | 10 |
| 210 | 618.9604 | 0.0062 | -0.0017 | 9 |
| 211 | 619.1840 | 0.0043 | -0.0180 | 9 |
| 212 | 619.4249 | 0.0048 | -0.0170 | 8 |
| 213 | 619.6729 | 0.0071 | -0.0089 | 10 |
| 214 | 619.9094 | 0.0041 | -0.0122 | 9 |
| 215 | 620.1398 | 0.0042 | -0.0218 | 9 |
| 216 | 620.3811 | 0.0032 | -0.0203 | 9 |
| 217 | 620.6226 | 0.0060 | -0.0188 | 10 |
| 218 | 620.8407 | 0.0075 | -0.0405 | 9 |
| 219 | 621.0753 | 0.0058 | -0.0458 | 9 |
| 220 | 621.3330 | 0.0045 | -0.0280 | 10 |
| 221 | 621.5654 | 0.0025 | -0.0355 | 10 |
| 222 | 621.7987 | 0.0064 | -0.0421 | 9 |
| 223 | 622.0415 | 0.0067 | -0.0391 | 8 |
| 224 | 622.2915 | 0.0036 | -0.0290 | 10 |
| 225 | 622.5277 | 0.0026 | -0.0327 | 10 |
| 226 | 622.7632 | 0.0074 | -0.0370 | 8 |
| 227 | 622.9880 | 0.0094 | -0.0521 | 9 |
| 228 | 623.2508 | 0.0070 | -0.0292 | 10 |

**Table E2.** Times of negative-superhump maxima in KIC 9406652 during time interval 2 (BJD 2455568–2455643) (continued).

| $E^*$ | Max† | Error | $O-C$‡ | $N$§ |
|---|---|---|---|---|
| 229 | 623.4702 | 0.0066 | -0.0497 | 10 |
| 231 | 623.9493 | 0.0175 | -0.0503 | 9 |
| 232 | 624.1975 | 0.0075 | -0.0420 | 10 |
| 233 | 624.4292 | 0.0167 | -0.0502 | 9 |
| 234 | 624.6840 | 0.0095 | -0.0353 | 9 |
| 235 | 624.9617 | 0.0078 | 0.0025 | 7 |
| 236 | 625.1800 | 0.0098 | -0.0190 | 10 |
| 237 | 625.4119 | 0.0084 | -0.0270 | 9 |
| 238 | 625.6555 | 0.0057 | -0.0233 | 8 |
| 239 | 625.9117 | 0.0146 | -0.0070 | 9 |
| 240 | 626.1362 | 0.0153 | -0.0224 | 10 |
| 241 | 626.3541 | 0.0092 | -0.0443 | 9 |
| 242 | 626.6132 | 0.0105 | -0.0251 | 9 |
| 243 | 626.8331 | 0.0190 | -0.0451 | 10 |
| 244 | 627.1074 | 0.0041 | -0.0107 | 10 |
| 245 | 627.3289 | 0.0120 | -0.0290 | 9 |
| 246 | 627.5740 | 0.0056 | -0.0238 | 9 |
| 247 | 627.8154 | 0.0034 | -0.0223 | 10 |
| 248 | 628.0811 | 0.0049 | 0.0035 | 10 |
| 249 | 628.3105 | 0.0064 | -0.0070 | 9 |
| 250 | 628.5623 | 0.0105 | 0.0049 | 9 |
| 254 | 629.5487 | 0.0198 | 0.0319 | 9 |
| 255 | 629.7374 | 0.0107 | -0.0193 | 10 |
| 256 | 630.0128 | 0.0152 | 0.0161 | 9 |
| 257 | 630.2890 | 0.0058 | 0.0525 | 9 |
| 258 | 630.4434 | 0.0092 | -0.0330 | 9 |
| 259 | 630.7015 | 0.0094 | -0.0147 | 10 |
| 260 | 630.9511 | 0.0065 | -0.0050 | 9 |
| 261 | 631.1876 | 0.0049 | -0.0085 | 9 |
| 262 | 631.4380 | 0.0057 | 0.0021 | 9 |
| 263 | 631.7060 | 0.0048 | 0.0302 | 8 |
| 264 | 631.9042 | 0.0071 | -0.0115 | 9 |
| 265 | 632.1613 | 0.0054 | 0.0058 | 9 |
| 266 | 632.3962 | 0.0057 | 0.0007 | 10 |
| 267 | 632.6340 | 0.0030 | -0.0013 | 10 |
| 268 | 632.8734 | 0.0056 | -0.0018 | 9 |
| 269 | 633.1229 | 0.0081 | 0.0078 | 9 |
| 270 | 633.3634 | 0.0074 | 0.0085 | 10 |

**Table E2.** Times of negative-superhump maxima in KIC 9406652 during time interval 2 (BJD 2455568–2455643) (continued).

| $E^*$ | Max† | Error | $O-C$‡ | $N$§ |
|---|---|---|---|---|
| 271 | 633.5984 | 0.0036 | 0.0035 | 10 |
| 272 | 633.8273 | 0.0081 | -0.0074 | 9 |
| 273 | 634.0625 | 0.0014 | -0.0121 | 9 |
| 274 | 634.3083 | 0.0035 | -0.0062 | 10 |
| 275 | 634.5471 | 0.0036 | -0.0072 | 10 |
| 276 | 634.7963 | 0.0025 | 0.0021 | 8 |
| 277 | 635.0253 | 0.0155 | -0.0088 | 9 |
| 278 | 635.2587 | 0.0048 | -0.0153 | 9 |
| 305 | 641.7797 | 0.0065 | 0.0290 | 10 |
| 306 | 642.0186 | 0.0089 | 0.0279 | 9 |
| 307 | 642.2587 | 0.0029 | 0.0282 | 9 |
| 308 | 642.4840 | 0.0031 | 0.0136 | 9 |
| 309 | 642.7233 | 0.0031 | 0.0130 | 10 |
| 310 | 642.9696 | 0.0047 | 0.0194 | 9 |

*Cycle counts.

†BJD−2455000.0.

‡ C = 245568.5626+0.23988 E.

§Number of points used for determining the maximum.

**Table E3.** Times of negative-superhump maxima in KIC 9406652 during time interval 3 (BJD 2455643–2455871).

| $E^*$ | Max$^\dagger$ | Error | $O-C^\ddagger$ | $N^\S$ |
|---|---|---|---|---|
| 0 | 643.2055 | 0.0031 | -0.0268 | 9 |
| 1 | 643.4588 | 0.0015 | -0.0134 | 9 |
| 2 | 643.7037 | 0.0040 | -0.0085 | 9 |
| 3 | 643.9427 | 0.0032 | -0.0093 | 9 |
| 4 | 644.1825 | 0.0036 | -0.0094 | 9 |
| 5 | 644.4224 | 0.0033 | -0.0094 | 9 |
| 6 | 644.6651 | 0.0048 | -0.0065 | 10 |
| 7 | 644.8902 | 0.0082 | -0.0213 | 9 |
| 8 | 645.1367 | 0.0040 | -0.0147 | 9 |
| 9 | 645.3766 | 0.0024 | -0.0147 | 10 |
| 10 | 645.6285 | 0.0035 | -0.0027 | 10 |
| 11 | 645.8587 | 0.0036 | -0.0124 | 9 |
| 12 | 646.0937 | 0.0021 | -0.0172 | 9 |
| 13 | 646.3391 | 0.0022 | -0.0117 | 10 |
| 14 | 646.5743 | 0.0056 | -0.0164 | 8 |
| 15 | 646.8265 | 0.0023 | -0.0040 | 9 |
| 16 | 647.0498 | 0.0071 | -0.0207 | 9 |
| 17 | 647.3018 | 0.0037 | -0.0085 | 10 |
| 18 | 647.5449 | 0.0017 | -0.0053 | 10 |
| 19 | 647.7848 | 0.0039 | -0.0052 | 9 |
| 20 | 648.0158 | 0.0046 | -0.0142 | 9 |
| 21 | 648.2634 | 0.0041 | -0.0065 | 10 |
| 22 | 648.4991 | 0.0016 | -0.0107 | 9 |
| 23 | 648.7515 | 0.0055 | 0.0019 | 9 |
| 24 | 648.9880 | 0.0062 | -0.0015 | 9 |
| 25 | 649.2199 | 0.0078 | -0.0094 | 10 |
| 26 | 649.4527 | 0.0026 | -0.0165 | 9 |
| 27 | 649.6979 | 0.0093 | -0.0112 | 9 |
| 28 | 649.9349 | 0.0020 | -0.0141 | 9 |
| 29 | 650.1671 | 0.0031 | -0.0218 | 10 |
| 30 | 650.4061 | 0.0023 | -0.0227 | 9 |
| 31 | 650.6528 | 0.0021 | -0.0159 | 9 |
| 32 | 650.8950 | 0.0018 | -0.0135 | 9 |
| 33 | 651.1229 | 0.0047 | -0.0255 | 10 |
| 34 | 651.3806 | 0.0030 | -0.0077 | 9 |
| 35 | 651.6093 | 0.0031 | -0.0189 | 9 |
| 36 | 651.8674 | 0.0045 | -0.0006 | 10 |
| 37 | 652.0968 | 0.0040 | -0.0111 | 9 |
| 38 | 652.3298 | 0.0039 | -0.0180 | 9 |
| 39 | 652.5922 | 0.0028 | 0.0045 | 8 |
| 40 | 652.8192 | 0.0044 | -0.0083 | 10 |
| 41 | 653.0436 | 0.0031 | -0.0238 | 10 |
| 42 | 653.2920 | 0.0071 | -0.0153 | 9 |
| 43 | 653.5334 | 0.0036 | -0.0138 | 9 |
| 44 | 653.7709 | 0.0065 | -0.0162 | 9 |
| 45 | 653.9856 | 0.0071 | -0.0413 | 9 |
| 46 | 654.2513 | 0.0009 | -0.0155 | 9 |
| 47 | 654.4928 | 0.0037 | -0.0139 | 9 |
| 48 | 654.7196 | 0.0029 | -0.0270 | 10 |
| 49 | 654.9584 | 0.0050 | -0.0281 | 9 |
| 50 | 655.2015 | 0.0031 | -0.0248 | 9 |
| 51 | 655.4466 | 0.0046 | -0.0196 | 9 |

**Table E3.** Times of negative-superhump maxima in KIC 9406652 during time interval 3 (BJD 2455643–2455871) (continued).

| $E^*$ | Max$^\dagger$ | Error | $O-C^\ddagger$ | $N^\S$ |
|---|---|---|---|---|
| 52 | 655.6797 | 0.0045 | -0.0264 | 10 |
| 53 | 655.9219 | 0.0070 | -0.0241 | 9 |
| 54 | 656.1676 | 0.0042 | -0.0182 | 9 |
| 55 | 656.4044 | 0.0037 | -0.0214 | 10 |
| 56 | 656.6396 | 0.0028 | -0.0261 | 10 |
| 57 | 656.8932 | 0.0027 | -0.0124 | 9 |
| 58 | 657.1148 | 0.0053 | -0.0306 | 9 |
| 59 | 657.3603 | 0.0067 | -0.0250 | 10 |
| 60 | 657.6114 | 0.0065 | -0.0138 | 9 |
| 61 | 657.8293 | 0.0044 | -0.0358 | 9 |
| 62 | 658.0635 | 0.0100 | -0.0414 | 9 |
| 63 | 658.3163 | 0.0034 | -0.0285 | 10 |
| 64 | 658.5697 | 0.0054 | -0.0150 | 9 |
| 65 | 658.8081 | 0.0027 | -0.0165 | 9 |
| 66 | 659.0376 | 0.0053 | -0.0269 | 9 |
| 67 | 659.2789 | 0.0057 | -0.0255 | 10 |
| 68 | 659.5169 | 0.0071 | -0.0273 | 9 |
| 69 | 659.7575 | 0.0045 | -0.0266 | 9 |
| 70 | 659.9983 | 0.0068 | -0.0257 | 9 |
| 71 | 660.2377 | 0.0032 | -0.0261 | 10 |
| 72 | 660.4762 | 0.0062 | -0.0275 | 9 |
| 73 | 660.7175 | 0.0024 | -0.0261 | 9 |
| 74 | 660.9672 | 0.0056 | -0.0163 | 9 |
| 75 | 661.1843 | 0.0092 | -0.0390 | 10 |
| 76 | 661.4178 | 0.0108 | -0.0454 | 8 |
| 78 | 661.8887 | 0.0070 | -0.0543 | 10 |
| 79 | 662.1475 | 0.0075 | -0.0353 | 10 |
| 80 | 662.3798 | 0.0031 | -0.0430 | 9 |
| 81 | 662.6253 | 0.0020 | -0.0373 | 9 |
| 82 | 662.8560 | 0.0023 | -0.0465 | 10 |
| 83 | 663.1015 | 0.0030 | -0.0409 | 10 |
| 84 | 663.3404 | 0.0065 | -0.0418 | 9 |
| 85 | 663.5916 | 0.0047 | -0.0305 | 9 |
| 86 | 663.8195 | 0.0065 | -0.0425 | 10 |
| 87 | 664.0723 | 0.0051 | -0.0296 | 10 |
| 88 | 664.3067 | 0.0089 | -0.0351 | 9 |
| 89 | 664.5555 | 0.0065 | -0.0262 | 8 |
| 90 | 664.7778 | 0.0027 | -0.0438 | 9 |
| 91 | 665.0170 | 0.0051 | -0.0444 | 9 |
| 92 | 665.2647 | 0.0051 | -0.0366 | 9 |
| 93 | 665.4839 | 0.0053 | -0.0573 | 9 |
| 94 | 665.7427 | 0.0035 | -0.0384 | 10 |
| 95 | 665.9708 | 0.0029 | -0.0501 | 9 |
| 96 | 666.2109 | 0.0088 | -0.0500 | 9 |
| 99 | 666.9438 | 0.0078 | -0.0367 | 9 |
| 100 | 667.1758 | 0.0066 | -0.0445 | 9 |
| 101 | 667.4106 | 0.0036 | -0.0496 | 9 |
| 102 | 667.6518 | 0.0057 | -0.0483 | 10 |
| 103 | 667.9009 | 0.0036 | -0.0391 | 9 |
| 104 | 668.1409 | 0.0034 | -0.0389 | 9 |
| 105 | 668.3972 | 0.0024 | -0.0226 | 10 |
| 106 | 668.6392 | 0.0035 | -0.0204 | 10 |

**Table E3.** Times of negative-superhump maxima in KIC 9406652 during time interval 3 (BJD 2455643–2455871) (continued).

| $E^*$ | Max$^\dagger$ | Error | $O-C^\ddagger$ | $N^\S$ |
|---|---|---|---|---|
| 107 | 668.8903 | 0.0028 | -0.0092 | 9 |
| 108 | 669.1153 | 0.0076 | -0.0241 | 9 |
| 109 | 669.3602 | 0.0110 | -0.0190 | 10 |
| 116 | 671.0149 | 0.0093 | -0.0435 | 9 |
| 117 | 671.2631 | 0.0064 | -0.0352 | 10 |
| 119 | 671.7301 | 0.0124 | -0.0480 | 9 |
| 121 | 672.2220 | 0.0103 | -0.0358 | 10 |
| 122 | 672.4753 | 0.0122 | -0.0224 | 9 |
| 123 | 672.6951 | 0.0074 | -0.0425 | 9 |
| 128 | 673.8916 | 0.0076 | -0.0454 | 10 |
| 129 | 674.1547 | 0.0065 | -0.0222 | 10 |
| 130 | 674.4035 | 0.0054 | -0.0132 | 9 |
| 132 | 674.8845 | 0.0088 | -0.0120 | 10 |
| 133 | 675.1269 | 0.0083 | -0.0095 | 10 |
| 134 | 675.3788 | 0.0085 | 0.0025 | 9 |
| 136 | 675.8570 | 0.0103 | 0.0010 | 10 |
| 137 | 676.0840 | 0.0087 | -0.0119 | 9 |
| 138 | 676.3011 | 0.0075 | -0.0347 | 9 |
| 139 | 676.6032 | 0.0180 | 0.0275 | 9 |
| 140 | 676.7963 | 0.0082 | -0.0192 | 10 |
| 141 | 677.0163 | 0.0070 | -0.0392 | 9 |
| 142 | 677.2594 | 0.0088 | -0.0359 | 9 |
| 144 | 677.7691 | 0.0111 | -0.0060 | 10 |
| 148 | 678.6851 | 0.0074 | -0.0495 | 10 |
| 149 | 678.9306 | 0.0061 | -0.0439 | 9 |
| 150 | 679.1907 | 0.0044 | -0.0237 | 9 |
| 151 | 679.4158 | 0.0025 | -0.0385 | 10 |
| 152 | 679.6609 | 0.0040 | -0.0333 | 10 |
| 153 | 679.8955 | 0.0030 | -0.0384 | 9 |
| 154 | 680.1541 | 0.0032 | -0.0198 | 9 |
| 155 | 680.3862 | 0.0025 | -0.0276 | 10 |
| 156 | 680.6272 | 0.0017 | -0.0264 | 9 |
| 157 | 680.8730 | 0.0034 | -0.0205 | 8 |
| 158 | 681.1313 | 0.0029 | -0.0021 | 9 |
| 159 | 681.3684 | 0.0042 | -0.0049 | 10 |
| 160 | 681.6179 | 0.0034 | 0.0048 | 9 |
| 161 | 681.8494 | 0.0037 | -0.0036 | 9 |
| 162 | 682.1136 | 0.0058 | 0.0207 | 9 |
| 163 | 682.3481 | 0.0029 | 0.0153 | 10 |
| 165 | 682.8442 | 0.0190 | 0.0317 | 9 |
| 167 | 683.2523 | 0.0048 | -0.0400 | 9 |
| 168 | 683.4942 | 0.0050 | -0.0380 | 9 |
| 169 | 683.7424 | 0.0023 | -0.0297 | 9 |
| 170 | 684.0055 | 0.0031 | -0.0065 | 9 |
| 171 | 684.2260 | 0.0052 | -0.0259 | 10 |
| 172 | 684.4709 | 0.0162 | -0.0209 | 9 |
| 173 | 684.7200 | 0.0051 | -0.0116 | 9 |
| 174 | 684.9494 | 0.0058 | -0.0221 | 7 |
| 175 | 685.2028 | 0.0107 | -0.0086 | 10 |
| 176 | 685.4303 | 0.0085 | -0.0209 | 9 |
| 177 | 685.6602 | 0.0096 | -0.0309 | 9 |
| 178 | 685.9269 | 0.0043 | -0.0041 | 10 |

**Table E3.** Times of negative-superhump maxima in KIC 9406652 during time interval 3 (BJD 2455643–2455871) (continued).

| $E^*$ | Max$^\dagger$ | Error | $O-C^\ddagger$ | $N^\S$ |
|---|---|---|---|---|
| 179 | 686.1641 | 0.0028 | -0.0068 | 9 |
| 180 | 686.4088 | 0.0056 | -0.0019 | 9 |
| 181 | 686.6360 | 0.0058 | -0.0146 | 9 |
| 182 | 686.8835 | 0.0078 | -0.0070 | 9 |
| 183 | 687.1040 | 0.0026 | -0.0264 | 9 |
| 184 | 687.3512 | 0.0041 | -0.0191 | 9 |
| 185 | 687.5906 | 0.0051 | -0.0196 | 9 |
| 186 | 687.8360 | 0.0019 | -0.0140 | 10 |
| 187 | 688.0798 | 0.0036 | -0.0101 | 9 |
| 188 | 688.3210 | 0.0028 | -0.0088 | 9 |
| 189 | 688.5485 | 0.0033 | -0.0211 | 10 |
| 190 | 688.7924 | 0.0035 | -0.0171 | 10 |
| 191 | 689.0378 | 0.0029 | -0.0116 | 9 |
| 192 | 689.2800 | 0.0030 | -0.0094 | 9 |
| 193 | 689.5306 | 0.0032 | 0.0014 | 10 |
| 194 | 689.7590 | 0.0050 | -0.0101 | 10 |
| 195 | 690.0059 | 0.0030 | -0.0030 | 9 |
| 196 | 690.2400 | 0.0031 | -0.0088 | 9 |
| 197 | 690.4961 | 0.0055 | 0.0074 | 10 |
| 198 | 690.7256 | 0.0044 | -0.0030 | 10 |
| 199 | 690.9549 | 0.0069 | -0.0136 | 9 |
| 200 | 691.1874 | 0.0019 | -0.0209 | 9 |
| 201 | 691.4220 | 0.0035 | -0.0262 | 10 |
| 202 | 691.6650 | 0.0033 | -0.0231 | 9 |
| 203 | 691.8998 | 0.0062 | -0.0282 | 9 |
| 204 | 692.1443 | 0.0061 | -0.0236 | 9 |
| 205 | 692.3811 | 0.0018 | -0.0267 | 10 |
| 206 | 692.6261 | 0.0034 | -0.0215 | 9 |
| 207 | 692.8604 | 0.0049 | -0.0271 | 8 |
| 208 | 693.1145 | 0.0035 | -0.0129 | 9 |
| 209 | 693.3434 | 0.0046 | -0.0238 | 10 |
| 210 | 693.5963 | 0.0056 | -0.0109 | 9 |
| 211 | 693.8351 | 0.0027 | -0.0120 | 9 |
| 212 | 694.0703 | 0.0023 | -0.0166 | 10 |
| 213 | 694.3000 | 0.0038 | -0.0268 | 10 |
| 214 | 694.5420 | 0.0051 | -0.0247 | 9 |
| 215 | 694.7918 | 0.0039 | -0.0148 | 9 |
| 216 | 695.0220 | 0.0038 | -0.0244 | 10 |
| 217 | 695.2712 | 0.0055 | -0.0152 | 10 |
| 218 | 695.4964 | 0.0047 | -0.0298 | 9 |
| 219 | 695.7392 | 0.0068 | -0.0269 | 8 |
| 220 | 695.9821 | 0.0047 | -0.0238 | 10 |
| 221 | 696.2235 | 0.0024 | -0.0223 | 10 |
| 222 | 696.4622 | 0.0078 | -0.0236 | 9 |
| 223 | 696.6951 | 0.0032 | -0.0305 | 9 |
| 224 | 696.9380 | 0.0046 | -0.0275 | 10 |
| 225 | 697.1753 | 0.0037 | -0.0300 | 9 |
| 226 | 697.4188 | 0.0041 | -0.0265 | 9 |
| 227 | 697.6587 | 0.0052 | -0.0264 | 9 |
| 228 | 697.9004 | 0.0047 | -0.0246 | 10 |
| 229 | 698.1561 | 0.0020 | -0.0088 | 9 |
| 230 | 698.4015 | 0.0032 | -0.0033 | 9 |

**Table E3.** Times of negative-superhump maxima in KIC 9406652 during time interval 3 (BJD 2455643–2455871) (continued).

| $E^*$ | Max[†] | Error | $O-C$[‡] | $N$[§] |
|---|---|---|---|---|
| 231 | 698.6453 | 0.0050 | 0.0007 | 9 |
| 232 | 698.8882 | 0.0046 | 0.0037 | 9 |
| 233 | 699.0932 | 0.0143 | -0.0312 | 9 |
| 234 | 699.3308 | 0.0159 | -0.0335 | 9 |
| 235 | 699.5642 | 0.0089 | -0.0399 | 10 |
| 236 | 699.8034 | 0.0047 | -0.0407 | 10 |
| 237 | 700.0477 | 0.0105 | -0.0363 | 9 |
| 238 | 700.2995 | 0.0078 | -0.0243 | 9 |
| 239 | 700.5248 | 0.0064 | -0.0389 | 10 |
| 240 | 700.7709 | 0.0030 | -0.0327 | 10 |
| 241 | 701.0065 | 0.0036 | -0.0369 | 9 |
| 242 | 701.2508 | 0.0070 | -0.0326 | 9 |
| 243 | 701.4994 | 0.0065 | -0.0238 | 10 |
| 244 | 701.7418 | 0.0085 | -0.0212 | 9 |
| 245 | 701.9818 | 0.0066 | -0.0212 | 9 |
| 246 | 702.2595 | 0.0124 | 0.0166 | 9 |
| 247 | 702.4768 | 0.0110 | -0.0059 | 10 |
| 249 | 702.9924 | 0.0109 | 0.0299 | 9 |
| 250 | 703.2003 | 0.0110 | -0.0021 | 9 |
| 252 | 703.7353 | 0.0170 | 0.0532 | 8 |
| 254 | 704.1559 | 0.0059 | -0.0060 | 9 |
| 255 | 704.3963 | 0.0061 | -0.0055 | 10 |
| 256 | 704.6047 | 0.0172 | -0.0369 | 9 |
| 257 | 704.8994 | 0.0066 | 0.0179 | 8 |
| 259 | 705.3723 | 0.0080 | 0.0110 | 9 |
| 264 | 706.5241 | 0.0118 | -0.0366 | 9 |
| 265 | 706.7505 | 0.0082 | -0.0501 | 9 |
| 266 | 707.0163 | 0.0059 | -0.0241 | 9 |
| 270 | 707.9716 | 0.0101 | -0.0283 | 10 |
| 271 | 708.2426 | 0.0034 | 0.0027 | 9 |
| 272 | 708.4772 | 0.0092 | -0.0025 | 9 |
| 273 | 708.7597 | 0.0074 | 0.0401 | 9 |
| 274 | 709.0010 | 0.0114 | 0.0416 | 10 |
| 277 | 709.6816 | 0.0051 | 0.0025 | 9 |
| 278 | 709.9223 | 0.0109 | 0.0033 | 9 |
| 279 | 710.1694 | 0.0166 | 0.0105 | 9 |
| 280 | 710.3877 | 0.0089 | -0.0111 | 9 |
| 281 | 710.6272 | 0.0039 | -0.0115 | 10 |
| 282 | 710.8773 | 0.0035 | -0.0012 | 9 |
| 283 | 711.1235 | 0.0023 | 0.0051 | 9 |
| 284 | 711.3576 | 0.0034 | -0.0006 | 9 |
| 285 | 711.6103 | 0.0031 | 0.0121 | 10 |
| 286 | 711.8528 | 0.0048 | 0.0148 | 10 |
| 287 | 712.0906 | 0.0047 | 0.0127 | 9 |
| 288 | 712.3407 | 0.0018 | 0.0229 | 9 |
| 289 | 712.5632 | 0.0040 | 0.0055 | 10 |
| 290 | 712.8032 | 0.0045 | 0.0056 | 10 |
| 291 | 713.0387 | 0.0056 | 0.0013 | 8 |
| 292 | 713.2850 | 0.0032 | 0.0077 | 9 |
| 293 | 713.5169 | 0.0020 | -0.0003 | 10 |
| 294 | 713.7643 | 0.0014 | 0.0072 | 9 |
| 295 | 714.0145 | 0.0044 | 0.0175 | 8 |

**Table E3.** Times of negative-superhump maxima in KIC 9406652 during time interval 3 (BJD 2455643–2455871) (continued).

| $E^*$ | Max[†] | Error | $O-C$[‡] | $N$[§] |
|---|---|---|---|---|
| 296 | 714.2443 | 0.0015 | 0.0074 | 9 |
| 297 | 714.4934 | 0.0014 | 0.0167 | 10 |
| 298 | 714.7375 | 0.0014 | 0.0209 | 9 |
| 299 | 714.9827 | 0.0020 | 0.0262 | 9 |
| 300 | 715.2293 | 0.0014 | 0.0329 | 9 |
| 301 | 715.4698 | 0.0011 | 0.0335 | 10 |
| 302 | 715.7185 | 0.0042 | 0.0424 | 9 |
| 303 | 715.9649 | 0.0047 | 0.0489 | 8 |
| 304 | 716.1866 | 0.0052 | 0.0307 | 10 |
| 305 | 716.4150 | 0.0069 | 0.0192 | 10 |
| 306 | 716.6596 | 0.0036 | 0.0239 | 9 |
| 307 | 716.9031 | 0.0050 | 0.0276 | 9 |
| 308 | 717.1410 | 0.0030 | 0.0256 | 10 |
| 309 | 717.3740 | 0.0044 | 0.0187 | 10 |
| 310 | 717.6165 | 0.0028 | 0.0213 | 9 |
| 311 | 717.8594 | 0.0050 | 0.0244 | 9 |
| 312 | 718.1075 | 0.0052 | 0.0326 | 9 |
| 313 | 718.3287 | 0.0056 | 0.0139 | 10 |
| 314 | 718.5751 | 0.0017 | 0.0204 | 9 |
| 315 | 718.8150 | 0.0044 | 0.0204 | 9 |
| 316 | 719.0654 | 0.0031 | 0.0309 | 9 |
| 317 | 719.2959 | 0.0033 | 0.0216 | 9 |
| 318 | 719.5342 | 0.0035 | 0.0200 | 9 |
| 323 | 720.7362 | 0.0038 | 0.0226 | 9 |
| 324 | 720.9856 | 0.0039 | 0.0321 | 10 |
| 325 | 721.2194 | 0.0022 | 0.0261 | 8 |
| 326 | 721.4536 | 0.0037 | 0.0203 | 9 |
| 327 | 721.6904 | 0.0020 | 0.0173 | 10 |
| 328 | 721.9244 | 0.0033 | 0.0114 | 9 |
| 329 | 722.1743 | 0.0031 | 0.0214 | 9 |
| 330 | 722.4088 | 0.0025 | 0.0160 | 9 |
| 331 | 722.6479 | 0.0016 | 0.0153 | 10 |
| 332 | 722.8852 | 0.0026 | 0.0127 | 10 |
| 333 | 723.1318 | 0.0029 | 0.0194 | 9 |
| 334 | 723.3712 | 0.0030 | 0.0189 | 9 |
| 335 | 723.6157 | 0.0027 | 0.0236 | 10 |
| 336 | 723.8583 | 0.0022 | 0.0262 | 10 |
| 337 | 724.0920 | 0.0015 | 0.0201 | 9 |
| 338 | 724.3436 | 0.0030 | 0.0318 | 9 |
| 339 | 724.5782 | 0.0029 | 0.0265 | 10 |
| 340 | 724.8183 | 0.0044 | 0.0268 | 9 |
| 341 | 725.0519 | 0.0020 | 0.0204 | 9 |
| 342 | 725.3040 | 0.0027 | 0.0327 | 9 |
| 343 | 725.5376 | 0.0029 | 0.0264 | 10 |
| 344 | 725.7783 | 0.0022 | 0.0272 | 9 |
| 345 | 726.0143 | 0.0030 | 0.0234 | 9 |
| 346 | 726.2550 | 0.0017 | 0.0241 | 9 |
| 347 | 726.4859 | 0.0023 | 0.0152 | 10 |
| 348 | 726.7314 | 0.0031 | 0.0208 | 9 |
| 349 | 726.9714 | 0.0027 | 0.0210 | 9 |
| 350 | 727.2128 | 0.0024 | 0.0224 | 10 |
| 351 | 727.4438 | 0.0017 | 0.0135 | 10 |

**Table E3.** Times of negative-superhump maxima in KIC 9406652 during time interval 3 (BJD 2455643–2455871) (continued).

| $E^*$ | Max$^\dagger$ | Error | $O-C^\ddagger$ | $N^\S$ |
|---|---|---|---|---|
| 352 | 727.6906 | 0.0028 | 0.0205 | 9 |
| 353 | 727.9326 | 0.0017 | 0.0226 | 8 |
| 354 | 728.1675 | 0.0021 | 0.0176 | 10 |
| 355 | 728.4146 | 0.0013 | 0.0248 | 10 |
| 356 | 728.6482 | 0.0035 | 0.0185 | 9 |
| 357 | 728.8928 | 0.0036 | 0.0233 | 9 |
| 358 | 729.1258 | 0.0017 | 0.0164 | 10 |
| 359 | 729.3738 | 0.0032 | 0.0245 | 10 |
| 360 | 729.6054 | 0.0039 | 0.0163 | 9 |
| 361 | 729.8403 | 0.0052 | 0.0112 | 9 |
| 362 | 730.0796 | 0.0028 | 0.0107 | 10 |
| 363 | 730.3199 | 0.0050 | 0.0111 | 9 |
| 364 | 730.5600 | 0.0038 | 0.0113 | 9 |
| 365 | 730.7927 | 0.0029 | 0.0041 | 8 |
| 366 | 731.0336 | 0.0025 | 0.0052 | 10 |
| 367 | 731.2819 | 0.0015 | 0.0136 | 9 |
| 368 | 731.5192 | 0.0021 | 0.0110 | 9 |
| 369 | 731.7563 | 0.0008 | 0.0082 | 9 |
| 370 | 732.0004 | 0.0018 | 0.0124 | 10 |
| 371 | 732.2433 | 0.0015 | 0.0154 | 9 |
| 372 | 732.4846 | 0.0027 | 0.0169 | 9 |
| 373 | 732.7177 | 0.0032 | 0.0101 | 10 |
| 374 | 732.9673 | 0.0032 | 0.0198 | 10 |
| 375 | 733.2011 | 0.0015 | 0.0138 | 9 |
| 376 | 733.4373 | 0.0024 | 0.0100 | 8 |
| 377 | 733.6732 | 0.0023 | 0.0061 | 10 |
| 378 | 733.9131 | 0.0039 | 0.0061 | 9 |
| 379 | 734.1546 | 0.0022 | 0.0077 | 9 |
| 380 | 734.3848 | 0.0021 | -0.0019 | 9 |
| 381 | 734.6271 | 0.0033 | 0.0005 | 10 |
| 382 | 734.8657 | 0.0023 | -0.0008 | 10 |
| 383 | 735.1009 | 0.0024 | -0.0055 | 9 |
| 384 | 735.3441 | 0.0014 | -0.0022 | 9 |
| 385 | 735.5839 | 0.0028 | -0.0023 | 10 |
| 386 | 735.8272 | 0.0020 | 0.0011 | 9 |
| 387 | 736.0689 | 0.0015 | 0.0029 | 9 |
| 388 | 736.3101 | 0.0013 | 0.0043 | 9 |
| 389 | 736.5483 | 0.0022 | 0.0026 | 10 |
| 390 | 736.7852 | 0.0031 | -0.0003 | 8 |
| 391 | 737.0168 | 0.0027 | -0.0087 | 9 |
| 392 | 737.2694 | 0.0012 | 0.0041 | 9 |
| 393 | 737.5110 | 0.0029 | 0.0058 | 10 |
| 394 | 737.7509 | 0.0020 | 0.0058 | 9 |
| 395 | 737.9843 | 0.0033 | -0.0007 | 9 |
| 396 | 738.2039 | 0.0030 | -0.0209 | 10 |
| 397 | 738.4509 | 0.0021 | -0.0138 | 10 |
| 398 | 738.6895 | 0.0021 | -0.0151 | 9 |
| 403 | 739.9071 | 0.0026 | 0.0031 | 7 |
| 404 | 740.1384 | 0.0027 | -0.0055 | 10 |
| 405 | 740.3702 | 0.0052 | -0.0135 | 10 |
| 406 | 740.6093 | 0.0028 | -0.0143 | 9 |
| 411 | 741.8217 | 0.0104 | -0.0013 | 9 |

**Table E3.** Times of negative-superhump maxima in KIC 9406652 during time interval 3 (BJD 2455643–2455871) (continued).

| $E^*$ | Max$^\dagger$ | Error | $O-C^\ddagger$ | $N^\S$ |
|---|---|---|---|---|
| 412 | 742.0670 | 0.0061 | 0.0040 | 10 |
| 421 | 744.1952 | 0.0059 | -0.0267 | 9 |
| 422 | 744.4389 | 0.0116 | -0.0228 | 9 |
| 423 | 744.6868 | 0.0102 | -0.0148 | 10 |
| 425 | 745.1642 | 0.0044 | -0.0172 | 9 |
| 426 | 745.4031 | 0.0094 | -0.0182 | 9 |
| 427 | 745.6721 | 0.0060 | 0.0110 | 10 |
| 428 | 745.8968 | 0.0101 | -0.0042 | 10 |
| 433 | 747.1057 | 0.0069 | 0.0053 | 9 |
| 435 | 747.6322 | 0.0137 | 0.0520 | 10 |
| 437 | 748.0397 | 0.0134 | -0.0202 | 9 |
| 438 | 748.2552 | 0.0026 | -0.0446 | 9 |
| 439 | 748.5234 | 0.0121 | -0.0163 | 9 |
| 440 | 748.7368 | 0.0065 | -0.0428 | 9 |
| 441 | 749.0044 | 0.0023 | -0.0151 | 9 |
| 442 | 749.2494 | 0.0033 | -0.0099 | 10 |
| 443 | 749.4894 | 0.0026 | -0.0098 | 10 |
| 444 | 749.7440 | 0.0029 | 0.0049 | 9 |
| 445 | 750.0056 | 0.0025 | 0.0266 | 9 |
| 446 | 750.2362 | 0.0070 | 0.0173 | 10 |
| 447 | 750.4807 | 0.0051 | 0.0220 | 10 |
| 448 | 750.7284 | 0.0033 | 0.0298 | 9 |
| 449 | 750.9901 | 0.0040 | 0.0516 | 8 |
| 450 | 751.2146 | 0.0020 | 0.0363 | 10 |
| 451 | 751.4408 | 0.0039 | 0.0226 | 10 |
| 452 | 751.6940 | 0.0023 | 0.0359 | 9 |
| 453 | 751.9294 | 0.0013 | 0.0314 | 9 |
| 454 | 752.1679 | 0.0021 | 0.0300 | 10 |
| 455 | 752.4126 | 0.0023 | 0.0349 | 9 |
| 456 | 752.6564 | 0.0024 | 0.0388 | 9 |
| 457 | 752.8977 | 0.0015 | 0.0401 | 9 |
| 458 | 753.1437 | 0.0016 | 0.0463 | 10 |
| 459 | 753.3877 | 0.0023 | 0.0504 | 9 |
| 460 | 753.6342 | 0.0030 | 0.0570 | 9 |
| 465 | 754.8223 | 0.0044 | 0.0457 | 10 |
| 466 | 755.0524 | 0.0059 | 0.0360 | 10 |
| 468 | 755.5294 | 0.0044 | 0.0332 | 9 |
| 469 | 755.7852 | 0.0050 | 0.0491 | 10 |
| 470 | 756.0165 | 0.0021 | 0.0405 | 10 |
| 471 | 756.2595 | 0.0031 | 0.0437 | 9 |
| 472 | 756.4969 | 0.0023 | 0.0412 | 9 |
| 473 | 756.7403 | 0.0029 | 0.0447 | 10 |
| 474 | 756.9792 | 0.0050 | 0.0437 | 7 |
| 475 | 757.2208 | 0.0025 | 0.0454 | 8 |
| 476 | 757.4583 | 0.0020 | 0.0431 | 9 |
| 477 | 757.7082 | 0.0024 | 0.0531 | 10 |
| 478 | 757.9463 | 0.0017 | 0.0513 | 9 |
| 479 | 758.1835 | 0.0018 | 0.0487 | 9 |
| 480 | 758.4213 | 0.0025 | 0.0465 | 9 |
| 481 | 758.6684 | 0.0016 | 0.0538 | 10 |
| 482 | 758.9082 | 0.0027 | 0.0537 | 9 |
| 483 | 759.1427 | 0.0046 | 0.0483 | 9 |

**Table E3.** Times of negative-superhump maxima in KIC 9406652 during time interval 3 (BJD 2455643–2455871) (continued).

| $E^*$ | Max$^\dagger$ | Error | $O-C^\ddagger$ | $N^\S$ |
|---|---|---|---|---|
| 484 | 759.3905 | 0.0020 | 0.0562 | 9 |
| 485 | 759.6316 | 0.0024 | 0.0574 | 10 |
| 486 | 759.8709 | 0.0024 | 0.0569 | 8 |
| 487 | 760.1105 | 0.0023 | 0.0565 | 9 |
| 488 | 760.3523 | 0.0029 | 0.0585 | 10 |
| 489 | 760.5854 | 0.0021 | 0.0517 | 10 |
| 490 | 760.8258 | 0.0027 | 0.0523 | 9 |
| 491 | 761.0597 | 0.0042 | 0.0463 | 9 |
| 492 | 761.3083 | 0.0021 | 0.0550 | 10 |
| 493 | 761.5470 | 0.0024 | 0.0538 | 10 |
| 494 | 761.7871 | 0.0014 | 0.0540 | 9 |
| 495 | 762.0262 | 0.0041 | 0.0533 | 9 |
| 496 | 762.2711 | 0.0029 | 0.0583 | 10 |
| 497 | 762.5028 | 0.0033 | 0.0501 | 10 |
| 498 | 762.7180 | 0.0073 | 0.0254 | 9 |
| 500 | 763.2280 | 0.0038 | 0.0556 | 10 |
| 501 | 763.4647 | 0.0016 | 0.0525 | 8 |
| 502 | 763.7045 | 0.0012 | 0.0524 | 9 |
| 503 | 763.9424 | 0.0034 | 0.0504 | 9 |
| 504 | 764.1849 | 0.0021 | 0.0530 | 10 |
| 505 | 764.4198 | 0.0016 | 0.0481 | 9 |
| 506 | 764.6637 | 0.0029 | 0.0520 | 9 |
| 507 | 764.9076 | 0.0017 | 0.0561 | 9 |
| 508 | 765.1384 | 0.0020 | 0.0470 | 10 |
| 509 | 765.3754 | 0.0015 | 0.0441 | 9 |
| 510 | 765.6151 | 0.0018 | 0.0439 | 9 |
| 511 | 765.8553 | 0.0021 | 0.0443 | 9 |
| 512 | 766.0944 | 0.0024 | 0.0435 | 10 |
| 513 | 766.3307 | 0.0017 | 0.0399 | 9 |
| 514 | 766.5743 | 0.0036 | 0.0436 | 9 |
| 515 | 766.8161 | 0.0022 | 0.0455 | 10 |
| 516 | 767.0454 | 0.0027 | 0.0349 | 10 |
| 517 | 767.2950 | 0.0015 | 0.0446 | 9 |
| 518 | 767.5307 | 0.0018 | 0.0405 | 9 |
| 519 | 767.7766 | 0.0021 | 0.0466 | 10 |
| 520 | 768.0099 | 0.0028 | 0.0399 | 10 |
| 521 | 768.2491 | 0.0041 | 0.0392 | 9 |
| 522 | 768.4899 | 0.0015 | 0.0402 | 9 |
| 523 | 768.7301 | 0.0025 | 0.0405 | 10 |
| 525 | 769.2006 | 0.0021 | 0.0312 | 9 |
| 526 | 769.4436 | 0.0024 | 0.0343 | 9 |
| 527 | 769.6839 | 0.0014 | 0.0348 | 10 |
| 528 | 769.9251 | 0.0017 | 0.0360 | 8 |
| 532 | 770.8826 | 0.0028 | 0.0341 | 7 |
| 533 | 771.1151 | 0.0064 | 0.0267 | 9 |
| 534 | 771.3597 | 0.0031 | 0.0315 | 10 |
| 535 | 771.6010 | 0.0014 | 0.0328 | 10 |
| 536 | 771.8412 | 0.0023 | 0.0332 | 9 |
| 537 | 772.0766 | 0.0017 | 0.0286 | 9 |
| 538 | 772.3185 | 0.0024 | 0.0307 | 10 |
| 539 | 772.5537 | 0.0034 | 0.0260 | 10 |
| 540 | 772.7955 | 0.0030 | 0.0279 | 9 |

**Table E3.** Times of negative-superhump maxima in KIC 9406652 during time interval 3 (BJD 2455643–2455871) (continued).

| $E^*$ | Max$^\dagger$ | Error | $O-C^\ddagger$ | $N^\S$ |
|---|---|---|---|---|
| 541 | 773.0236 | 0.0027 | 0.0161 | 8 |
| 542 | 773.2743 | 0.0017 | 0.0270 | 10 |
| 543 | 773.5111 | 0.0024 | 0.0239 | 10 |
| 544 | 773.7504 | 0.0080 | 0.0233 | 9 |
| 545 | 773.9885 | 0.0018 | 0.0215 | 9 |
| 546 | 774.2246 | 0.0020 | 0.0178 | 10 |
| 547 | 774.4692 | 0.0018 | 0.0225 | 9 |
| 548 | 774.7059 | 0.0028 | 0.0193 | 9 |
| 549 | 774.9475 | 0.0053 | 0.0210 | 9 |
| 550 | 775.1846 | 0.0031 | 0.0182 | 10 |
| 551 | 775.4283 | 0.0029 | 0.0220 | 9 |
| 552 | 775.6670 | 0.0025 | 0.0209 | 9 |
| 553 | 775.9075 | 0.0028 | 0.0215 | 8 |
| 554 | 776.1458 | 0.0033 | 0.0200 | 10 |
| 555 | 776.3905 | 0.0035 | 0.0248 | 9 |
| 556 | 776.6251 | 0.0029 | 0.0195 | 9 |
| 557 | 776.8605 | 0.0036 | 0.0150 | 10 |
| 558 | 777.1013 | 0.0034 | 0.0159 | 10 |
| 559 | 777.3294 | 0.0028 | 0.0041 | 9 |
| 560 | 777.5716 | 0.0015 | 0.0064 | 9 |
| 561 | 777.8036 | 0.0029 | -0.0015 | 10 |
| 562 | 778.0430 | 0.0024 | -0.0020 | 10 |
| 563 | 778.2834 | 0.0022 | -0.0014 | 9 |
| 564 | 778.5199 | 0.0023 | -0.0047 | 9 |
| 565 | 778.7600 | 0.0011 | -0.0046 | 10 |
| 566 | 778.9966 | 0.0046 | -0.0078 | 9 |
| 567 | 779.2461 | 0.0018 | 0.0018 | 9 |
| 568 | 779.4874 | 0.0024 | 0.0032 | 9 |
| 569 | 779.7276 | 0.0021 | 0.0036 | 10 |
| 570 | 779.9720 | 0.0037 | 0.0080 | 10 |
| 571 | 780.2063 | 0.0015 | 0.0025 | 9 |
| 572 | 780.4497 | 0.0031 | 0.0060 | 9 |
| 573 | 780.6883 | 0.0028 | 0.0047 | 10 |
| 574 | 780.9231 | 0.0026 | -0.0004 | 9 |
| 575 | 781.1554 | 0.0027 | -0.0080 | 9 |
| 576 | 781.3937 | 0.0032 | -0.0096 | 9 |
| 577 | 781.6305 | 0.0024 | -0.0127 | 10 |
| 578 | 781.8657 | 0.0032 | -0.0173 | 8 |
| 579 | 782.1229 | 0.0023 | 0.0001 | 9 |
| 580 | 782.3478 | 0.0017 | -0.0149 | 9 |
| 581 | 782.6005 | 0.0043 | -0.0022 | 10 |
| 582 | 782.8291 | 0.0036 | -0.0134 | 9 |
| 583 | 783.0699 | 0.0025 | -0.0125 | 9 |
| 584 | 783.3078 | 0.0034 | -0.0144 | 10 |
| 585 | 783.6002 | 0.0116 | 0.0380 | 10 |
| 586 | 783.7832 | 0.0116 | -0.0189 | 9 |
| 587 | 784.0180 | 0.0075 | -0.0239 | 9 |
| 588 | 784.2714 | 0.0051 | -0.0104 | 10 |
| 589 | 784.5209 | 0.0085 | -0.0007 | 10 |
| 590 | 784.7323 | 0.0094 | -0.0293 | 9 |
| 591 | 785.0035 | 0.0105 | 0.0021 | 9 |
| 592 | 785.2476 | 0.0161 | 0.0062 | 10 |

**Table E3.** Times of negative-superhump maxima in KIC 9406652 during time interval 3 (BJD 2455643–2455871) (continued).

| $E^*$ | Max$^\dagger$ | Error | $O-C^\ddagger$ | $N^\S$ |
|---|---|---|---|---|
| 593 | 785.5025 | 0.0074 | 0.0213 | 10 |
| 594 | 785.7165 | 0.0034 | -0.0046 | 9 |
| 595 | 785.9464 | 0.0051 | -0.0146 | 9 |
| 596 | 786.1958 | 0.0123 | -0.0051 | 10 |
| 597 | 786.4142 | 0.0062 | -0.0265 | 9 |
| 598 | 786.6660 | 0.0116 | -0.0146 | 9 |
| 599 | 786.9093 | 0.0050 | -0.0112 | 9 |
| 600 | 787.1729 | 0.0061 | 0.0125 | 10 |
| 601 | 787.3740 | 0.0074 | -0.0263 | 9 |
| 602 | 787.6390 | 0.0074 | -0.0011 | 9 |
| 604 | 788.1475 | 0.0047 | 0.0276 | 10 |
| 605 | 788.3668 | 0.0058 | 0.0071 | 9 |
| 606 | 788.6021 | 0.0070 | 0.0024 | 9 |
| 607 | 788.8559 | 0.0104 | 0.0164 | 10 |
| 608 | 789.1022 | 0.0073 | 0.0228 | 10 |
| 609 | 789.3619 | 0.0100 | 0.0426 | 9 |
| 612 | 790.0219 | 0.0056 | -0.0170 | 10 |
| 613 | 790.2616 | 0.0022 | -0.0172 | 9 |
| 614 | 790.4868 | 0.0058 | -0.0319 | 9 |
| 615 | 790.7431 | 0.0026 | -0.0154 | 10 |
| 616 | 790.9788 | 0.0052 | -0.0196 | 10 |
| 617 | 791.2278 | 0.0044 | -0.0105 | 9 |
| 618 | 791.4940 | 0.0029 | 0.0158 | 9 |
| 619 | 791.7339 | 0.0021 | 0.0158 | 10 |
| 620 | 791.9835 | 0.0019 | 0.0255 | 9 |
| 621 | 792.2165 | 0.0061 | 0.0186 | 9 |
| 622 | 792.4595 | 0.0034 | 0.0218 | 9 |
| 623 | 792.6899 | 0.0029 | 0.0123 | 10 |
| 624 | 792.9323 | 0.0016 | 0.0148 | 9 |
| 625 | 793.1688 | 0.0035 | 0.0115 | 9 |
| 626 | 793.4168 | 0.0022 | 0.0195 | 9 |
| 627 | 793.6400 | 0.0026 | 0.0029 | 10 |
| 628 | 793.8985 | 0.0029 | 0.0215 | 8 |
| 629 | 794.1297 | 0.0016 | 0.0128 | 9 |
| 630 | 794.3783 | 0.0016 | 0.0215 | 10 |
| 631 | 794.6153 | 0.0019 | 0.0186 | 10 |
| 632 | 794.8606 | 0.0023 | 0.0241 | 9 |
| 633 | 795.0960 | 0.0035 | 0.0196 | 9 |
| 634 | 795.3417 | 0.0032 | 0.0255 | 10 |
| 635 | 795.5816 | 0.0025 | 0.0255 | 10 |
| 636 | 795.8196 | 0.0021 | 0.0235 | 9 |
| 637 | 796.0572 | 0.0018 | 0.0213 | 9 |
| 638 | 796.2989 | 0.0013 | 0.0231 | 10 |
| 639 | 796.5349 | 0.0026 | 0.0192 | 10 |
| 640 | 796.7803 | 0.0042 | 0.0248 | 8 |
| 641 | 797.0118 | 0.0028 | 0.0163 | 9 |
| 642 | 797.2614 | 0.0030 | 0.0261 | 10 |
| 643 | 797.5007 | 0.0027 | 0.0255 | 9 |
| 644 | 797.7439 | 0.0013 | 0.0289 | 9 |
| 645 | 797.9786 | 0.0034 | 0.0237 | 6 |
| 646 | 798.2163 | 0.0011 | 0.0214 | 10 |
| 647 | 798.4476 | 0.0012 | 0.0129 | 9 |

**Table E3.** Times of negative-superhump maxima in KIC 9406652 during time interval 3 (BJD 2455643–2455871) (continued).

| $E^*$ | Max$^\dagger$ | Error | $O-C^\ddagger$ | $N^\S$ |
|---|---|---|---|---|
| 648 | 798.6896 | 0.0043 | 0.0150 | 9 |
| 649 | 798.9294 | 0.0031 | 0.0149 | 9 |
| 650 | 799.1662 | 0.0021 | 0.0119 | 10 |
| 651 | 799.4123 | 0.0027 | 0.0180 | 9 |
| 652 | 799.6564 | 0.0043 | 0.0223 | 7 |
| 653 | 799.8868 | 0.0029 | 0.0128 | 9 |
| 654 | 800.1346 | 0.0021 | 0.0207 | 10 |
| 655 | 800.3730 | 0.0013 | 0.0192 | 9 |
| 656 | 800.6169 | 0.0019 | 0.0233 | 9 |
| 657 | 800.8592 | 0.0019 | 0.0257 | 10 |
| 658 | 801.0968 | 0.0019 | 0.0234 | 10 |
| 659 | 801.3346 | 0.0032 | 0.0213 | 9 |
| 660 | 801.5729 | 0.0014 | 0.0198 | 9 |
| 661 | 801.8100 | 0.0013 | 0.0170 | 10 |
| 662 | 802.0538 | 0.0014 | 0.0208 | 10 |
| 667 | 803.2433 | 0.0018 | 0.0110 | 9 |
| 668 | 803.4885 | 0.0026 | 0.0163 | 9 |
| 669 | 803.7244 | 0.0027 | 0.0123 | 10 |
| 670 | 803.9678 | 0.0012 | 0.0158 | 9 |
| 671 | 804.2090 | 0.0013 | 0.0171 | 9 |
| 672 | 804.4502 | 0.0016 | 0.0185 | 9 |
| 673 | 804.6880 | 0.0013 | 0.0164 | 10 |
| 674 | 804.9275 | 0.0040 | 0.0160 | 8 |
| 675 | 805.1626 | 0.0014 | 0.0113 | 9 |
| 676 | 805.4045 | 0.0015 | 0.0132 | 10 |
| 677 | 805.6460 | 0.0018 | 0.0148 | 10 |
| 678 | 805.8816 | 0.0011 | 0.0106 | 9 |
| 679 | 806.1266 | 0.0011 | 0.0157 | 9 |
| 680 | 806.3569 | 0.0024 | 0.0061 | 10 |
| 681 | 806.5947 | 0.0027 | 0.0041 | 10 |
| 682 | 806.8393 | 0.0030 | 0.0088 | 8 |
| 683 | 807.0753 | 0.0050 | 0.0049 | 8 |
| 684 | 807.3078 | 0.0017 | -0.0025 | 10 |
| 685 | 807.5539 | 0.0010 | 0.0038 | 10 |
| 686 | 807.7852 | 0.0013 | -0.0048 | 9 |
| 687 | 808.0329 | 0.0013 | 0.0030 | 8 |
| 688 | 808.2703 | 0.0020 | 0.0005 | 9 |
| 689 | 808.5143 | 0.0018 | 0.0046 | 9 |
| 690 | 808.7525 | 0.0013 | 0.0029 | 9 |
| 691 | 808.9993 | 0.0022 | 0.0099 | 9 |
| 692 | 809.2332 | 0.0018 | 0.0039 | 10 |
| 693 | 809.4709 | 0.0013 | 0.0017 | 9 |
| 694 | 809.7089 | 0.0020 | -0.0001 | 9 |
| 695 | 809.9511 | 0.0014 | 0.0022 | 9 |
| 696 | 810.1884 | 0.0012 | -0.0005 | 10 |
| 697 | 810.4307 | 0.0013 | 0.0020 | 9 |
| 698 | 810.6671 | 0.0011 | -0.0015 | 9 |
| 699 | 810.9039 | 0.0025 | -0.0046 | 8 |
| 700 | 811.1400 | 0.0028 | -0.0083 | 10 |
| 701 | 811.3782 | 0.0019 | -0.0100 | 9 |
| 702 | 811.6148 | 0.0017 | -0.0134 | 9 |
| 703 | 811.8555 | 0.0013 | -0.0125 | 10 |

**Table E3.** Times of negative-superhump maxima in KIC 9406652 during time interval 3 (BJD 2455643–2455871) (continued).

| $E^*$ | Max$^\dagger$ | Error | $O-C^\ddagger$ | $N^\S$ |
|---|---|---|---|---|
| 704 | 812.0958 | 0.0018 | -0.0121 | 10 |
| 705 | 812.3395 | 0.0020 | -0.0083 | 9 |
| 706 | 812.5797 | 0.0017 | -0.0080 | 9 |
| 707 | 812.8248 | 0.0022 | -0.0027 | 10 |
| 708 | 813.0509 | 0.0029 | -0.0165 | 10 |
| 709 | 813.2999 | 0.0028 | -0.0074 | 9 |
| 710 | 813.5324 | 0.0045 | -0.0147 | 9 |
| 711 | 813.7814 | 0.0017 | -0.0056 | 10 |
| 712 | 814.0099 | 0.0015 | -0.0171 | 9 |
| 713 | 814.2500 | 0.0013 | -0.0168 | 9 |
| 714 | 814.4839 | 0.0031 | -0.0228 | 9 |
| 715 | 814.7259 | 0.0023 | -0.0207 | 10 |
| 716 | 814.9676 | 0.0039 | -0.0189 | 9 |
| 717 | 815.1953 | 0.0030 | -0.0310 | 9 |
| 718 | 815.4339 | 0.0030 | -0.0323 | 9 |
| 719 | 815.6761 | 0.0031 | -0.0300 | 10 |
| 720 | 815.9154 | 0.0030 | -0.0305 | 9 |
| 721 | 816.1596 | 0.0030 | -0.0263 | 9 |
| 722 | 816.4035 | 0.0021 | -0.0222 | 9 |
| 723 | 816.6416 | 0.0021 | -0.0240 | 10 |
| 724 | 816.8828 | 0.0031 | -0.0227 | 8 |
| 725 | 817.1211 | 0.0025 | -0.0243 | 9 |
| 726 | 817.3587 | 0.0035 | -0.0266 | 10 |
| 727 | 817.6016 | 0.0027 | -0.0235 | 10 |
| 728 | 817.8408 | 0.0025 | -0.0242 | 9 |
| 729 | 818.0766 | 0.0019 | -0.0283 | 9 |
| 730 | 818.3158 | 0.0035 | -0.0289 | 10 |
| 731 | 818.5462 | 0.0030 | -0.0384 | 10 |
| 732 | 818.7761 | 0.0067 | -0.0485 | 9 |
| 733 | 819.0257 | 0.0031 | -0.0387 | 9 |
| 734 | 819.2705 | 0.0019 | -0.0337 | 10 |
| 735 | 819.5076 | 0.0046 | -0.0366 | 10 |
| 736 | 819.7466 | 0.0051 | -0.0375 | 9 |
| 737 | 819.9785 | 0.0039 | -0.0454 | 9 |
| 738 | 820.2148 | 0.0033 | -0.0490 | 10 |
| 741 | 820.9527 | 0.0142 | -0.0308 | 9 |
| 742 | 821.2097 | 0.0106 | -0.0136 | 10 |
| 743 | 821.4414 | 0.0095 | -0.0218 | 9 |
| 744 | 821.6998 | 0.0097 | -0.0033 | 9 |
| 745 | 821.9180 | 0.0075 | -0.0250 | 9 |
| 746 | 822.1658 | 0.0098 | -0.0171 | 10 |
| 747 | 822.3747 | 0.0070 | -0.0480 | 9 |
| 748 | 822.6448 | 0.0093 | -0.0178 | 9 |
| 749 | 822.8768 | 0.0038 | -0.0257 | 9 |
| 750 | 823.0869 | 0.0041 | -0.0555 | 10 |
| 751 | 823.3659 | 0.0069 | -0.0164 | 9 |
| 752 | 823.5758 | 0.0099 | -0.0464 | 9 |
| 753 | 823.8205 | 0.0066 | -0.0415 | 10 |
| 754 | 824.0774 | 0.0058 | -0.0245 | 10 |
| 755 | 824.3013 | 0.0047 | -0.0405 | 9 |
| 756 | 824.5550 | 0.0067 | -0.0267 | 9 |
| 758 | 825.0358 | 0.0080 | -0.0256 | 10 |

**Table E3.** Times of negative-superhump maxima in KIC 9406652 during time interval 3 (BJD 2455643–2455871) (continued).

| $E^*$ | Max$^\dagger$ | Error | $O-C^\ddagger$ | $N^\S$ |
|---|---|---|---|---|
| 760 | 825.5426 | 0.0062 | 0.0014 | 9 |
| 761 | 825.7547 | 0.0063 | -0.0264 | 9 |
| 762 | 826.0342 | 0.0053 | 0.0133 | 9 |
| 764 | 826.5224 | 0.0164 | 0.0217 | 9 |
| 765 | 826.7950 | 0.0083 | 0.0545 | 10 |
| 769 | 827.6543 | 0.0037 | -0.0458 | 10 |
| 770 | 827.9016 | 0.0114 | -0.0384 | 9 |
| 771 | 828.1472 | 0.0020 | -0.0327 | 9 |
| 772 | 828.3942 | 0.0031 | -0.0256 | 10 |
| 773 | 828.6464 | 0.0023 | -0.0132 | 10 |
| 774 | 828.8851 | 0.0025 | -0.0144 | 7 |
| 775 | 829.1349 | 0.0015 | -0.0045 | 9 |
| 776 | 829.3703 | 0.0026 | -0.0089 | 10 |
| 777 | 829.6080 | 0.0015 | -0.0111 | 10 |
| 778 | 829.8473 | 0.0016 | -0.0117 | 9 |
| 779 | 830.0885 | 0.0030 | -0.0104 | 9 |
| 780 | 830.3286 | 0.0015 | -0.0102 | 10 |
| 781 | 830.5664 | 0.0009 | -0.0123 | 10 |
| 782 | 830.8102 | 0.0022 | -0.0083 | 9 |
| 783 | 831.0490 | 0.0036 | -0.0094 | 9 |
| 784 | 831.2966 | 0.0013 | -0.0017 | 10 |
| 785 | 831.5399 | 0.0015 | 0.0018 | 10 |
| 786 | 831.7832 | 0.0015 | 0.0051 | 8 |
| 787 | 832.0319 | 0.0034 | 0.0140 | 7 |
| 788 | 832.2692 | 0.0028 | 0.0114 | 10 |
| 789 | 832.5067 | 0.0035 | 0.0090 | 9 |
| 790 | 832.7517 | 0.0014 | 0.0142 | 9 |
| 791 | 832.9840 | 0.0013 | 0.0066 | 9 |
| 792 | 833.2172 | 0.0020 | -0.0001 | 8 |
| 797 | 834.4211 | 0.0027 | 0.0044 | 9 |
| 798 | 834.6616 | 0.0014 | 0.0050 | 9 |
| 799 | 834.8944 | 0.0020 | -0.0021 | 10 |
| 800 | 835.1403 | 0.0039 | 0.0040 | 10 |
| 801 | 835.3810 | 0.0032 | 0.0047 | 9 |
| 802 | 835.6146 | 0.0021 | -0.0015 | 9 |
| 803 | 835.8598 | 0.0026 | 0.0038 | 10 |
| 804 | 836.0960 | 0.0018 | 0.0001 | 10 |
| 805 | 836.3329 | 0.0009 | -0.0028 | 8 |
| 806 | 836.5677 | 0.0028 | -0.0079 | 9 |
| 807 | 836.8047 | 0.0043 | -0.0108 | 10 |
| 808 | 837.0302 | 0.0037 | -0.0252 | 9 |
| 809 | 837.2853 | 0.0026 | -0.0100 | 7 |
| 810 | 837.5218 | 0.0045 | -0.0134 | 9 |
| 811 | 837.7719 | 0.0019 | -0.0031 | 10 |
| 812 | 838.0129 | 0.0018 | -0.0020 | 9 |
| 813 | 838.2593 | 0.0018 | 0.0045 | 9 |
| 814 | 838.4975 | 0.0020 | 0.0028 | 9 |
| 815 | 838.7250 | 0.0023 | -0.0095 | 10 |
| 816 | 838.9776 | 0.0042 | 0.0032 | 9 |
| 817 | 839.2058 | 0.0023 | -0.0085 | 8 |
| 818 | 839.4569 | 0.0014 | 0.0027 | 9 |
| 819 | 839.6911 | 0.0025 | -0.0030 | 10 |

**Table E3.** Times of negative-superhump maxima in KIC 9406652 during time interval 3 (BJD 2455643–2455871) (continued).

| $E^*$ | Max$^\dagger$ | Error | $O-C^\ddagger$ | $N^\S$ |
|---|---|---|---|---|
| 820 | 839.9208 | 0.0010 | -0.0132 | 9 |
| 821 | 840.1700 | 0.0023 | -0.0039 | 9 |
| 822 | 840.4068 | 0.0024 | -0.0070 | 10 |
| 823 | 840.6501 | 0.0036 | -0.0035 | 10 |
| 824 | 840.8847 | 0.0014 | -0.0088 | 9 |
| 825 | 841.1249 | 0.0009 | -0.0085 | 9 |
| 826 | 841.3891 | 0.0107 | 0.0158 | 9 |
| 827 | 841.6078 | 0.0021 | -0.0053 | 10 |
| 828 | 841.8469 | 0.0010 | -0.0061 | 9 |
| 829 | 842.0855 | 0.0024 | -0.0074 | 9 |
| 830 | 842.3255 | 0.0036 | -0.0072 | 8 |
| 831 | 842.5639 | 0.0021 | -0.0087 | 10 |
| 832 | 842.8018 | 0.0023 | -0.0107 | 9 |
| 833 | 843.0439 | 0.0084 | -0.0085 | 7 |
| 834 | 843.2898 | 0.0028 | -0.0025 | 10 |
| 835 | 843.5260 | 0.0029 | -0.0062 | 10 |
| 836 | 843.7608 | 0.0037 | -0.0112 | 9 |
| 837 | 844.0031 | 0.0040 | -0.0089 | 9 |
| 838 | 844.2340 | 0.0017 | -0.0178 | 10 |
| 839 | 844.4675 | 0.0023 | -0.0242 | 9 |
| 840 | 844.7121 | 0.0039 | -0.0194 | 9 |
| 841 | 844.9280 | 0.0101 | -0.0435 | 9 |
| 842 | 845.1851 | 0.0130 | -0.0262 | 9 |
| 843 | 845.4298 | 0.0018 | -0.0214 | 9 |
| 844 | 845.6713 | 0.0026 | -0.0198 | 9 |
| 845 | 845.9149 | 0.0018 | -0.0160 | 9 |
| 846 | 846.1497 | 0.0024 | -0.0211 | 10 |
| 847 | 846.3926 | 0.0017 | -0.0181 | 9 |
| 848 | 846.6351 | 0.0015 | -0.0155 | 9 |
| 849 | 846.8714 | 0.0016 | -0.0191 | 10 |
| 850 | 847.1141 | 0.0030 | -0.0163 | 10 |
| 851 | 847.3452 | 0.0023 | -0.0250 | 8 |
| 852 | 847.5969 | 0.0015 | -0.0132 | 9 |
| 853 | 847.8304 | 0.0010 | -0.0196 | 10 |
| 854 | 848.0660 | 0.0011 | -0.0239 | 10 |
| 855 | 848.3033 | 0.0023 | -0.0264 | 9 |
| 856 | 848.5405 | 0.0021 | -0.0292 | 9 |
| 857 | 848.7748 | 0.0019 | -0.0347 | 9 |
| 858 | 849.0095 | 0.0014 | -0.0399 | 10 |
| 859 | 849.2565 | 0.0028 | -0.0327 | 9 |
| 860 | 849.4937 | 0.0019 | -0.0354 | 9 |
| 861 | 849.7406 | 0.0010 | -0.0285 | 10 |
| 862 | 849.9787 | 0.0026 | -0.0303 | 9 |
| 863 | 850.2107 | 0.0022 | -0.0381 | 9 |
| 864 | 850.4553 | 0.0020 | -0.0333 | 9 |
| 865 | 850.6924 | 0.0026 | -0.0361 | 10 |
| 866 | 850.9358 | 0.0054 | -0.0326 | 9 |
| 867 | 851.1717 | 0.0024 | -0.0366 | 8 |
| 868 | 851.4069 | 0.0026 | -0.0413 | 9 |
| 869 | 851.6547 | 0.0038 | -0.0334 | 10 |
| 870 | 851.8883 | 0.0035 | -0.0397 | 9 |
| 871 | 852.1299 | 0.0092 | -0.0380 | 7 |

**Table E3.** Times of negative-superhump maxima in KIC 9406652 during time interval 3 (BJD 2455643–2455871) (continued).

| $E^*$ | Max$^\dagger$ | Error | $O-C^\ddagger$ | $N^\S$ |
|---|---|---|---|---|
| 872 | 852.3793 | 0.0059 | -0.0284 | 10 |
| 873 | 852.6166 | 0.0030 | -0.0310 | 10 |
| 874 | 852.8594 | 0.0031 | -0.0281 | 9 |
| 875 | 853.0816 | 0.0024 | -0.0458 | 9 |
| 876 | 853.3106 | 0.0068 | -0.0566 | 10 |
| 877 | 853.5592 | 0.0040 | -0.0479 | 10 |
| 878 | 853.7974 | 0.0110 | -0.0496 | 9 |
| 879 | 854.0419 | 0.0056 | -0.0450 | 8 |
| 880 | 854.2844 | 0.0110 | -0.0424 | 9 |
| 881 | 854.5190 | 0.0067 | -0.0477 | 10 |
| 883 | 854.9990 | 0.0057 | -0.0474 | 9 |
| 885 | 855.4863 | 0.0091 | -0.0398 | 9 |
| 886 | 855.7135 | 0.0088 | -0.0525 | 9 |
| 887 | 855.9709 | 0.0067 | -0.0351 | 9 |
| 888 | 856.2126 | 0.0086 | -0.0332 | 10 |
| 890 | 856.6785 | 0.0155 | -0.0471 | 9 |
| 892 | 857.1641 | 0.0073 | -0.0412 | 9 |
| 893 | 857.4171 | 0.0119 | -0.0281 | 9 |
| 894 | 857.6334 | 0.0063 | -0.0517 | 9 |
| 895 | 857.8909 | 0.0077 | -0.0341 | 9 |
| 896 | 858.1247 | 0.0028 | -0.0402 | 10 |
| 900 | 859.1221 | 0.0065 | -0.0023 | 10 |
| 901 | 859.3215 | 0.0070 | -0.0427 | 9 |
| 903 | 859.7956 | 0.0116 | -0.0484 | 10 |
| 904 | 860.0493 | 0.0087 | -0.0346 | 9 |
| 907 | 860.7580 | 0.0084 | -0.0455 | 10 |
| 908 | 860.9999 | 0.0118 | -0.0435 | 9 |
| 911 | 861.7193 | 0.0075 | -0.0437 | 10 |
| 912 | 861.9687 | 0.0061 | -0.0342 | 9 |
| 913 | 862.2161 | 0.0029 | -0.0267 | 9 |
| 914 | 862.4546 | 0.0045 | -0.0281 | 9 |
| 915 | 862.7076 | 0.0040 | -0.0150 | 10 |
| 916 | 862.9537 | 0.0046 | -0.0088 | 9 |
| 918 | 863.4116 | 0.0067 | -0.0306 | 9 |
| 919 | 863.6688 | 0.0049 | -0.0133 | 10 |
| 920 | 863.8877 | 0.0049 | -0.0343 | 9 |
| 921 | 864.1264 | 0.0100 | -0.0354 | 9 |
| 923 | 864.6114 | 0.0026 | -0.0302 | 10 |
| 924 | 864.8581 | 0.0045 | -0.0234 | 9 |
| 925 | 865.0981 | 0.0038 | -0.0232 | 9 |
| 929 | 866.0644 | 0.0031 | -0.0165 | 6 |
| 930 | 866.2901 | 0.0017 | -0.0306 | 10 |
| 931 | 866.5356 | 0.0013 | -0.0250 | 10 |
| 932 | 866.7739 | 0.0025 | -0.0267 | 9 |
| 933 | 867.0038 | 0.0052 | -0.0366 | 9 |
| 934 | 867.2502 | 0.0020 | -0.0301 | 10 |
| 935 | 867.4903 | 0.0039 | -0.0298 | 9 |
| 936 | 867.7293 | 0.0035 | -0.0307 | 9 |
| 937 | 867.9731 | 0.0025 | -0.0268 | 9 |
| 938 | 868.2215 | 0.0023 | -0.0183 | 9 |
| 939 | 868.4644 | 0.0019 | -0.0153 | 9 |
| 940 | 868.7086 | 0.0023 | -0.0110 | 9 |

**Table E3.** Times of negative-superhump maxima in KIC 9406652 during time interval 3 (BJD 2455643–2455871) (continued).

| $E^*$ | Max$^\dagger$ | Error | $O-C^\ddagger$ | $N^\S$ |
|---|---|---|---|---|
| 941 | 868.9750 | 0.0062 | 0.0155 | 9 |
| 942 | 869.1842 | 0.0016 | -0.0151 | 10 |
| 943 | 869.4629 | 0.0023 | 0.0237 | 9 |
| 944 | 869.6957 | 0.0022 | 0.0166 | 9 |
| 945 | 869.8923 | 0.0053 | -0.0267 | 10 |
| 946 | 870.1577 | 0.0025 | -0.0011 | 10 |
| 947 | 870.3962 | 0.0023 | -0.0025 | 9 |
| 948 | 870.6301 | 0.0048 | -0.0085 | 8 |
| 949 | 870.8708 | 0.0013 | -0.0077 | 10 |

$^*$Cycle counts.

$^\dagger$BJD−2455000.0.

$^\ddagger$ C = 2455643.2055+0.23988 E.

$^\S$Number of points used for determining the maximum.
