# Supplementary material for: KIC 9406652: A laboratory of the tilted disk in cataclysmic variable stars
Source: arXiv:2008.11328 ancillary file (2020-08-27)
Supplement: Supplementary file 2 [file si-kic940-2.pdf]

**Table E4.** Times of negative-superhump maxima in KIC 9406652 during time interval 4 (BJD 2455871–2456058).

| $E^*$ | Max <sup>†</sup> | Error  | $O - C^\ddagger$ | $N^\S$ |
|-------|------------------|--------|------------------|--------|
| 0     | 871.1184         | 0.0020 | 0.0092           | 9      |
| 1     | 871.3548         | 0.0050 | 0.0058           | 5      |
| 2     | 871.5990         | 0.0014 | 0.0103           | 10     |
| 3     | 871.8444         | 0.0053 | 0.0159           | 9      |
| 4     | 872.0645         | 0.0034 | -0.0038          | 9      |
| 5     | 872.3069         | 0.0027 | -0.0011          | 10     |
| 6     | 872.5343         | 0.0028 | -0.0134          | 10     |
| 7     | 872.7864         | 0.0034 | -0.0011          | 9      |
| 8     | 873.0195         | 0.0021 | -0.0078          | 9      |
| 9     | 873.2671         | 0.0023 | 0.0001           | 10     |
| 10    | 873.5080         | 0.0025 | 0.0012           | 9      |
| 11    | 873.7484         | 0.0014 | 0.0019           | 9      |
| 12    | 873.9883         | 0.0021 | 0.0020           | 9      |
| 13    | 874.2226         | 0.0026 | -0.0034          | 8      |
| 14    | 874.4651         | 0.0016 | -0.0007          | 9      |
| 15    | 874.7057         | 0.0021 | 0.0002           | 9      |
| 16    | 874.9542         | 0.0032 | 0.0089           | 10     |
| 17    | 875.1845         | 0.0021 | -0.0005          | 10     |
| 18    | 875.4270         | 0.0029 | 0.0023           | 9      |
| 19    | 875.6627         | 0.0033 | -0.0018          | 9      |
| 20    | 875.9013         | 0.0028 | -0.0029          | 10     |
| 21    | 876.1391         | 0.0017 | -0.0049          | 10     |
| 22    | 876.3747         | 0.0019 | -0.0091          | 9      |
| 23    | 876.6173         | 0.0028 | -0.0062          | 9      |
| 24    | 876.8632         | 0.0016 | -0.0001          | 10     |
| 25    | 877.1043         | 0.0022 | 0.0013           | 9      |
| 26    | 877.3453         | 0.0016 | 0.0025           | 9      |
| 27    | 877.5823         | 0.0017 | -0.0002          | 9      |
| 28    | 877.8222         | 0.0023 | -0.0000          | 10     |
| 29    | 878.0644         | 0.0017 | 0.0024           | 9      |
| 30    | 878.2989         | 0.0014 | -0.0029          | 9      |
| 31    | 878.5420         | 0.0021 | 0.0005           | 10     |
| 32    | 878.7778         | 0.0025 | -0.0034          | 10     |
| 33    | 879.0249         | 0.0027 | 0.0039           | 9      |
| 34    | 879.2680         | 0.0040 | 0.0072           | 9      |
| 35    | 879.4979         | 0.0041 | -0.0026          | 10     |
| 36    | 879.7385         | 0.0040 | -0.0018          | 10     |
| 37    | 879.9753         | 0.0043 | -0.0047          | 9      |
| 38    | 880.2152         | 0.0040 | -0.0045          | 8      |
| 39    | 880.4448         | 0.0021 | -0.0147          | 10     |
| 40    | 880.6826         | 0.0024 | -0.0167          | 9      |
| 41    | 880.9289         | 0.0040 | -0.0101          | 9      |
| 42    | 881.1741         | 0.0027 | -0.0047          | 9      |
| 43    | 881.4097         | 0.0014 | -0.0088          | 10     |
| 44    | 881.6562         | 0.0022 | -0.0020          | 9      |
| 45    | 881.8862         | 0.0025 | -0.0118          | 9      |
| 46    | 882.1381         | 0.0032 | 0.0004           | 10     |
| 47    | 882.3718         | 0.0031 | -0.0057          | 10     |
| 48    | 882.6166         | 0.0037 | -0.0007          | 9      |
| 49    | 882.8527         | 0.0022 | -0.0043          | 9      |
| 50    | 883.0911         | 0.0019 | -0.0057          | 10     |
| 51    | 883.3344         | 0.0030 | -0.0021          | 10     |

**Table E4.** Times of negative-superhump maxima in KIC 9406652 during time interval 4 (BJD 2455871–2456058) (continued).

| $E^*$ | Max <sup>†</sup> | Error  | $O - C^\ddagger$ | $N^\S$ |
|-------|------------------|--------|------------------|--------|
| 52    | 883.5654         | 0.0035 | -0.0109          | 9      |
| 53    | 883.7925         | 0.0047 | -0.0235          | 9      |
| 54    | 884.0395         | 0.0043 | -0.0162          | 10     |
| 55    | 884.2788         | 0.0038 | -0.0167          | 9      |
| 56    | 884.5123         | 0.0032 | -0.0229          | 9      |
| 57    | 884.7548         | 0.0012 | -0.0202          | 9      |
| 58    | 884.9963         | 0.0022 | -0.0185          | 10     |
| 59    | 885.2382         | 0.0038 | -0.0163          | 9      |
| 60    | 885.4775         | 0.0022 | -0.0168          | 9      |
| 61    | 885.7157         | 0.0021 | -0.0183          | 9      |
| 62    | 885.9628         | 0.0021 | -0.0109          | 10     |
| 63    | 886.2139         | 0.0030 | 0.0004           | 8      |
| 64    | 886.4430         | 0.0040 | -0.0102          | 9      |
| 65    | 886.6846         | 0.0037 | -0.0084          | 10     |
| 66    | 886.9038         | 0.0059 | -0.0289          | 10     |
| 67    | 887.1544         | 0.0066 | -0.0181          | 9      |
| 68    | 887.3860         | 0.0034 | -0.0262          | 9      |
| 69    | 887.6189         | 0.0081 | -0.0331          | 10     |
| 70    | 887.8467         | 0.0050 | -0.0451          | 9      |
| 71    | 888.0988         | 0.0078 | -0.0327          | 9      |
| 72    | 888.3338         | 0.0043 | -0.0374          | 9      |
| 73    | 888.5702         | 0.0035 | -0.0408          | 10     |
| 74    | 888.8159         | 0.0027 | -0.0348          | 9      |
| 75    | 889.0592         | 0.0085 | -0.0313          | 7      |
| 76    | 889.2954         | 0.0041 | -0.0349          | 9      |
| 77    | 889.5445         | 0.0039 | -0.0255          | 10     |
| 78    | 889.8002         | 0.0018 | -0.0095          | 9      |
| 80    | 890.2777         | 0.0050 | -0.0115          | 10     |
| 82    | 890.7439         | 0.0041 | -0.0248          | 9      |
| 83    | 890.9890         | 0.0130 | -0.0195          | 9      |
| 84    | 891.2276         | 0.0046 | -0.0207          | 10     |
| 85    | 891.4731         | 0.0136 | -0.0149          | 9      |
| 86    | 891.7038         | 0.0091 | -0.0239          | 9      |
| 87    | 891.9826         | 0.0056 | 0.0151           | 9      |
| 88    | 892.1882         | 0.0107 | -0.0190          | 9      |
| 89    | 892.4281         | 0.0098 | -0.0189          | 9      |
| 91    | 892.9110         | 0.0061 | -0.0155          | 9      |
| 94    | 893.6342         | 0.0079 | -0.0116          | 9      |
| 95    | 893.8527         | 0.0086 | -0.0328          | 10     |
| 98    | 894.5690         | 0.0039 | -0.0357          | 9      |
| 99    | 894.8258         | 0.0052 | -0.0187          | 10     |
| 101   | 895.3133         | 0.0010 | -0.0107          | 9      |
| 102   | 895.5578         | 0.0031 | -0.0060          | 9      |
| 103   | 895.8126         | 0.0035 | 0.0091           | 10     |
| 104   | 896.0551         | 0.0032 | 0.0118           | 9      |
| 112   | 897.9326         | 0.0080 | -0.0286          | 9      |
| 113   | 898.1861         | 0.0053 | -0.0149          | 9      |
| 114   | 898.4302         | 0.0036 | -0.0105          | 10     |
| 115   | 898.6731         | 0.0028 | -0.0074          | 10     |
| 116   | 898.9059         | 0.0063 | -0.0143          | 9      |
| 117   | 899.1423         | 0.0021 | -0.0177          | 8      |
| 118   | 899.3930         | 0.0017 | -0.0068          | 10     |

**Table E4.** Times of negative-superhump maxima in KIC 9406652 during time interval 4 (BJD 2455871–2456058) (continued).

| $E^*$ | Max <sup>†</sup> | Error  | $O - C^\ddagger$ | $N^\S$ |
|-------|------------------|--------|------------------|--------|
| 119   | 899.6435         | 0.0018 | 0.0040           | 9      |
| 120   | 899.8791         | 0.0024 | -0.0001          | 9      |
| 121   | 900.1236         | 0.0011 | 0.0046           | 9      |
| 122   | 900.3687         | 0.0026 | 0.0099           | 10     |
| 123   | 900.6005         | 0.0025 | 0.0020           | 9      |
| 124   | 900.8450         | 0.0015 | 0.0067           | 9      |
| 125   | 901.0762         | 0.0044 | -0.0018          | 10     |
| 126   | 901.3172         | 0.0018 | -0.0006          | 10     |
| 127   | 901.5673         | 0.0040 | 0.0098           | 9      |
| 128   | 901.7985         | 0.0028 | 0.0012           | 9      |
| 129   | 902.0456         | 0.0015 | 0.0086           | 10     |
| 130   | 902.2894         | 0.0011 | 0.0126           | 9      |
| 131   | 902.5311         | 0.0014 | 0.0146           | 9      |
| 132   | 902.7656         | 0.0024 | 0.0094           | 9      |
| 133   | 903.0110         | 0.0012 | 0.0150           | 5      |
| 144   | 905.6523         | 0.0029 | 0.0190           | 8      |
| 145   | 905.8805         | 0.0021 | 0.0075           | 10     |
| 146   | 906.1209         | 0.0027 | 0.0082           | 9      |
| 147   | 906.3564         | 0.0017 | 0.0039           | 9      |
| 148   | 906.6016         | 0.0019 | 0.0093           | 10     |
| 149   | 906.8428         | 0.0040 | 0.0108           | 9      |
| 150   | 907.0783         | 0.0040 | 0.0066           | 9      |
| 151   | 907.3223         | 0.0014 | 0.0108           | 9      |
| 152   | 907.5595         | 0.0018 | 0.0082           | 10     |
| 153   | 907.7990         | 0.0017 | 0.0080           | 9      |
| 154   | 908.0417         | 0.0018 | 0.0110           | 9      |
| 155   | 908.2845         | 0.0020 | 0.0140           | 10     |
| 156   | 908.5277         | 0.0012 | 0.0174           | 10     |
| 157   | 908.7674         | 0.0008 | 0.0174           | 8      |
| 158   | 909.0117         | 0.0023 | 0.0219           | 5      |
| 159   | 909.2434         | 0.0011 | 0.0139           | 10     |
| 160   | 909.4785         | 0.0017 | 0.0092           | 10     |
| 161   | 909.7189         | 0.0022 | 0.0099           | 9      |
| 162   | 909.9607         | 0.0024 | 0.0119           | 9      |
| 163   | 910.2061         | 0.0017 | 0.0176           | 10     |
| 164   | 910.4386         | 0.0017 | 0.0104           | 9      |
| 165   | 910.6769         | 0.0020 | 0.0089           | 9      |
| 166   | 910.9187         | 0.0020 | 0.0109           | 9      |
| 167   | 911.1492         | 0.0033 | 0.0017           | 10     |
| 168   | 911.3883         | 0.0040 | 0.0011           | 9      |
| 169   | 911.6302         | 0.0041 | 0.0032           | 8      |
| 170   | 911.8671         | 0.0032 | 0.0003           | 10     |
| 171   | 912.1154         | 0.0017 | 0.0089           | 10     |
| 172   | 912.3558         | 0.0016 | 0.0095           | 9      |
| 173   | 912.5976         | 0.0013 | 0.0116           | 9      |
| 174   | 912.8458         | 0.0018 | 0.0201           | 10     |
| 175   | 913.0798         | 0.0046 | 0.0143           | 10     |
| 176   | 913.3263         | 0.0017 | 0.0210           | 9      |
| 177   | 913.5694         | 0.0022 | 0.0244           | 9      |
| 178   | 913.7993         | 0.0026 | 0.0145           | 10     |
| 179   | 914.0421         | 0.0024 | 0.0176           | 9      |
| 180   | 914.2771         | 0.0019 | 0.0128           | 9      |

**Table E4.** Times of negative-superhump maxima in KIC 9406652 during time interval 4 (BJD 2455871–2456058) (continued).

| $E^*$ | Max <sup>†</sup> | Error  | $O - C^\ddagger$ | $N^\S$ |
|-------|------------------|--------|------------------|--------|
| 181   | 914.5145         | 0.0018 | 0.0105           | 9      |
| 182   | 914.7606         | 0.0014 | 0.0168           | 9      |
| 183   | 914.9957         | 0.0029 | 0.0122           | 9      |
| 184   | 915.2269         | 0.0023 | 0.0036           | 9      |
| 185   | 915.4684         | 0.0045 | 0.0054           | 10     |
| 186   | 915.7134         | 0.0019 | 0.0106           | 10     |
| 187   | 915.9429         | 0.0027 | 0.0004           | 8      |
| 188   | 916.1876         | 0.0016 | 0.0053           | 9      |
| 189   | 916.4371         | 0.0014 | 0.0151           | 10     |
| 190   | 916.6748         | 0.0026 | 0.0130           | 10     |
| 191   | 916.9134         | 0.0024 | 0.0119           | 9      |
| 192   | 917.1569         | 0.0018 | 0.0156           | 9      |
| 193   | 917.3964         | 0.0019 | 0.0154           | 10     |
| 194   | 917.6343         | 0.0029 | 0.0136           | 8      |
| 195   | 917.8661         | 0.0017 | 0.0056           | 9      |
| 196   | 918.1058         | 0.0021 | 0.0056           | 9      |
| 197   | 918.3503         | 0.0025 | 0.0103           | 10     |
| 200   | 919.0534         | 0.0045 | -0.0058          | 10     |
| 201   | 919.2937         | 0.0016 | -0.0053          | 10     |
| 202   | 919.5327         | 0.0015 | -0.0061          | 9      |
| 203   | 919.7704         | 0.0006 | -0.0081          | 9      |
| 204   | 920.0201         | 0.0022 | 0.0018           | 10     |
| 205   | 920.2485         | 0.0006 | -0.0095          | 10     |
| 206   | 920.4945         | 0.0011 | -0.0032          | 9      |
| 207   | 920.7346         | 0.0027 | -0.0029          | 9      |
| 208   | 920.9832         | 0.0018 | 0.0060           | 10     |
| 209   | 921.2230         | 0.0017 | 0.0060           | 9      |
| 210   | 921.4581         | 0.0017 | 0.0013           | 9      |
| 211   | 921.7057         | 0.0018 | 0.0092           | 9      |
| 212   | 921.9325         | 0.0024 | -0.0038          | 10     |
| 213   | 922.1800         | 0.0009 | 0.0040           | 9      |
| 214   | 922.4119         | 0.0028 | -0.0039          | 8      |
| 215   | 922.6532         | 0.0031 | -0.0023          | 10     |
| 216   | 922.8772         | 0.0032 | -0.0180          | 10     |
| 217   | 923.1288         | 0.0024 | -0.0062          | 9      |
| 218   | 923.3657         | 0.0031 | -0.0090          | 9      |
| 219   | 923.6077         | 0.0029 | -0.0068          | 9      |
| 220   | 923.8465         | 0.0035 | -0.0078          | 10     |
| 221   | 924.0805         | 0.0056 | -0.0135          | 9      |
| 222   | 924.3262         | 0.0048 | -0.0075          | 9      |
| 223   | 924.5662         | 0.0039 | -0.0073          | 10     |
| 224   | 924.8022         | 0.0068 | -0.0110          | 9      |
| 225   | 925.0394         | 0.0057 | -0.0136          | 9      |
| 226   | 925.2950         | 0.0051 | 0.0022           | 9      |
| 227   | 925.5310         | 0.0042 | -0.0015          | 10     |
| 228   | 925.7644         | 0.0027 | -0.0078          | 9      |
| 229   | 926.0265         | 0.0038 | 0.0145           | 9      |
| 230   | 926.2377         | 0.0047 | -0.0140          | 10     |
| 231   | 926.4903         | 0.0032 | -0.0012          | 10     |
| 232   | 926.7451         | 0.0039 | 0.0139           | 8      |
| 233   | 926.9772         | 0.0092 | 0.0062           | 9      |
| 234   | 927.1998         | 0.0062 | -0.0110          | 10     |

**Table E4.** Times of negative-superhump maxima in KIC 9406652 during time interval 4 (BJD 2455871–2456058) (continued).

| $E^*$ | Max <sup>†</sup> | Error  | $O - C^\ddagger$ | $N^\S$ |
|-------|------------------|--------|------------------|--------|
| 235   | 927.4265         | 0.0057 | -0.0240          | 10     |
| 236   | 927.6790         | 0.0040 | -0.0112          | 9      |
| 237   | 927.9115         | 0.0054 | -0.0185          | 9      |
| 238   | 928.1438         | 0.0047 | -0.0260          | 10     |
| 239   | 928.3915         | 0.0014 | -0.0180          | 9      |
| 240   | 928.6547         | 0.0067 | 0.0055           | 9      |
| 241   | 928.8808         | 0.0034 | -0.0082          | 9      |
| 242   | 929.1405         | 0.0033 | 0.0118           | 10     |
| 243   | 929.3768         | 0.0043 | 0.0083           | 7      |
| 244   | 929.6296         | 0.0053 | 0.0213           | 7      |
| 245   | 929.8240         | 0.0084 | -0.0240          | 8      |
| 258   | 932.9150         | 0.0103 | -0.0498          | 9      |
| 259   | 933.1712         | 0.0108 | -0.0333          | 9      |
| 260   | 933.4171         | 0.0089 | -0.0272          | 10     |
| 261   | 933.6439         | 0.0055 | -0.0401          | 10     |
| 262   | 933.8923         | 0.0120 | -0.0315          | 9      |
| 263   | 934.1277         | 0.0084 | -0.0358          | 9      |
| 264   | 934.3968         | 0.0035 | -0.0064          | 9      |
| 265   | 934.6293         | 0.0060 | -0.0137          | 10     |
| 266   | 934.8755         | 0.0063 | -0.0072          | 9      |
| 267   | 935.1097         | 0.0065 | -0.0128          | 9      |
| 268   | 935.3530         | 0.0066 | -0.0092          | 10     |
| 269   | 935.6005         | 0.0120 | -0.0015          | 9      |
| 270   | 935.8609         | 0.0142 | 0.0192           | 9      |
| 271   | 936.0666         | 0.0075 | -0.0149          | 9      |
| 272   | 936.3276         | 0.0040 | 0.0064           | 10     |
| 273   | 936.5739         | 0.0052 | 0.0129           | 9      |
| 274   | 936.8165         | 0.0029 | 0.0158           | 9      |
| 275   | 937.0406         | 0.0079 | 0.0001           | 10     |
| 276   | 937.2908         | 0.0013 | 0.0105           | 8      |
| 277   | 937.5283         | 0.0030 | 0.0083           | 9      |
| 278   | 937.7754         | 0.0034 | 0.0157           | 9      |
| 279   | 938.0207         | 0.0044 | 0.0212           | 10     |
| 280   | 938.2541         | 0.0029 | 0.0149           | 10     |
| 281   | 938.4968         | 0.0033 | 0.0179           | 9      |
| 282   | 938.7341         | 0.0035 | 0.0154           | 9      |
| 283   | 938.9803         | 0.0024 | 0.0218           | 10     |
| 284   | 939.2186         | 0.0027 | 0.0203           | 9      |
| 285   | 939.4609         | 0.0031 | 0.0229           | 9      |
| 286   | 939.7013         | 0.0022 | 0.0235           | 9      |
| 287   | 939.9396         | 0.0018 | 0.0221           | 10     |
| 288   | 940.1854         | 0.0014 | 0.0282           | 9      |
| 289   | 940.4234         | 0.0025 | 0.0264           | 8      |
| 290   | 940.6655         | 0.0028 | 0.0288           | 10     |
| 291   | 940.9032         | 0.0060 | 0.0267           | 10     |
| 292   | 941.1392         | 0.0052 | 0.0230           | 9      |
| 293   | 941.3679         | 0.0046 | 0.0119           | 9      |
| 294   | 941.5953         | 0.0087 | -0.0005          | 10     |
| 295   | 941.8401         | 0.0032 | 0.0046           | 10     |
| 296   | 942.0820         | 0.0043 | 0.0068           | 8      |
| 297   | 942.3152         | 0.0038 | 0.0002           | 9      |
| 298   | 942.5576         | 0.0068 | 0.0029           | 10     |

**Table E4.** Times of negative-superhump maxima in KIC 9406652 during time interval 4 (BJD 2455871–2456058) (continued).

| $E^*$ | Max <sup>†</sup> | Error  | $O - C^\ddagger$ | $N^\S$ |
|-------|------------------|--------|------------------|--------|
| 299   | 942.7997         | 0.0047 | 0.0052           | 9      |
| 300   | 943.0573         | 0.0073 | 0.0231           | 9      |
| 301   | 943.2807         | 0.0076 | 0.0067           | 6      |
| 302   | 943.5276         | 0.0034 | 0.0138           | 10     |
| 303   | 943.7666         | 0.0056 | 0.0131           | 9      |
| 304   | 944.0224         | 0.0109 | 0.0292           | 9      |
| 305   | 944.2450         | 0.0074 | 0.0120           | 10     |
| 306   | 944.4866         | 0.0061 | 0.0138           | 10     |
| 307   | 944.7257         | 0.0062 | 0.0132           | 9      |
| 308   | 944.9801         | 0.0020 | 0.0279           | 9      |
| 309   | 945.2065         | 0.0022 | 0.0145           | 10     |
| 310   | 945.4516         | 0.0053 | 0.0198           | 10     |
| 311   | 945.6757         | 0.0042 | 0.0042           | 9      |
| 312   | 945.9187         | 0.0021 | 0.0075           | 9      |
| 313   | 946.1747         | 0.0030 | 0.0237           | 9      |
| 314   | 946.4036         | 0.0066 | 0.0128           | 9      |
| 315   | 946.6474         | 0.0035 | 0.0169           | 9      |
| 316   | 946.8842         | 0.0050 | 0.0139           | 9      |
| 317   | 947.1237         | 0.0020 | 0.0137           | 10     |
| 318   | 947.3617         | 0.0044 | 0.0119           | 9      |
| 319   | 947.5993         | 0.0045 | 0.0098           | 9      |
| 320   | 947.8372         | 0.0028 | 0.0080           | 10     |
| 321   | 948.0869         | 0.0025 | 0.0179           | 10     |
| 322   | 948.3229         | 0.0021 | 0.0142           | 9      |
| 323   | 948.5767         | 0.0040 | 0.0282           | 9      |
| 324   | 948.7965         | 0.0045 | 0.0083           | 10     |
| 326   | 949.2689         | 0.0108 | 0.0011           | 8      |
| 327   | 949.5070         | 0.0104 | -0.0005          | 9      |
| 337   | 951.9097         | 0.0041 | 0.0047           | 8      |
| 338   | 952.1423         | 0.0039 | -0.0024          | 9      |
| 339   | 952.3910         | 0.0034 | 0.0065           | 10     |
| 340   | 952.6251         | 0.0035 | 0.0008           | 10     |
| 341   | 952.8693         | 0.0040 | 0.0053           | 9      |
| 342   | 953.0947         | 0.0051 | -0.0090          | 9      |
| 343   | 953.3433         | 0.0059 | -0.0002          | 10     |
| 344   | 953.5842         | 0.0083 | 0.0010           | 9      |
| 345   | 953.8065         | 0.0078 | -0.0165          | 9      |
| 346   | 954.0533         | 0.0062 | -0.0094          | 9      |
| 351   | 955.2633         | 0.0124 | 0.0018           | 6      |
| 352   | 955.4919         | 0.0024 | -0.0094          | 9      |
| 353   | 955.7282         | 0.0017 | -0.0128          | 9      |
| 354   | 955.9697         | 0.0030 | -0.0111          | 10     |
| 355   | 956.2152         | 0.0023 | -0.0053          | 10     |
| 356   | 956.4566         | 0.0045 | -0.0036          | 8      |
| 357   | 956.6894         | 0.0047 | -0.0106          | 9      |
| 358   | 956.9362         | 0.0093 | -0.0036          | 10     |
| 359   | 957.1518         | 0.0072 | -0.0277          | 9      |
| 360   | 957.4027         | 0.0122 | -0.0166          | 9      |
| 361   | 957.6225         | 0.0033 | -0.0365          | 9      |
| 362   | 957.8716         | 0.0060 | -0.0271          | 10     |
| 363   | 958.1072         | 0.0132 | -0.0313          | 8      |
| 364   | 958.3381         | 0.0067 | -0.0401          | 9      |

**Table E4.** Times of negative-superhump maxima in KIC 9406652 during time interval 4 (BJD 2455871–2456058) (continued).

| $E^*$ | Max <sup>†</sup> | Error  | $O - C^{\ddagger}$ | $N^{\S}$ |
|-------|------------------|--------|--------------------|----------|
| 365   | 958.5840         | 0.0036 | -0.0340            | 10       |
| 366   | 958.8326         | 0.0087 | -0.0251            | 7        |
| 370   | 959.7902         | 0.0031 | -0.0266            | 10       |
| 371   | 960.0364         | 0.0046 | -0.0201            | 9        |
| 372   | 960.2836         | 0.0035 | -0.0126            | 9        |
| 373   | 960.5217         | 0.0050 | -0.0143            | 10       |
| 374   | 960.7671         | 0.0072 | -0.0086            | 9        |
| 375   | 961.0196         | 0.0058 | 0.0041             | 9        |
| 376   | 961.2540         | 0.0073 | -0.0012            | 9        |
| 377   | 961.4855         | 0.0067 | -0.0095            | 10       |
| 378   | 961.6957         | 0.0135 | -0.0390            | 9        |
| 379   | 961.9533         | 0.0173 | -0.0212            | 8        |
| 380   | 962.1614         | 0.0064 | -0.0528            | 10       |
| 381   | 962.4145         | 0.0024 | -0.0395            | 10       |
| 382   | 962.6536         | 0.0036 | -0.0401            | 9        |
| 383   | 962.8984         | 0.0087 | -0.0351            | 9        |
| 384   | 963.1338         | 0.0033 | -0.0394            | 9        |
| 385   | 963.3811         | 0.0050 | -0.0319            | 10       |
| 386   | 963.6429         | 0.0027 | -0.0098            | 9        |
| 387   | 963.8593         | 0.0058 | -0.0332            | 9        |
| 388   | 964.1222         | 0.0058 | -0.0101            | 10       |
| 389   | 964.3410         | 0.0122 | -0.0310            | 9        |
| 390   | 964.6332         | 0.0062 | 0.0215             | 9        |
| 398   | 966.5502         | 0.0036 | 0.0204             | 9        |
| 399   | 966.7503         | 0.0138 | -0.0192            | 10       |
| 415   | 970.5541         | 0.0098 | -0.0514            | 10       |
| 416   | 970.8231         | 0.0095 | -0.0222            | 8        |
| 418   | 971.2876         | 0.0083 | -0.0372            | 10       |
| 419   | 971.5194         | 0.0025 | -0.0451            | 9        |
| 420   | 971.7810         | 0.0048 | -0.0233            | 9        |
| 421   | 972.0231         | 0.0061 | -0.0209            | 9        |
| 422   | 972.2787         | 0.0096 | -0.0051            | 10       |
| 423   | 972.5195         | 0.0034 | -0.0040            | 9        |
| 424   | 972.7532         | 0.0075 | -0.0100            | 9        |
| 425   | 973.0026         | 0.0114 | -0.0004            | 10       |
| 426   | 973.2405         | 0.0026 | -0.0022            | 10       |
| 427   | 973.4808         | 0.0139 | -0.0017            | 9        |
| 429   | 973.9263         | 0.0102 | -0.0357            | 10       |
| 431   | 974.4047         | 0.0056 | -0.0368            | 9        |
| 432   | 974.6581         | 0.0098 | -0.0232            | 9        |
| 433   | 974.9075         | 0.0045 | -0.0135            | 10       |
| 434   | 975.1454         | 0.0051 | -0.0154            | 9        |
| 435   | 975.3994         | 0.0037 | -0.0011            | 9        |
| 436   | 975.6511         | 0.0041 | 0.0108             | 9        |
| 437   | 975.8775         | 0.0045 | -0.0025            | 10       |
| 438   | 976.1255         | 0.0039 | 0.0058             | 9        |
| 439   | 976.3648         | 0.0039 | 0.0053             | 9        |
| 440   | 976.6056         | 0.0014 | 0.0064             | 10       |
| 441   | 976.8533         | 0.0028 | 0.0143             | 9        |
| 442   | 977.0998         | 0.0040 | 0.0210             | 9        |
| 443   | 977.3356         | 0.0026 | 0.0171             | 9        |
| 444   | 977.5762         | 0.0028 | 0.0179             | 10       |

**Table E4.** Times of negative-superhump maxima in KIC 9406652 during time interval 4 (BJD 2455871–2456058) (continued).

| $E^*$ | Max <sup>†</sup> | Error  | $O - C^{\ddagger}$ | $N^{\S}$ |
|-------|------------------|--------|--------------------|----------|
| 445   | 977.8164         | 0.0016 | 0.0184             | 10       |
| 446   | 978.0492         | 0.0023 | 0.0115             | 9        |
| 447   | 978.2844         | 0.0022 | 0.0069             | 9        |
| 448   | 978.5272         | 0.0021 | 0.0099             | 10       |
| 449   | 978.7548         | 0.0019 | -0.0022            | 9        |
| 450   | 978.9965         | 0.0020 | -0.0003            | 9        |
| 451   | 979.2375         | 0.0025 | 0.0010             | 9        |
| 452   | 979.4807         | 0.0022 | 0.0044             | 10       |
| 453   | 979.7198         | 0.0025 | 0.0038             | 9        |
| 454   | 979.9507         | 0.0051 | -0.0051            | 7        |
| 455   | 980.2005         | 0.0022 | 0.0050             | 10       |
| 456   | 980.4336         | 0.0021 | -0.0017            | 10       |
| 457   | 980.6696         | 0.0031 | -0.0054            | 9        |
| 458   | 980.9091         | 0.0015 | -0.0057            | 9        |
| 459   | 981.1601         | 0.0010 | 0.0056             | 10       |
| 460   | 981.3995         | 0.0040 | 0.0052             | 10       |
| 461   | 981.6404         | 0.0053 | 0.0064             | 9        |
| 462   | 981.8650         | 0.0049 | -0.0087            | 9        |
| 463   | 982.1116         | 0.0047 | -0.0019            | 10       |
| 464   | 982.3550         | 0.0092 | 0.0018             | 9        |
| 465   | 982.5828         | 0.0062 | -0.0102            | 9        |
| 466   | 982.8257         | 0.0085 | -0.0070            | 8        |
| 467   | 983.0703         | 0.0096 | -0.0022            | 10       |
| 468   | 983.2869         | 0.0072 | -0.0253            | 9        |
| 469   | 983.5511         | 0.0028 | -0.0009            | 9        |
| 470   | 983.7812         | 0.0035 | -0.0105            | 10       |
| 471   | 984.0234         | 0.0033 | -0.0081            | 10       |
| 472   | 984.2695         | 0.0019 | -0.0018            | 9        |
| 473   | 984.5125         | 0.0022 | 0.0015             | 9        |
| 474   | 984.7558         | 0.0030 | 0.0051             | 10       |
| 475   | 985.0061         | 0.0046 | 0.0156             | 10       |
| 476   | 985.2476         | 0.0021 | 0.0173             | 9        |
| 477   | 985.4870         | 0.0034 | 0.0170             | 9        |
| 478   | 985.7305         | 0.0056 | 0.0207             | 9        |
| 479   | 985.9652         | 0.0050 | 0.0157             | 9        |
| 480   | 986.2049         | 0.0038 | 0.0156             | 9        |
| 481   | 986.4460         | 0.0039 | 0.0170             | 9        |
| 482   | 986.6814         | 0.0047 | 0.0126             | 10       |
| 483   | 986.8894         | 0.0066 | -0.0191            | 9        |
| 488   | 988.1027         | 0.0029 | -0.0045            | 9        |
| 489   | 988.3319         | 0.0033 | -0.0151            | 10       |
| 490   | 988.5780         | 0.0024 | -0.0088            | 10       |
| 491   | 988.8213         | 0.0018 | -0.0052            | 9        |
| 492   | 989.0615         | 0.0114 | -0.0047            | 9        |
| 493   | 989.2996         | 0.0042 | -0.0064            | 10       |
| 494   | 989.5280         | 0.0155 | -0.0178            | 9        |
| 495   | 989.7768         | 0.0024 | -0.0087            | 9        |
| 496   | 990.0170         | 0.0042 | -0.0082            | 8        |
| 497   | 990.2717         | 0.0085 | 0.0067             | 10       |
| 498   | 990.4819         | 0.0137 | -0.0229            | 9        |
| 499   | 990.7115         | 0.0113 | -0.0330            | 9        |
| 500   | 990.9554         | 0.0119 | -0.0289            | 10       |

**Table E4.** Times of negative-superhump maxima in KIC 9406652 during time interval 4 (BJD 2455871–2456058) (continued).

| $E^*$ | Max <sup>†</sup> | Error  | $O - C^{\ddagger}$ | $N^{\S}$ |
|-------|------------------|--------|--------------------|----------|
| 501   | 991.2003         | 0.0124 | -0.0237            | 10       |
| 502   | 991.4395         | 0.0172 | -0.0242            | 9        |
| 503   | 991.6780         | 0.0102 | -0.0255            | 9        |
| 504   | 991.9264         | 0.0060 | -0.0169            | 10       |
| 505   | 992.1570         | 0.0045 | -0.0260            | 10       |
| 506   | 992.4099         | 0.0020 | -0.0129            | 9        |
| 507   | 992.6490         | 0.0029 | -0.0135            | 9        |
| 508   | 992.8934         | 0.0031 | -0.0089            | 9        |
| 510   | 993.3905         | 0.0097 | 0.0088             | 9        |
| 537   | 999.8145         | 0.0029 | -0.0405            | 9        |
| 538   | 1000.0513        | 0.0021 | -0.0434            | 10       |
| 539   | 1000.2835        | 0.0038 | -0.0510            | 9        |
| 540   | 1000.5337        | 0.0039 | -0.0405            | 9        |
| 541   | 1000.7751        | 0.0048 | -0.0389            | 9        |
| 542   | 1001.0207        | 0.0056 | -0.0330            | 10       |
| 543   | 1001.2740        | 0.0034 | -0.0195            | 9        |
| 544   | 1001.5295        | 0.0027 | -0.0037            | 9        |
| 545   | 1001.7846        | 0.0029 | 0.0116             | 10       |
| 546   | 1002.0300        | 0.0042 | 0.0173             | 9        |
| 547   | 1002.2827        | 0.0071 | 0.0302             | 9        |
| 548   | 1002.5023        | 0.0094 | 0.0100             | 9        |
| 549   | 1002.7230        | 0.0082 | -0.0090            | 10       |
| 550   | 1003.0126        | 0.0175 | 0.0408             | 9        |
| 551   | 1003.2258        | 0.0114 | 0.0143             | 9        |
| 552   | 1003.4629        | 0.0065 | 0.0116             | 9        |
| 553   | 1003.6819        | 0.0076 | -0.0091            | 10       |
| 554   | 1003.9574        | 0.0167 | 0.0267             | 9        |
| 555   | 1004.1760        | 0.0086 | 0.0055             | 9        |
| 556   | 1004.4318        | 0.0076 | 0.0215             | 9        |
| 557   | 1004.6483        | 0.0165 | -0.0017            | 10       |
| 561   | 1005.5819        | 0.0092 | -0.0271            | 10       |
| 563   | 1006.0358        | 0.0136 | -0.0527            | 9        |
| 564   | 1006.2843        | 0.0081 | -0.0439            | 10       |
| 565   | 1006.5340        | 0.0059 | -0.0340            | 9        |
| 566   | 1006.7856        | 0.0141 | -0.0222            | 9        |
| 567   | 1007.0355        | 0.0042 | -0.0120            | 9        |
| 568   | 1007.2956        | 0.0030 | 0.0084             | 10       |
| 569   | 1007.5348        | 0.0047 | 0.0078             | 9        |
| 570   | 1007.7744        | 0.0054 | 0.0077             | 9        |
| 571   | 1008.0256        | 0.0036 | 0.0191             | 9        |
| 572   | 1008.2592        | 0.0164 | 0.0130             | 10       |
| 573   | 1008.5057        | 0.0061 | 0.0197             | 9        |
| 574   | 1008.7187        | 0.0118 | -0.0071            | 9        |
| 575   | 1008.9814        | 0.0062 | 0.0158             | 10       |
| 576   | 1009.2222        | 0.0097 | 0.0169             | 10       |
| 577   | 1009.4397        | 0.0058 | -0.0053            | 9        |
| 578   | 1009.6735        | 0.0052 | -0.0113            | 9        |
| 580   | 1010.1685        | 0.0037 | 0.0042             | 9        |
| 581   | 1010.3945        | 0.0059 | -0.0095            | 8        |
| 582   | 1010.6429        | 0.0040 | -0.0009            | 9        |
| 583   | 1010.9065        | 0.0045 | 0.0230             | 9        |
| 584   | 1011.1044        | 0.0056 | -0.0188            | 9        |

**Table E4.** Times of negative-superhump maxima in KIC 9406652 during time interval 4 (BJD 2455871–2456058) (continued).

| $E^*$ | Max <sup>†</sup> | Error  | $O - C^{\ddagger}$ | $N^{\S}$ |
|-------|------------------|--------|--------------------|----------|
| 585   | 1011.3628        | 0.0031 | -0.0002            | 9        |
| 586   | 1011.6250        | 0.0089 | 0.0222             | 10       |
| 587   | 1011.8229        | 0.0065 | -0.0196            | 9        |
| 588   | 1012.1112        | 0.0076 | 0.0290             | 9        |
| 589   | 1012.3307        | 0.0104 | 0.0087             | 9        |
| 590   | 1012.5802        | 0.0091 | 0.0184             | 10       |
| 591   | 1012.8072        | 0.0032 | 0.0057             | 10       |
| 592   | 1013.0440        | 0.0143 | 0.0028             | 6        |
| 593   | 1013.2991        | 0.0054 | 0.0181             | 9        |
| 594   | 1013.5276        | 0.0037 | 0.0068             | 10       |
| 595   | 1013.7610        | 0.0033 | 0.0005             | 9        |
| 596   | 1014.0080        | 0.0046 | 0.0078             | 9        |
| 597   | 1014.2488        | 0.0053 | 0.0088             | 9        |
| 598   | 1014.4741        | 0.0103 | -0.0056            | 10       |
| 599   | 1014.7084        | 0.0076 | -0.0111            | 9        |
| 600   | 1014.9624        | 0.0039 | 0.0032             | 8        |
| 604   | 1015.9399        | 0.0025 | 0.0217             | 9        |
| 605   | 1016.1756        | 0.0026 | 0.0176             | 10       |
| 606   | 1016.4040        | 0.0037 | 0.0063             | 10       |
| 607   | 1016.6425        | 0.0062 | 0.0050             | 9        |
| 608   | 1016.8778        | 0.0029 | 0.0006             | 9        |
| 609   | 1017.1338        | 0.0055 | 0.0168             | 10       |
| 610   | 1017.3767        | 0.0087 | 0.0200             | 9        |
| 611   | 1017.6095        | 0.0050 | 0.0130             | 9        |
| 612   | 1017.8445        | 0.0018 | 0.0082             | 9        |
| 613   | 1018.0976        | 0.0089 | 0.0216             | 9        |
| 614   | 1018.2919        | 0.0045 | -0.0238            | 8        |
| 615   | 1018.5648        | 0.0055 | 0.0093             | 9        |
| 616   | 1018.8087        | 0.0032 | 0.0134             | 10       |
| 617   | 1019.0347        | 0.0050 | -0.0003            | 10       |
| 618   | 1019.3023        | 0.0040 | 0.0275             | 9        |
| 619   | 1019.5233        | 0.0014 | 0.0088             | 9        |
| 620   | 1019.7647        | 0.0037 | 0.0105             | 10       |
| 621   | 1020.0113        | 0.0041 | 0.0173             | 10       |
| 622   | 1020.2560        | 0.0042 | 0.0222             | 9        |
| 623   | 1020.4970        | 0.0059 | 0.0235             | 9        |
| 624   | 1020.7257        | 0.0053 | 0.0124             | 10       |
| 625   | 1020.9832        | 0.0073 | 0.0302             | 7        |
| 626   | 1021.2044        | 0.0032 | 0.0117             | 9        |
| 627   | 1021.4437        | 0.0032 | 0.0112             | 9        |
| 628   | 1021.6726        | 0.0037 | 0.0004             | 10       |
| 629   | 1021.9301        | 0.0031 | 0.0181             | 9        |
| 630   | 1022.1544        | 0.0051 | 0.0026             | 9        |
| 631   | 1022.4035        | 0.0040 | 0.0120             | 10       |
| 632   | 1022.6368        | 0.0034 | 0.0055             | 10       |
| 633   | 1022.8807        | 0.0035 | 0.0097             | 9        |
| 634   | 1023.1125        | 0.0027 | 0.0017             | 9        |
| 635   | 1023.3597        | 0.0037 | 0.0092             | 10       |
| 636   | 1023.5896        | 0.0018 | -0.0006            | 10       |
| 637   | 1023.8379        | 0.0020 | 0.0079             | 9        |
| 638   | 1024.0728        | 0.0037 | 0.0031             | 8        |
| 639   | 1024.3184        | 0.0032 | 0.0089             | 10       |

**Table E4.** Times of negative-superhump maxima in KIC 9406652 during time interval 4 (BJD 2455871–2456058) (continued).

| $E^*$ | Max <sup>†</sup> | Error  | $O - C^{\ddagger}$ | $N^{\S}$ |
|-------|------------------|--------|--------------------|----------|
| 640   | 1024.5582        | 0.0021 | 0.0089             | 9        |
| 641   | 1024.7934        | 0.0025 | 0.0044             | 9        |
| 642   | 1025.0268        | 0.0044 | -0.0019            | 9        |
| 643   | 1025.2807        | 0.0077 | 0.0122             | 10       |
| 644   | 1025.4891        | 0.0082 | -0.0192            | 8        |
| 645   | 1025.7444        | 0.0031 | -0.0036            | 9        |
| 646   | 1025.9834        | 0.0036 | -0.0044            | 10       |
| 647   | 1026.2231        | 0.0031 | -0.0044            | 10       |
| 648   | 1026.4495        | 0.0022 | -0.0177            | 9        |
| 649   | 1026.7006        | 0.0036 | -0.0064            | 9        |
| 650   | 1026.9509        | 0.0061 | 0.0042             | 8        |
| 651   | 1027.1763        | 0.0037 | -0.0102            | 10       |
| 652   | 1027.4221        | 0.0018 | -0.0042            | 9        |
| 653   | 1027.6634        | 0.0022 | -0.0026            | 9        |
| 654   | 1027.8962        | 0.0024 | -0.0096            | 10       |
| 655   | 1028.1448        | 0.0034 | -0.0007            | 9        |
| 656   | 1028.3827        | 0.0031 | -0.0026            | 9        |
| 657   | 1028.6348        | 0.0054 | 0.0098             | 9        |
| 658   | 1028.8566        | 0.0036 | -0.0082            | 10       |
| 659   | 1029.0979        | 0.0048 | -0.0066            | 9        |
| 660   | 1029.3512        | 0.0045 | 0.0070             | 9        |
| 661   | 1029.5794        | 0.0025 | -0.0046            | 10       |
| 662   | 1029.8236        | 0.0027 | -0.0001            | 10       |
| 663   | 1030.0557        | 0.0070 | -0.0078            | 6        |
| 664   | 1030.2944        | 0.0059 | -0.0089            | 9        |
| 665   | 1030.5215        | 0.0027 | -0.0215            | 10       |
| 666   | 1030.7594        | 0.0046 | -0.0233            | 10       |
| 667   | 1031.0037        | 0.0020 | -0.0188            | 9        |
| 668   | 1031.2507        | 0.0041 | -0.0116            | 9        |
| 669   | 1031.4915        | 0.0029 | -0.0105            | 10       |
| 670   | 1031.7316        | 0.0024 | -0.0102            | 9        |
| 671   | 1031.9845        | 0.0022 | 0.0030             | 9        |
| 672   | 1032.2208        | 0.0051 | -0.0004            | 9        |
| 673   | 1032.4572        | 0.0070 | -0.0038            | 10       |
| 674   | 1032.6778        | 0.0036 | -0.0229            | 9        |
| 675   | 1032.9375        | 0.0022 | -0.0030            | 7        |
| 676   | 1033.1816        | 0.0027 | 0.0013             | 9        |
| 677   | 1033.4054        | 0.0072 | -0.0146            | 10       |
| 678   | 1033.6506        | 0.0060 | -0.0092            | 9        |
| 679   | 1033.8797        | 0.0071 | -0.0198            | 8        |
| 680   | 1034.1264        | 0.0086 | -0.0128            | 10       |
| 681   | 1034.3658        | 0.0056 | -0.0132            | 9        |
| 682   | 1034.5907        | 0.0030 | -0.0280            | 9        |
| 683   | 1034.8456        | 0.0038 | -0.0129            | 9        |
| 684   | 1035.0589        | 0.0065 | -0.0394            | 9        |
| 685   | 1035.3116        | 0.0034 | -0.0264            | 9        |
| 686   | 1035.5588        | 0.0077 | -0.0189            | 9        |
| 687   | 1035.7776        | 0.0071 | -0.0399            | 9        |
| 688   | 1036.0356        | 0.0050 | -0.0216            | 10       |
| 689   | 1036.2823        | 0.0026 | -0.0147            | 9        |
| 690   | 1036.5206        | 0.0064 | -0.0162            | 9        |
| 691   | 1036.7623        | 0.0062 | -0.0142            | 10       |

**Table E4.** Times of negative-superhump maxima in KIC 9406652 during time interval 4 (BJD 2455871–2456058) (continued).

| $E^*$ | Max <sup>†</sup> | Error  | $O - C^{\ddagger}$ | $N^{\S}$ |
|-------|------------------|--------|--------------------|----------|
| 692   | 1037.0014        | 0.0051 | -0.0149            | 10       |
| 693   | 1037.2427        | 0.0035 | -0.0133            | 9        |
| 694   | 1037.4764        | 0.0041 | -0.0193            | 9        |
| 695   | 1037.7334        | 0.0059 | -0.0021            | 10       |
| 696   | 1037.9681        | 0.0044 | -0.0072            | 9        |
| 697   | 1038.1993        | 0.0047 | -0.0157            | 9        |
| 698   | 1038.4099        | 0.0034 | -0.0448            | 9        |
| 699   | 1038.6682        | 0.0050 | -0.0263            | 10       |
| 701   | 1039.1485        | 0.0036 | -0.0255            | 9        |
| 702   | 1039.3830        | 0.0087 | -0.0307            | 10       |
| 703   | 1039.6083        | 0.0037 | -0.0452            | 10       |
| 704   | 1039.8543        | 0.0065 | -0.0390            | 9        |
| 705   | 1040.1079        | 0.0077 | -0.0251            | 9        |
| 706   | 1040.3449        | 0.0035 | -0.0279            | 10       |
| 707   | 1040.6051        | 0.0031 | -0.0074            | 10       |
| 708   | 1040.8465        | 0.0057 | -0.0057            | 8        |
| 709   | 1041.0881        | 0.0038 | -0.0039            | 9        |
| 710   | 1041.3186        | 0.0084 | -0.0132            | 10       |
| 711   | 1041.5909        | 0.0097 | 0.0194             | 9        |
| 720   | 1043.7069        | 0.0123 | -0.0223            | 9        |
| 721   | 1043.9383        | 0.0083 | -0.0307            | 10       |
| 722   | 1044.1893        | 0.0091 | -0.0195            | 10       |
| 726   | 1045.1153        | 0.0175 | -0.0524            | 9        |
| 728   | 1045.5976        | 0.0086 | -0.0496            | 9        |
| 729   | 1045.8547        | 0.0060 | -0.0323            | 10       |
| 730   | 1046.0766        | 0.0063 | -0.0501            | 9        |
| 731   | 1046.3337        | 0.0104 | -0.0328            | 9        |
| 732   | 1046.6037        | 0.0090 | -0.0025            | 10       |
| 733   | 1046.8528        | 0.0076 | 0.0068             | 10       |
| 734   | 1047.0951        | 0.0025 | 0.0093             | 9        |
| 736   | 1047.5905        | 0.0044 | 0.0253             | 10       |
| 741   | 1048.7894        | 0.0057 | 0.0254             | 7        |
| 746   | 1049.9430        | 0.0042 | -0.0197            | 9        |
| 747   | 1050.1965        | 0.0082 | -0.0060            | 10       |
| 748   | 1050.4301        | 0.0051 | -0.0121            | 10       |
| 749   | 1050.6563        | 0.0039 | -0.0257            | 8        |
| 750   | 1050.8999        | 0.0093 | -0.0219            | 9        |
| 751   | 1051.1545        | 0.0060 | -0.0070            | 9        |
| 752   | 1051.3841        | 0.0056 | -0.0172            | 10       |
| 753   | 1051.6440        | 0.0038 | 0.0030             | 9        |
| 754   | 1051.8737        | 0.0037 | -0.0070            | 9        |
| 755   | 1052.1420        | 0.0051 | 0.0215             | 10       |
| 756   | 1052.3585        | 0.0030 | -0.0017            | 9        |
| 757   | 1052.6047        | 0.0035 | 0.0047             | 9        |
| 758   | 1052.8651        | 0.0118 | 0.0253             | 9        |
| 759   | 1053.0907        | 0.0053 | 0.0112             | 10       |
| 760   | 1053.3380        | 0.0038 | 0.0187             | 9        |
| 761   | 1053.5539        | 0.0032 | -0.0051            | 6        |
| 762   | 1053.8182        | 0.0018 | 0.0194             | 8        |
| 763   | 1054.0420        | 0.0022 | 0.0035             | 10       |
| 764   | 1054.2877        | 0.0030 | 0.0095             | 9        |
| 765   | 1054.5324        | 0.0038 | 0.0144             | 9        |

**Table E4.** Times of negative-superhump maxima in KIC 9406652 during time interval 4 (BJD 2455871–2456058) (continued).

| $E^*$ | Max <sup>†</sup> | Error  | $O - C^‡$ | $N^§$ |
|-------|------------------|--------|-----------|-------|
| 766   | 1054.7740        | 0.0032 | 0.0162    | 10    |
| 767   | 1055.0082        | 0.0034 | 0.0107    | 10    |
| 768   | 1055.2569        | 0.0034 | 0.0196    | 9     |
| 769   | 1055.4929        | 0.0023 | 0.0159    | 9     |
| 770   | 1055.7343        | 0.0033 | 0.0175    | 10    |
| 771   | 1055.9859        | 0.0028 | 0.0294    | 9     |
| 772   | 1056.2217        | 0.0026 | 0.0254    | 9     |
| 773   | 1056.4558        | 0.0024 | 0.0198    | 9     |
| 774   | 1056.6922        | 0.0049 | 0.0164    | 9     |
| 775   | 1056.9369        | 0.0040 | 0.0214    | 9     |
| 776   | 1057.1755        | 0.0045 | 0.0202    | 9     |
| 777   | 1057.4297        | 0.0075 | 0.0347    | 10    |
| 778   | 1057.6779        | 0.0067 | 0.0431    | 10    |
| 779   | 1057.8944        | 0.0080 | 0.0199    | 9     |

\*Cycle counts.

<sup>†</sup>BJD–2455000.0.

<sup>‡</sup> $C = 2455871.1184 + 0.23975 E$ .

<sup>§</sup>Number of points used for determining the maximum.

**Table E5.** Times of negative-superhump maxima in KIC 9406652 during time interval 5 (BJD 2456058–2456200).

| $E^*$ | Max <sup>†</sup> | Error  | $O - C^{\ddagger}$ | $N^{\S}$ |
|-------|------------------|--------|--------------------|----------|
| 0     | 1058.1206        | 0.0060 | -0.0261            | 10       |
| 1     | 1058.3743        | 0.0039 | -0.0120            | 9        |
| 2     | 1058.6142        | 0.0047 | -0.0117            | 9        |
| 3     | 1058.8540        | 0.0057 | -0.0115            | 10       |
| 4     | 1059.1069        | 0.0029 | 0.0019             | 10       |
| 5     | 1059.3387        | 0.0029 | -0.0059            | 9        |
| 6     | 1059.5791        | 0.0029 | -0.0050            | 8        |
| 7     | 1059.8190        | 0.0050 | -0.0047            | 9        |
| 8     | 1060.0574        | 0.0056 | -0.0059            | 9        |
| 9     | 1060.2995        | 0.0037 | -0.0033            | 9        |
| 10    | 1060.5380        | 0.0051 | -0.0044            | 10       |
| 11    | 1060.7825        | 0.0034 | 0.0005             | 10       |
| 12    | 1061.0016        | 0.0161 | -0.0199            | 9        |
| 13    | 1061.2422        | 0.0042 | -0.0188            | 9        |
| 14    | 1061.4820        | 0.0037 | -0.0186            | 10       |
| 15    | 1061.7330        | 0.0044 | -0.0071            | 9        |
| 16    | 1061.9670        | 0.0020 | -0.0127            | 7        |
| 17    | 1062.2048        | 0.0057 | -0.0145            | 9        |
| 18    | 1062.4419        | 0.0044 | -0.0169            | 10       |
| 19    | 1062.6981        | 0.0049 | -0.0003            | 8        |
| 20    | 1062.9279        | 0.0026 | -0.0101            | 9        |
| 21    | 1063.1725        | 0.0043 | -0.0051            | 10       |
| 22    | 1063.4029        | 0.0024 | -0.0142            | 10       |
| 23    | 1063.6412        | 0.0040 | -0.0154            | 9        |
| 24    | 1063.8859        | 0.0023 | -0.0103            | 9        |
| 25    | 1064.1267        | 0.0019 | -0.0091            | 10       |
| 26    | 1064.3787        | 0.0029 | 0.0034             | 9        |
| 28    | 1064.8711        | 0.0089 | 0.0166             | 10       |
| 29    | 1065.0878        | 0.0031 | -0.0062            | 10       |
| 30    | 1065.3333        | 0.0051 | -0.0002            | 9        |
| 31    | 1065.5700        | 0.0049 | -0.0031            | 9        |
| 32    | 1065.8118        | 0.0047 | -0.0009            | 9        |
| 33    | 1066.0294        | 0.0047 | -0.0228            | 9        |
| 34    | 1066.2875        | 0.0034 | -0.0043            | 9        |
| 35    | 1066.5239        | 0.0024 | -0.0074            | 9        |
| 36    | 1066.7569        | 0.0023 | -0.0140            | 10       |
| 37    | 1066.9990        | 0.0030 | -0.0115            | 9        |
| 38    | 1067.2287        | 0.0033 | -0.0213            | 9        |
| 39    | 1067.4772        | 0.0021 | -0.0124            | 10       |
| 40    | 1067.7186        | 0.0019 | -0.0105            | 10       |
| 41    | 1067.9684        | 0.0028 | -0.0003            | 8        |
| 42    | 1068.2077        | 0.0033 | -0.0006            | 7        |
| 43    | 1068.4414        | 0.0024 | -0.0064            | 10       |
| 44    | 1068.6929        | 0.0019 | 0.0055             | 8        |
| 45    | 1068.9214        | 0.0022 | -0.0055            | 9        |
| 46    | 1069.1682        | 0.0030 | 0.0017             | 9        |
| 47    | 1069.4093        | 0.0044 | 0.0032             | 10       |
| 48    | 1069.6415        | 0.0022 | -0.0041            | 9        |
| 49    | 1069.8795        | 0.0025 | -0.0057            | 9        |
| 50    | 1070.1099        | 0.0037 | -0.0149            | 10       |
| 51    | 1070.3481        | 0.0025 | -0.0162            | 10       |
| 52    | 1070.5879        | 0.0025 | -0.0160            | 9        |

**Table E5.** Times of negative-superhump maxima in KIC 9406652 during time interval 5 (BJD 2456058–2456200) (continued).

| $E^*$ | Max <sup>†</sup> | Error  | $O - C^{\ddagger}$ | $N^{\S}$ |
|-------|------------------|--------|--------------------|----------|
| 53    | 1070.8221        | 0.0043 | -0.0213            | 9        |
| 54    | 1071.0640        | 0.0023 | -0.0190            | 10       |
| 55    | 1071.3033        | 0.0017 | -0.0193            | 9        |
| 56    | 1071.5467        | 0.0016 | -0.0154            | 9        |
| 57    | 1071.7903        | 0.0014 | -0.0114            | 10       |
| 58    | 1072.0315        | 0.0016 | -0.0097            | 10       |
| 59    | 1072.2788        | 0.0019 | -0.0020            | 9        |
| 60    | 1072.5233        | 0.0024 | 0.0030             | 9        |
| 62    | 1073.0009        | 0.0011 | 0.0014             | 9        |
| 63    | 1073.2344        | 0.0018 | -0.0047            | 9        |
| 64    | 1073.4692        | 0.0056 | -0.0094            | 9        |
| 65    | 1073.7106        | 0.0021 | -0.0075            | 10       |
| 66    | 1073.9596        | 0.0037 | 0.0018             | 9        |
| 67    | 1074.1826        | 0.0040 | -0.0146            | 9        |
| 68    | 1074.4182        | 0.0022 | -0.0187            | 8        |
| 69    | 1074.6628        | 0.0022 | -0.0136            | 9        |
| 70    | 1074.9002        | 0.0019 | -0.0157            | 9        |
| 71    | 1075.1456        | 0.0024 | -0.0100            | 9        |
| 72    | 1075.3845        | 0.0016 | -0.0106            | 10       |
| 73    | 1075.6224        | 0.0013 | -0.0123            | 9        |
| 74    | 1075.8682        | 0.0026 | -0.0060            | 9        |
| 75    | 1076.1052        | 0.0017 | -0.0086            | 10       |
| 76    | 1076.3458        | 0.0018 | -0.0076            | 10       |
| 77    | 1076.5818        | 0.0015 | -0.0111            | 9        |
| 78    | 1076.8305        | 0.0027 | -0.0019            | 9        |
| 79    | 1077.0554        | 0.0030 | -0.0166            | 10       |
| 80    | 1077.2999        | 0.0034 | -0.0116            | 9        |
| 81    | 1077.5392        | 0.0040 | -0.0120            | 9        |
| 82    | 1077.7828        | 0.0052 | -0.0079            | 9        |
| 87    | 1078.9641        | 0.0022 | -0.0244            | 10       |
| 88    | 1079.2006        | 0.0020 | -0.0274            | 8        |
| 89    | 1079.4450        | 0.0023 | -0.0226            | 9        |
| 90    | 1079.6868        | 0.0023 | -0.0204            | 10       |
| 91    | 1079.9329        | 0.0029 | -0.0138            | 9        |
| 92    | 1080.1627        | 0.0019 | -0.0236            | 9        |
| 93    | 1080.4112        | 0.0026 | -0.0147            | 9        |
| 94    | 1080.6529        | 0.0026 | -0.0125            | 9        |
| 95    | 1080.8877        | 0.0035 | -0.0172            | 9        |
| 96    | 1081.1307        | 0.0026 | -0.0138            | 9        |
| 97    | 1081.3697        | 0.0038 | -0.0144            | 10       |
| 98    | 1081.6127        | 0.0024 | -0.0110            | 10       |
| 99    | 1081.8492        | 0.0053 | -0.0140            | 9        |
| 100   | 1082.0812        | 0.0042 | -0.0216            | 9        |
| 101   | 1082.3197        | 0.0066 | -0.0226            | 10       |
| 102   | 1082.5504        | 0.0049 | -0.0315            | 9        |
| 103   | 1082.7927        | 0.0022 | -0.0288            | 9        |
| 104   | 1083.0397        | 0.0032 | -0.0213            | 10       |
| 105   | 1083.2725        | 0.0010 | -0.0281            | 10       |
| 106   | 1083.5111        | 0.0015 | -0.0290            | 8        |
| 107   | 1083.7509        | 0.0029 | -0.0288            | 9        |
| 108   | 1083.9944        | 0.0017 | -0.0248            | 10       |
| 109   | 1084.2369        | 0.0031 | -0.0219            | 9        |

**Table E5.** Times of negative-superhump maxima in KIC 9406652 during time interval 5 (BJD 2456058–2456200) (continued).

| $E^*$ | Max <sup>†</sup> | Error  | $O - C^{\ddagger}$ | $N^{\S}$ |
|-------|------------------|--------|--------------------|----------|
| 110   | 1084.4747        | 0.0025 | -0.0237            | 9        |
| 111   | 1084.7221        | 0.0022 | -0.0158            | 9        |
| 112   | 1084.9707        | 0.0039 | -0.0068            | 10       |
| 113   | 1085.2050        | 0.0037 | -0.0120            | 9        |
| 114   | 1085.4327        | 0.0028 | -0.0239            | 9        |
| 115   | 1085.6795        | 0.0034 | -0.0166            | 10       |
| 116   | 1085.9143        | 0.0088 | -0.0214            | 10       |
| 117   | 1086.1501        | 0.0036 | -0.0252            | 9        |
| 118   | 1086.3885        | 0.0102 | -0.0263            | 9        |
| 119   | 1086.6254        | 0.0022 | -0.0290            | 8        |
| 120   | 1086.8738        | 0.0038 | -0.0202            | 9        |
| 121   | 1087.1055        | 0.0051 | -0.0280            | 9        |
| 122   | 1087.3477        | 0.0026 | -0.0254            | 10       |
| 123   | 1087.5920        | 0.0034 | -0.0206            | 10       |
| 124   | 1087.8347        | 0.0030 | -0.0175            | 9        |
| 125   | 1088.0724        | 0.0046 | -0.0194            | 9        |
| 126   | 1088.3083        | 0.0034 | -0.0230            | 10       |
| 127   | 1088.5375        | 0.0078 | -0.0333            | 9        |
| 128   | 1088.7791        | 0.0059 | -0.0313            | 9        |
| 129   | 1089.0249        | 0.0070 | -0.0251            | 9        |
| 130   | 1089.2585        | 0.0062 | -0.0311            | 10       |
| 131   | 1089.4896        | 0.0051 | -0.0395            | 8        |
| 132   | 1089.7340        | 0.0043 | -0.0347            | 9        |
| 133   | 1089.9752        | 0.0045 | -0.0331            | 10       |
| 134   | 1090.2144        | 0.0059 | -0.0334            | 10       |
| 135   | 1090.4455        | 0.0038 | -0.0419            | 9        |
| 136   | 1090.6858        | 0.0035 | -0.0411            | 9        |
| 137   | 1090.9312        | 0.0022 | -0.0353            | 10       |
| 138   | 1091.1749        | 0.0036 | -0.0311            | 9        |
| 139   | 1091.4114        | 0.0046 | -0.0342            | 9        |
| 140   | 1091.6526        | 0.0027 | -0.0326            | 9        |
| 141   | 1091.8868        | 0.0031 | -0.0379            | 10       |
| 142   | 1092.1332        | 0.0036 | -0.0311            | 9        |
| 143   | 1092.3610        | 0.0047 | -0.0428            | 9        |
| 144   | 1092.6068        | 0.0038 | -0.0366            | 9        |
| 145   | 1092.8472        | 0.0084 | -0.0358            | 10       |
| 146   | 1093.0834        | 0.0069 | -0.0391            | 9        |
| 147   | 1093.3209        | 0.0044 | -0.0412            | 9        |
| 148   | 1093.5534        | 0.0051 | -0.0482            | 10       |
| 150   | 1094.0402        | 0.0061 | -0.0406            | 9        |
| 151   | 1094.2758        | 0.0030 | -0.0446            | 10       |
| 152   | 1094.5180        | 0.0029 | -0.0419            | 10       |
| 153   | 1094.7470        | 0.0073 | -0.0525            | 9        |
| 154   | 1094.9936        | 0.0065 | -0.0454            | 9        |
| 155   | 1095.2318        | 0.0029 | -0.0467            | 10       |
| 156   | 1095.4753        | 0.0016 | -0.0428            | 8        |
| 157   | 1095.7114        | 0.0041 | -0.0462            | 9        |
| 158   | 1095.9745        | 0.0083 | -0.0227            | 9        |
| 159   | 1096.2040        | 0.0023 | -0.0328            | 10       |
| 160   | 1096.4534        | 0.0021 | -0.0229            | 9        |
| 161   | 1096.6908        | 0.0042 | -0.0251            | 9        |
| 162   | 1096.9279        | 0.0078 | -0.0276            | 10       |

**Table E5.** Times of negative-superhump maxima in KIC 9406652 during time interval 5 (BJD 2456058–2456200) (continued).

| $E^*$ | Max <sup>†</sup> | Error  | $O - C^{\ddagger}$ | $N^{\S}$ |
|-------|------------------|--------|--------------------|----------|
| 163   | 1097.1749        | 0.0053 | -0.0201            | 10       |
| 165   | 1097.6396        | 0.0017 | -0.0345            | 9        |
| 166   | 1097.9026        | 0.0122 | -0.0111            | 10       |
| 167   | 1098.1465        | 0.0037 | -0.0067            | 9        |
| 168   | 1098.3550        | 0.0078 | -0.0378            | 9        |
| 169   | 1098.6110        | 0.0076 | -0.0214            | 10       |
| 170   | 1098.8608        | 0.0095 | -0.0111            | 10       |
| 171   | 1099.0931        | 0.0045 | -0.0184            | 9        |
| 172   | 1099.3585        | 0.0048 | 0.0074             | 9        |
| 173   | 1099.5865        | 0.0098 | -0.0042            | 10       |
| 174   | 1099.8218        | 0.0051 | -0.0084            | 9        |
| 175   | 1100.0409        | 0.0090 | -0.0288            | 9        |
| 176   | 1100.2922        | 0.0090 | -0.0171            | 7        |
| 177   | 1100.5296        | 0.0050 | -0.0192            | 10       |
| 178   | 1100.7843        | 0.0074 | -0.0042            | 9        |
| 179   | 1101.0063        | 0.0086 | -0.0217            | 9        |
| 180   | 1101.2477        | 0.0063 | -0.0198            | 10       |
| 181   | 1101.5100        | 0.0024 | 0.0029             | 9        |
| 186   | 1102.7082        | 0.0099 | 0.0033             | 9        |
| 187   | 1102.9370        | 0.0064 | -0.0075            | 9        |
| 189   | 1103.3898        | 0.0051 | -0.0338            | 9        |
| 190   | 1103.6575        | 0.0060 | -0.0057            | 8        |
| 191   | 1103.8928        | 0.0028 | -0.0099            | 10       |
| 192   | 1104.1137        | 0.0100 | -0.0285            | 10       |
| 193   | 1104.3629        | 0.0035 | -0.0189            | 8        |
| 194   | 1104.6038        | 0.0047 | -0.0176            | 9        |
| 195   | 1104.8575        | 0.0026 | -0.0035            | 10       |
| 196   | 1105.1030        | 0.0073 | 0.0025             | 9        |
| 197   | 1105.3267        | 0.0051 | -0.0134            | 9        |
| 198   | 1105.5630        | 0.0061 | -0.0166            | 10       |
| 199   | 1105.8113        | 0.0054 | -0.0079            | 10       |
| 200   | 1106.0074        | 0.0076 | -0.0513            | 5        |
| 205   | 1107.2522        | 0.0034 | -0.0043            | 9        |
| 206   | 1107.4912        | 0.0025 | -0.0049            | 10       |
| 207   | 1107.7247        | 0.0025 | -0.0110            | 9        |
| 208   | 1107.9892        | 0.0029 | 0.0140             | 9        |
| 209   | 1108.2122        | 0.0032 | -0.0026            | 10       |
| 210   | 1108.4547        | 0.0018 | 0.0003             | 10       |
| 211   | 1108.6984        | 0.0027 | 0.0045             | 9        |
| 212   | 1108.9433        | 0.0033 | 0.0098             | 9        |
| 213   | 1109.1856        | 0.0021 | 0.0125             | 9        |
| 214   | 1109.4297        | 0.0029 | 0.0171             | 9        |
| 215   | 1109.6662        | 0.0029 | 0.0141             | 9        |
| 216   | 1109.9116        | 0.0035 | 0.0198             | 10       |
| 217   | 1110.1510        | 0.0041 | 0.0197             | 10       |
| 218   | 1110.3968        | 0.0048 | 0.0259             | 9        |
| 219   | 1110.6351        | 0.0040 | 0.0247             | 9        |
| 220   | 1110.8696        | 0.0025 | 0.0196             | 10       |
| 221   | 1111.1102        | 0.0027 | 0.0207             | 9        |
| 222   | 1111.3442        | 0.0031 | 0.0151             | 9        |
| 223   | 1111.6143        | 0.0049 | 0.0456             | 9        |
| 224   | 1111.8401        | 0.0037 | 0.0319             | 7        |

**Table E5.** Times of negative-superhump maxima in KIC 9406652 during time interval 5 (BJD 2456058–2456200) (continued).

| $E^*$ | Max <sup>†</sup> | Error  | $O - C^{\ddagger}$ | $N^{\S}$ |
|-------|------------------|--------|--------------------|----------|
| 225   | 1112.0858        | 0.0057 | 0.0380             | 8        |
| 226   | 1112.3230        | 0.0035 | 0.0356             | 9        |
| 227   | 1112.5637        | 0.0024 | 0.0368             | 10       |
| 228   | 1112.8148        | 0.0022 | 0.0483             | 10       |
| 229   | 1113.0507        | 0.0025 | 0.0447             | 5        |
| 230   | 1113.2803        | 0.0038 | 0.0347             | 9        |
| 231   | 1113.5247        | 0.0026 | 0.0396             | 10       |
| 232   | 1113.7531        | 0.0034 | 0.0284             | 9        |
| 233   | 1113.9970        | 0.0024 | 0.0328             | 9        |
| 234   | 1114.2342        | 0.0013 | 0.0304             | 8        |
| 235   | 1114.4763        | 0.0018 | 0.0329             | 10       |
| 236   | 1114.7193        | 0.0018 | 0.0364             | 9        |
| 237   | 1114.9565        | 0.0024 | 0.0340             | 9        |
| 238   | 1115.2002        | 0.0025 | 0.0382             | 10       |
| 239   | 1115.4430        | 0.0030 | 0.0414             | 9        |
| 240   | 1115.6831        | 0.0016 | 0.0419             | 9        |
| 241   | 1115.9254        | 0.0024 | 0.0447             | 9        |
| 242   | 1116.1598        | 0.0020 | 0.0395             | 10       |
| 243   | 1116.3991        | 0.0019 | 0.0393             | 8        |
| 244   | 1116.6399        | 0.0026 | 0.0405             | 9        |
| 245   | 1116.8833        | 0.0020 | 0.0444             | 10       |
| 246   | 1117.1203        | 0.0017 | 0.0418             | 10       |
| 247   | 1117.3582        | 0.0036 | 0.0401             | 9        |
| 248   | 1117.6026        | 0.0028 | 0.0450             | 9        |
| 249   | 1117.8464        | 0.0043 | 0.0492             | 9        |
| 250   | 1118.0782        | 0.0044 | 0.0414             | 8        |
| 251   | 1118.3166        | 0.0036 | 0.0403             | 9        |
| 252   | 1118.5582        | 0.0021 | 0.0423             | 9        |
| 253   | 1118.7967        | 0.0029 | 0.0413             | 10       |
| 254   | 1119.0323        | 0.0014 | 0.0373             | 9        |
| 255   | 1119.2729        | 0.0027 | 0.0383             | 9        |
| 256   | 1119.5172        | 0.0015 | 0.0431             | 10       |
| 257   | 1119.7558        | 0.0029 | 0.0421             | 10       |
| 258   | 1119.9947        | 0.0021 | 0.0415             | 9        |
| 259   | 1120.2337        | 0.0022 | 0.0409             | 9        |
| 260   | 1120.4720        | 0.0018 | 0.0396             | 10       |
| 261   | 1120.7173        | 0.0045 | 0.0453             | 9        |
| 262   | 1120.9510        | 0.0031 | 0.0395             | 9        |
| 263   | 1121.1955        | 0.0022 | 0.0444             | 10       |
| 264   | 1121.4372        | 0.0023 | 0.0466             | 10       |
| 265   | 1121.6766        | 0.0040 | 0.0464             | 9        |
| 266   | 1121.9153        | 0.0032 | 0.0455             | 9        |
| 267   | 1122.1525        | 0.0033 | 0.0432             | 10       |
| 268   | 1122.3853        | 0.0035 | 0.0364             | 9        |
| 298   | 1129.5802        | 0.0026 | 0.0445             | 9        |
| 299   | 1129.8207        | 0.0019 | 0.0455             | 9        |
| 300   | 1130.0571        | 0.0034 | 0.0424             | 10       |
| 301   | 1130.2991        | 0.0022 | 0.0448             | 9        |
| 302   | 1130.5337        | 0.0024 | 0.0398             | 9        |
| 303   | 1130.7694        | 0.0010 | 0.0359             | 10       |
| 304   | 1131.0164        | 0.0020 | 0.0434             | 10       |
| 305   | 1131.2530        | 0.0012 | 0.0404             | 8        |

**Table E5.** Times of negative-superhump maxima in KIC 9406652 during time interval 5 (BJD 2456058–2456200) (continued).

| $E^*$ | Max <sup>†</sup> | Error  | $O - C^{\ddagger}$ | $N^{\S}$ |
|-------|------------------|--------|--------------------|----------|
| 306   | 1131.4949        | 0.0020 | 0.0428             | 9        |
| 307   | 1131.7302        | 0.0012 | 0.0385             | 10       |
| 308   | 1131.9757        | 0.0027 | 0.0445             | 9        |
| 309   | 1132.2112        | 0.0021 | 0.0404             | 9        |
| 310   | 1132.4524        | 0.0016 | 0.0420             | 9        |
| 311   | 1132.6908        | 0.0012 | 0.0409             | 10       |
| 312   | 1132.9254        | 0.0037 | 0.0359             | 9        |
| 313   | 1133.1657        | 0.0023 | 0.0367             | 9        |
| 314   | 1133.4117        | 0.0020 | 0.0431             | 10       |
| 315   | 1133.6529        | 0.0018 | 0.0447             | 10       |
| 316   | 1133.8832        | 0.0024 | 0.0355             | 9        |
| 317   | 1134.1245        | 0.0035 | 0.0372             | 9        |
| 318   | 1134.3621        | 0.0022 | 0.0352             | 9        |
| 319   | 1134.6043        | 0.0041 | 0.0379             | 9        |
| 320   | 1134.8389        | 0.0043 | 0.0329             | 9        |
| 321   | 1135.0804        | 0.0028 | 0.0349             | 10       |
| 322   | 1135.3271        | 0.0034 | 0.0420             | 10       |
| 323   | 1135.5678        | 0.0049 | 0.0432             | 9        |
| 324   | 1135.8018        | 0.0032 | 0.0376             | 9        |
| 325   | 1136.0452        | 0.0047 | 0.0415             | 10       |
| 326   | 1136.2904        | 0.0029 | 0.0471             | 9        |
| 327   | 1136.5248        | 0.0014 | 0.0419             | 9        |
| 328   | 1136.7686        | 0.0019 | 0.0462             | 9        |
| 329   | 1137.0008        | 0.0016 | 0.0388             | 10       |
| 330   | 1137.2399        | 0.0025 | 0.0383             | 8        |
| 331   | 1137.4841        | 0.0022 | 0.0429             | 9        |
| 332   | 1137.7207        | 0.0024 | 0.0400             | 10       |
| 333   | 1137.9489        | 0.0041 | 0.0286             | 9        |
| 339   | 1139.3880        | 0.0036 | 0.0304             | 10       |
| 340   | 1139.6294        | 0.0015 | 0.0323             | 10       |
| 341   | 1139.8756        | 0.0023 | 0.0389             | 9        |
| 342   | 1140.1148        | 0.0031 | 0.0385             | 9        |
| 343   | 1140.3545        | 0.0022 | 0.0386             | 10       |
| 344   | 1140.5920        | 0.0021 | 0.0366             | 9        |
| 345   | 1140.8274        | 0.0014 | 0.0324             | 9        |
| 346   | 1141.0694        | 0.0014 | 0.0349             | 8        |
| 347   | 1141.3091        | 0.0023 | 0.0350             | 10       |
| 348   | 1141.5468        | 0.0025 | 0.0331             | 9        |
| 349   | 1141.7816        | 0.0022 | 0.0284             | 9        |
| 350   | 1142.0174        | 0.0026 | 0.0246             | 10       |
| 351   | 1142.2672        | 0.0011 | 0.0349             | 10       |
| 352   | 1142.4931        | 0.0017 | 0.0212             | 9        |
| 353   | 1142.7370        | 0.0020 | 0.0255             | 9        |
| 354   | 1142.9725        | 0.0021 | 0.0215             | 10       |
| 355   | 1143.2163        | 0.0033 | 0.0257             | 9        |
| 356   | 1143.4613        | 0.0022 | 0.0311             | 9        |
| 357   | 1143.6947        | 0.0023 | 0.0251             | 9        |
| 358   | 1143.9351        | 0.0026 | 0.0259             | 9        |
| 359   | 1144.1791        | 0.0022 | 0.0303             | 9        |
| 360   | 1144.4159        | 0.0028 | 0.0276             | 9        |
| 361   | 1144.6605        | 0.0034 | 0.0325             | 10       |
| 362   | 1144.8968        | 0.0015 | 0.0293             | 10       |

**Table E5.** Times of negative-superhump maxima in KIC 9406652 during time interval 5 (BJD 2456058–2456200) (continued).

| $E^*$ | Max <sup>†</sup> | Error  | $O - C^\ddagger$ | $N^\S$ |
|-------|------------------|--------|------------------|--------|
| 363   | 1145.1298        | 0.0019 | 0.0228           | 9      |
| 364   | 1145.3702        | 0.0023 | 0.0236           | 9      |
| 365   | 1145.6113        | 0.0026 | 0.0252           | 10     |
| 366   | 1145.8526        | 0.0034 | 0.0268           | 9      |
| 367   | 1146.0834        | 0.0021 | 0.0182           | 9      |
| 368   | 1146.3264        | 0.0030 | 0.0216           | 10     |
| 369   | 1146.5590        | 0.0024 | 0.0146           | 10     |
| 370   | 1146.8040        | 0.0024 | 0.0201           | 9      |
| 371   | 1147.0397        | 0.0017 | 0.0162           | 8      |
| 372   | 1147.2806        | 0.0008 | 0.0176           | 10     |
| 373   | 1147.5175        | 0.0015 | 0.0149           | 9      |
| 374   | 1147.7559        | 0.0020 | 0.0137           | 9      |
| 375   | 1147.9930        | 0.0020 | 0.0112           | 9      |
| 376   | 1148.2449        | 0.0015 | 0.0236           | 10     |
| 377   | 1148.4810        | 0.0012 | 0.0201           | 9      |
| 378   | 1148.7183        | 0.0030 | 0.0178           | 9      |
| 379   | 1148.9593        | 0.0029 | 0.0193           | 10     |
| 380   | 1149.2019        | 0.0021 | 0.0223           | 10     |
| 381   | 1149.4318        | 0.0029 | 0.0127           | 9      |
| 382   | 1149.6739        | 0.0030 | 0.0152           | 9      |
| 383   | 1149.9077        | 0.0017 | 0.0094           | 9      |
| 384   | 1150.1439        | 0.0026 | 0.0061           | 9      |
| 385   | 1150.3893        | 0.0015 | 0.0120           | 9      |
| 386   | 1150.6255        | 0.0021 | 0.0086           | 9      |
| 387   | 1150.8612        | 0.0019 | 0.0047           | 10     |
| 388   | 1151.1034        | 0.0027 | 0.0074           | 9      |
| 389   | 1151.3474        | 0.0017 | 0.0118           | 9      |
| 390   | 1151.5875        | 0.0015 | 0.0123           | 10     |
| 391   | 1151.8309        | 0.0025 | 0.0162           | 10     |
| 392   | 1152.0686        | 0.0062 | 0.0143           | 9      |
| 393   | 1152.3072        | 0.0020 | 0.0133           | 9      |
| 394   | 1152.5517        | 0.0019 | 0.0183           | 10     |
| 395   | 1152.7846        | 0.0020 | 0.0117           | 9      |
| 396   | 1153.0214        | 0.0029 | 0.0089           | 8      |
| 397   | 1153.2556        | 0.0026 | 0.0035           | 10     |
| 398   | 1153.5006        | 0.0024 | 0.0089           | 10     |
| 399   | 1153.7373        | 0.0022 | 0.0061           | 9      |
| 400   | 1153.9842        | 0.0045 | 0.0135           | 9      |
| 401   | 1154.2046        | 0.0039 | -0.0057          | 10     |
| 402   | 1154.4505        | 0.0013 | 0.0006           | 9      |
| 403   | 1154.6853        | 0.0015 | -0.0041          | 9      |
| 404   | 1154.9246        | 0.0010 | -0.0044          | 9      |
| 405   | 1155.1637        | 0.0011 | -0.0048          | 10     |
| 406   | 1155.4105        | 0.0024 | 0.0024           | 9      |
| 407   | 1155.6586        | 0.0018 | 0.0110           | 9      |
| 408   | 1155.8942        | 0.0024 | 0.0070           | 9      |
| 409   | 1156.1312        | 0.0013 | 0.0044           | 8      |
| 410   | 1156.3706        | 0.0024 | 0.0042           | 9      |
| 411   | 1156.6100        | 0.0011 | 0.0040           | 9      |
| 412   | 1156.8474        | 0.0022 | 0.0019           | 10     |
| 413   | 1157.0845        | 0.0023 | -0.0006          | 9      |
| 414   | 1157.3325        | 0.0026 | 0.0079           | 9      |

**Table E5.** Times of negative-superhump maxima in KIC 9406652 during time interval 5 (BJD 2456058–2456200) (continued).

| $E^*$ | Max <sup>†</sup> | Error  | $O - C^\ddagger$ | $N^\S$ |
|-------|------------------|--------|------------------|--------|
| 415   | 1157.5669        | 0.0015 | 0.0028           | 10     |
| 416   | 1157.8039        | 0.0024 | 0.0002           | 10     |
| 417   | 1158.0364        | 0.0024 | -0.0069          | 9      |
| 418   | 1158.2763        | 0.0017 | -0.0065          | 9      |
| 419   | 1158.5167        | 0.0024 | -0.0057          | 10     |
| 420   | 1158.7483        | 0.0023 | -0.0137          | 9      |
| 421   | 1158.9903        | 0.0015 | -0.0112          | 8      |
| 422   | 1159.2367        | 0.0020 | -0.0043          | 9      |
| 423   | 1159.4763        | 0.0036 | -0.0043          | 10     |
| 424   | 1159.7190        | 0.0014 | -0.0012          | 9      |
| 425   | 1159.9607        | 0.0030 | 0.0009           | 9      |
| 426   | 1160.1931        | 0.0030 | -0.0062          | 10     |
| 427   | 1160.4314        | 0.0024 | -0.0074          | 10     |
| 428   | 1160.6683        | 0.0024 | -0.0101          | 9      |
| 429   | 1160.9223        | 0.0024 | 0.0043           | 9      |
| 430   | 1161.1463        | 0.0040 | -0.0113          | 10     |
| 431   | 1161.3892        | 0.0027 | -0.0079          | 9      |
| 432   | 1161.6210        | 0.0030 | -0.0157          | 9      |
| 433   | 1161.8582        | 0.0026 | -0.0181          | 8      |
| 434   | 1162.0974        | 0.0025 | -0.0184          | 10     |
| 435   | 1162.3371        | 0.0029 | -0.0183          | 9      |
| 436   | 1162.5791        | 0.0039 | -0.0158          | 9      |
| 437   | 1162.8142        | 0.0020 | -0.0203          | 10     |
| 438   | 1163.0597        | 0.0021 | -0.0144          | 10     |
| 439   | 1163.2981        | 0.0015 | -0.0155          | 9      |
| 440   | 1163.5443        | 0.0016 | -0.0089          | 9      |
| 441   | 1163.7785        | 0.0018 | -0.0143          | 10     |
| 442   | 1164.0135        | 0.0033 | -0.0188          | 9      |
| 443   | 1164.2632        | 0.0029 | -0.0086          | 9      |
| 444   | 1164.4974        | 0.0022 | -0.0140          | 10     |
| 445   | 1164.7339        | 0.0025 | -0.0171          | 10     |
| 446   | 1164.9798        | 0.0035 | -0.0107          | 9      |
| 447   | 1165.2125        | 0.0036 | -0.0176          | 9      |
| 448   | 1165.4442        | 0.0036 | -0.0254          | 10     |
| 449   | 1165.6781        | 0.0039 | -0.0311          | 9      |
| 450   | 1165.9178        | 0.0093 | -0.0309          | 9      |
| 451   | 1166.1444        | 0.0022 | -0.0439          | 9      |
| 452   | 1166.4033        | 0.0041 | -0.0245          | 10     |
| 453   | 1166.6300        | 0.0040 | -0.0375          | 9      |
| 454   | 1166.8801        | 0.0023 | -0.0269          | 9      |
| 455   | 1167.1160        | 0.0040 | -0.0306          | 10     |
| 456   | 1167.3604        | 0.0028 | -0.0258          | 10     |
| 457   | 1167.6077        | 0.0033 | -0.0179          | 9      |
| 458   | 1167.8491        | 0.0018 | -0.0162          | 8      |
| 459   | 1168.0878        | 0.0039 | -0.0170          | 10     |
| 460   | 1168.3258        | 0.0024 | -0.0186          | 9      |
| 461   | 1168.5572        | 0.0022 | -0.0267          | 9      |
| 462   | 1168.7941        | 0.0037 | -0.0294          | 9      |
| 463   | 1169.0289        | 0.0019 | -0.0342          | 10     |
| 464   | 1169.2693        | 0.0118 | -0.0333          | 5      |
| 468   | 1170.2236        | 0.0081 | -0.0373          | 8      |
| 469   | 1170.4500        | 0.0067 | -0.0504          | 8      |

**Table E5.** Times of negative-superhump maxima in KIC 9406652 during time interval 5 (BJD 2456058–2456200) (continued).

| $E^*$ | Max <sup>†</sup> | Error  | $O - C^{\ddagger}$ | $N^{\S}$ |
|-------|------------------|--------|--------------------|----------|
| 470   | 1170.7002        | 0.0029 | -0.0397            | 10       |
| 471   | 1170.9494        | 0.0034 | -0.0302            | 9        |
| 472   | 1171.1833        | 0.0087 | -0.0358            | 9        |
| 473   | 1171.4204        | 0.0027 | -0.0383            | 10       |
| 474   | 1171.6680        | 0.0043 | -0.0302            | 10       |
| 475   | 1171.8948        | 0.0071 | -0.0430            | 9        |
| 476   | 1172.1428        | 0.0047 | -0.0345            | 9        |
| 477   | 1172.3772        | 0.0036 | -0.0397            | 9        |
| 478   | 1172.6219        | 0.0043 | -0.0346            | 9        |
| 479   | 1172.8448        | 0.0053 | -0.0512            | 9        |
| 480   | 1173.0956        | 0.0050 | -0.0399            | 9        |
| 481   | 1173.3203        | 0.0046 | -0.0548            | 10       |
| 482   | 1173.5663        | 0.0066 | -0.0484            | 9        |
| 483   | 1173.8029        | 0.0085 | -0.0514            | 9        |
| 484   | 1174.0437        | 0.0045 | -0.0501            | 10       |
| 485   | 1174.2828        | 0.0027 | -0.0506            | 10       |
| 486   | 1174.5295        | 0.0035 | -0.0434            | 9        |
| 487   | 1174.7688        | 0.0055 | -0.0436            | 9        |
| 488   | 1175.0113        | 0.0025 | -0.0408            | 10       |
| 489   | 1175.2496        | 0.0050 | -0.0420            | 8        |
| 490   | 1175.4900        | 0.0021 | -0.0412            | 9        |
| 491   | 1175.7410        | 0.0025 | -0.0297            | 9        |
| 492   | 1175.9773        | 0.0030 | -0.0330            | 10       |
| 493   | 1176.2061        | 0.0031 | -0.0437            | 8        |
| 495   | 1176.6782        | 0.0019 | -0.0507            | 10       |
| 496   | 1176.9250        | 0.0033 | -0.0435            | 10       |
| 497   | 1177.1558        | 0.0040 | -0.0522            | 9        |
| 499   | 1177.6325        | 0.0072 | -0.0547            | 10       |
| 500   | 1177.8751        | 0.0034 | -0.0516            | 9        |
| 501   | 1178.1050        | 0.0052 | -0.0613            | 9        |
| 502   | 1178.3530        | 0.0044 | -0.0529            | 10       |
| 503   | 1178.6026        | 0.0054 | -0.0428            | 10       |
| 504   | 1178.8420        | 0.0030 | -0.0430            | 9        |
| 505   | 1179.0620        | 0.0039 | -0.0625            | 8        |
| 506   | 1179.3195        | 0.0061 | -0.0446            | 10       |
| 507   | 1179.5501        | 0.0028 | -0.0535            | 9        |
| 508   | 1179.8018        | 0.0079 | -0.0415            | 9        |
| 509   | 1180.0345        | 0.0065 | -0.0483            | 9        |
| 510   | 1180.2647        | 0.0058 | -0.0577            | 10       |
| 512   | 1180.7534        | 0.0051 | -0.0481            | 9        |
| 515   | 1181.4630        | 0.0082 | -0.0572            | 9        |
| 518   | 1182.1902        | 0.0028 | -0.0487            | 9        |
| 519   | 1182.4201        | 0.0051 | -0.0583            | 9        |
| 524   | 1183.6275        | 0.0107 | -0.0487            | 10       |
| 527   | 1184.3420        | 0.0055 | -0.0529            | 9        |
| 528   | 1184.5836        | 0.0068 | -0.0509            | 10       |
| 538   | 1186.9988        | 0.0058 | -0.0312            | 8        |
| 540   | 1187.4555        | 0.0065 | -0.0537            | 9        |
| 543   | 1188.1954        | 0.0064 | -0.0325            | 10       |
| 548   | 1189.3991        | 0.0088 | -0.0265            | 9        |
| 549   | 1189.6117        | 0.0067 | -0.0535            | 10       |
| 550   | 1189.8493        | 0.0029 | -0.0554            | 10       |

**Table E5.** Times of negative-superhump maxima in KIC 9406652 during time interval 5 (BJD 2456058–2456200) (continued).

| $E^*$ | Max <sup>†</sup> | Error  | $O - C^{\ddagger}$ | $N^{\S}$ |
|-------|------------------|--------|--------------------|----------|
| 552   | 1190.3468        | 0.0113 | -0.0370            | 9        |
| 553   | 1190.6077        | 0.0137 | -0.0157            | 10       |
| 554   | 1190.8316        | 0.0054 | -0.0314            | 9        |
| 557   | 1191.5768        | 0.0090 | -0.0049            | 10       |
| 564   | 1193.2208        | 0.0044 | -0.0378            | 9        |
| 565   | 1193.4537        | 0.0019 | -0.0445            | 9        |
| 566   | 1193.6936        | 0.0040 | -0.0441            | 9        |
| 567   | 1193.9497        | 0.0046 | -0.0275            | 9        |
| 568   | 1194.1761        | 0.0039 | -0.0407            | 10       |
| 569   | 1194.4333        | 0.0041 | -0.0231            | 9        |
| 570   | 1194.6560        | 0.0034 | -0.0400            | 9        |
| 571   | 1194.9049        | 0.0025 | -0.0306            | 10       |
| 572   | 1195.1423        | 0.0024 | -0.0328            | 10       |
| 573   | 1195.3925        | 0.0034 | -0.0222            | 9        |
| 574   | 1195.6371        | 0.0026 | -0.0171            | 9        |
| 575   | 1195.8715        | 0.0028 | -0.0223            | 10       |
| 576   | 1196.1181        | 0.0036 | -0.0152            | 8        |
| 577   | 1196.3603        | 0.0029 | -0.0125            | 9        |
| 578   | 1196.6060        | 0.0032 | -0.0064            | 10       |
| 579   | 1196.8554        | 0.0059 | 0.0034             | 10       |
| 580   | 1197.0972        | 0.0016 | 0.0057             | 9        |
| 581   | 1197.3243        | 0.0039 | -0.0068            | 9        |
| 582   | 1197.5688        | 0.0033 | -0.0019            | 10       |
| 583   | 1197.8236        | 0.0064 | 0.0134             | 9        |
| 584   | 1198.0578        | 0.0044 | 0.0080             | 9        |
| 585   | 1198.2988        | 0.0038 | 0.0094             | 9        |
| 586   | 1198.5473        | 0.0055 | 0.0183             | 10       |
| 587   | 1198.7821        | 0.0030 | 0.0136             | 9        |
| 588   | 1198.9980        | 0.0048 | -0.0100            | 9        |
| 589   | 1199.2636        | 0.0059 | 0.0160             | 9        |
| 590   | 1199.5116        | 0.0068 | 0.0244             | 10       |
| 591   | 1199.7406        | 0.0045 | 0.0138             | 9        |
| 592   | 1199.9734        | 0.0049 | 0.0071             | 6        |

\*Cycle counts.

<sup>†</sup>BJD–2455000.0.

<sup>‡</sup> $C = 2456058.1206 + 0.23956 E$ .

<sup>§</sup>Number of points used for determining the maximum.

**Table E6.** Times of negative-superhump maxima in KIC 9406652 during time interval 6 (BJD 2456200–2456312).

| $E^*$ | Max <sup>†</sup> | Error  | $O - C^{\ddagger}$ | $N^{\S}$ |
|-------|------------------|--------|--------------------|----------|
| 0     | 1200.2252        | 0.0054 | 0.0034             | 10       |
| 1     | 1200.4708        | 0.0047 | 0.0092             | 9        |
| 2     | 1200.7103        | 0.0044 | 0.0089             | 9        |
| 3     | 1200.9612        | 0.0037 | 0.0199             | 10       |
| 4     | 1201.2055        | 0.0026 | 0.0245             | 9        |
| 5     | 1201.4452        | 0.0055 | 0.0244             | 9        |
| 6     | 1201.6770        | 0.0111 | 0.0164             | 9        |
| 7     | 1201.9134        | 0.0075 | 0.0130             | 10       |
| 8     | 1202.1483        | 0.0069 | 0.0081             | 8        |
| 9     | 1202.4058        | 0.0119 | 0.0258             | 9        |
| 10    | 1202.5955        | 0.0091 | -0.0243            | 10       |
| 11    | 1202.8645        | 0.0080 | 0.0049             | 10       |
| 12    | 1203.0933        | 0.0029 | -0.0061            | 9        |
| 13    | 1203.3406        | 0.0028 | 0.0014             | 8        |
| 14    | 1203.5798        | 0.0064 | 0.0008             | 10       |
| 15    | 1203.8273        | 0.0060 | 0.0085             | 10       |
| 17    | 1204.2696        | 0.0044 | -0.0288            | 6        |
| 27    | 1206.6986        | 0.0075 | 0.0022             | 9        |
| 28    | 1206.9371        | 0.0052 | 0.0009             | 9        |
| 29    | 1207.1805        | 0.0039 | 0.0045             | 10       |
| 30    | 1207.4198        | 0.0035 | 0.0040             | 9        |
| 31    | 1207.6613        | 0.0045 | 0.0057             | 9        |
| 32    | 1207.8966        | 0.0106 | 0.0012             | 9        |
| 33    | 1208.1359        | 0.0061 | 0.0007             | 10       |
| 34    | 1208.3774        | 0.0053 | 0.0024             | 10       |
| 35    | 1208.6167        | 0.0049 | 0.0019             | 9        |
| 36    | 1208.8647        | 0.0055 | 0.0101             | 9        |
| 37    | 1209.1103        | 0.0045 | 0.0159             | 10       |
| 38    | 1209.3416        | 0.0039 | 0.0074             | 9        |
| 39    | 1209.5818        | 0.0031 | 0.0078             | 9        |
| 40    | 1209.8337        | 0.0038 | 0.0199             | 9        |
| 41    | 1210.0737        | 0.0093 | 0.0201             | 10       |
| 42    | 1210.3017        | 0.0050 | 0.0083             | 8        |
| 43    | 1210.5320        | 0.0051 | -0.0012            | 9        |
| 44    | 1210.7678        | 0.0068 | -0.0052            | 9        |
| 45    | 1211.0057        | 0.0053 | -0.0071            | 10       |
| 46    | 1211.2471        | 0.0027 | -0.0055            | 9        |
| 47    | 1211.4915        | 0.0032 | -0.0009            | 9        |
| 48    | 1211.7269        | 0.0047 | -0.0053            | 10       |
| 49    | 1211.9809        | 0.0047 | 0.0089             | 10       |
| 50    | 1212.2141        | 0.0052 | 0.0023             | 9        |
| 51    | 1212.4512        | 0.0017 | -0.0004            | 9        |
| 52    | 1212.6990        | 0.0042 | 0.0076             | 10       |
| 53    | 1212.9455        | 0.0041 | 0.0143             | 10       |
| 54    | 1213.1804        | 0.0043 | 0.0094             | 9        |
| 55    | 1213.4269        | 0.0038 | 0.0161             | 9        |
| 56    | 1213.6644        | 0.0041 | 0.0138             | 10       |
| 57    | 1213.9014        | 0.0030 | 0.0110             | 9        |
| 58    | 1214.1395        | 0.0026 | 0.0093             | 9        |
| 59    | 1214.3710        | 0.0030 | 0.0010             | 9        |
| 60    | 1214.5970        | 0.0046 | -0.0128            | 10       |
| 61    | 1214.8405        | 0.0047 | -0.0091            | 9        |

**Table E6.** Times of negative-superhump maxima in KIC 9406652 during time interval 6 (BJD 2456200–2456312) (continued).

| $E^*$ | Max <sup>†</sup> | Error  | $O - C^{\ddagger}$ | $N^{\S}$ |
|-------|------------------|--------|--------------------|----------|
| 62    | 1215.0752        | 0.0063 | -0.0142            | 9        |
| 63    | 1215.3171        | 0.0044 | -0.0121            | 10       |
| 64    | 1215.5620        | 0.0047 | -0.0070            | 10       |
| 65    | 1215.8074        | 0.0032 | -0.0014            | 9        |
| 66    | 1216.0409        | 0.0061 | -0.0077            | 9        |
| 67    | 1216.2856        | 0.0041 | -0.0028            | 9        |
| 68    | 1216.5296        | 0.0053 | 0.0014             | 10       |
| 69    | 1216.7697        | 0.0031 | 0.0017             | 9        |
| 70    | 1217.0104        | 0.0035 | 0.0026             | 9        |
| 71    | 1217.2634        | 0.0059 | 0.0158             | 10       |
| 72    | 1217.5001        | 0.0047 | 0.0127             | 9        |
| 73    | 1217.7395        | 0.0035 | 0.0123             | 9        |
| 74    | 1217.9800        | 0.0047 | 0.0130             | 9        |
| 75    | 1218.2082        | 0.0046 | 0.0014             | 10       |
| 76    | 1218.4489        | 0.0036 | 0.0023             | 9        |
| 77    | 1218.6751        | 0.0070 | -0.0113            | 9        |
| 78    | 1218.9166        | 0.0048 | -0.0096            | 9        |
| 79    | 1219.1499        | 0.0061 | -0.0161            | 10       |
| 80    | 1219.4007        | 0.0056 | -0.0051            | 9        |
| 81    | 1219.6383        | 0.0024 | -0.0073            | 9        |
| 82    | 1219.8828        | 0.0041 | -0.0026            | 10       |
| 83    | 1220.1348        | 0.0060 | 0.0096             | 8        |
| 84    | 1220.3608        | 0.0054 | -0.0042            | 9        |
| 85    | 1220.6003        | 0.0039 | -0.0044            | 9        |
| 86    | 1220.8422        | 0.0049 | -0.0024            | 10       |
| 87    | 1221.0835        | 0.0067 | -0.0009            | 10       |
| 88    | 1221.3334        | 0.0073 | 0.0092             | 9        |
| 89    | 1221.5588        | 0.0051 | -0.0052            | 9        |
| 90    | 1221.8104        | 0.0051 | 0.0066             | 10       |
| 91    | 1222.0359        | 0.0043 | -0.0077            | 9        |
| 92    | 1222.2912        | 0.0027 | 0.0078             | 8        |
| 93    | 1222.5237        | 0.0034 | 0.0005             | 9        |
| 94    | 1222.7536        | 0.0052 | -0.0094            | 10       |
| 95    | 1222.9844        | 0.0043 | -0.0184            | 9        |
| 96    | 1223.2181        | 0.0081 | -0.0245            | 9        |
| 97    | 1223.4667        | 0.0053 | -0.0157            | 9        |
| 98    | 1223.7064        | 0.0030 | -0.0158            | 10       |
| 99    | 1223.9542        | 0.0040 | -0.0078            | 9        |
| 100   | 1224.1955        | 0.0030 | -0.0063            | 9        |
| 101   | 1224.4319        | 0.0061 | -0.0097            | 9        |
| 102   | 1224.6750        | 0.0034 | -0.0064            | 10       |
| 103   | 1224.9204        | 0.0047 | -0.0008            | 9        |
| 104   | 1225.1524        | 0.0065 | -0.0086            | 8        |
| 105   | 1225.4016        | 0.0055 | 0.0008             | 10       |
| 106   | 1225.6521        | 0.0084 | 0.0115             | 10       |
| 107   | 1225.8721        | 0.0043 | -0.0083            | 9        |
| 108   | 1226.1181        | 0.0040 | -0.0021            | 9        |
| 109   | 1226.3529        | 0.0027 | -0.0071            | 9        |
| 110   | 1226.5873        | 0.0110 | -0.0125            | 9        |
| 111   | 1226.8047        | 0.0090 | -0.0349            | 9        |
| 112   | 1227.0477        | 0.0066 | -0.0317            | 9        |
| 113   | 1227.2927        | 0.0052 | -0.0265            | 10       |

**Table E6.** Times of negative-superhump maxima in KIC 9406652 during time interval 6 (BJD 2456200–2456312) (continued).

| $E^*$ | Max <sup>†</sup> | Error  | $O - C^\ddagger$ | $N^\S$ |
|-------|------------------|--------|------------------|--------|
| 114   | 1227.5441        | 0.0049 | -0.0149          | 9      |
| 115   | 1227.7845        | 0.0034 | -0.0143          | 9      |
| 116   | 1228.0165        | 0.0027 | -0.0221          | 10     |
| 117   | 1228.2688        | 0.0053 | -0.0096          | 9      |
| 118   | 1228.4996        | 0.0033 | -0.0186          | 9      |
| 119   | 1228.7420        | 0.0047 | -0.0160          | 9      |
| 120   | 1228.9797        | 0.0053 | -0.0181          | 9      |
| 121   | 1229.2176        | 0.0071 | -0.0200          | 9      |
| 122   | 1229.4616        | 0.0098 | -0.0158          | 9      |
| 123   | 1229.6913        | 0.0063 | -0.0259          | 9      |
| 124   | 1229.9426        | 0.0053 | -0.0144          | 10     |
| 125   | 1230.1754        | 0.0041 | -0.0214          | 9      |
| 126   | 1230.4110        | 0.0031 | -0.0256          | 9      |
| 127   | 1230.6456        | 0.0047 | -0.0308          | 9      |
| 128   | 1230.8831        | 0.0047 | -0.0331          | 10     |
| 129   | 1231.1190        | 0.0092 | -0.0370          | 8      |
| 130   | 1231.3500        | 0.0081 | -0.0458          | 9      |
| 131   | 1231.6008        | 0.0087 | -0.0348          | 9      |
| 132   | 1231.8515        | 0.0045 | -0.0239          | 10     |
| 133   | 1232.0920        | 0.0023 | -0.0232          | 9      |
| 134   | 1232.3277        | 0.0019 | -0.0273          | 9      |
| 135   | 1232.5696        | 0.0037 | -0.0252          | 10     |
| 136   | 1232.8085        | 0.0050 | -0.0261          | 10     |
| 137   | 1233.0470        | 0.0070 | -0.0274          | 9      |
| 138   | 1233.2850        | 0.0065 | -0.0292          | 9      |
| 139   | 1233.5345        | 0.0073 | -0.0195          | 10     |
| 140   | 1233.7751        | 0.0049 | -0.0187          | 10     |
| 141   | 1234.0043        | 0.0046 | -0.0293          | 9      |
| 142   | 1234.2593        | 0.0057 | -0.0141          | 8      |
| 143   | 1234.4963        | 0.0043 | -0.0169          | 10     |
| 144   | 1234.7001        | 0.0079 | -0.0529          | 9      |
| 145   | 1234.9329        | 0.0063 | -0.0599          | 9      |
| 146   | 1235.1853        | 0.0066 | -0.0473          | 9      |
| 147   | 1235.4262        | 0.0063 | -0.0462          | 10     |
| 148   | 1235.6580        | 0.0062 | -0.0542          | 9      |
| 149   | 1235.9075        | 0.0074 | -0.0445          | 9      |
| 150   | 1236.1518        | 0.0046 | -0.0400          | 9      |
| 151   | 1236.4009        | 0.0044 | -0.0307          | 10     |
| 152   | 1236.6375        | 0.0053 | -0.0339          | 9      |
| 153   | 1236.8819        | 0.0067 | -0.0293          | 9      |
| 154   | 1237.1231        | 0.0081 | -0.0279          | 9      |
| 160   | 1238.5766        | 0.0062 | -0.0132          | 9      |
| 161   | 1238.8263        | 0.0169 | -0.0033          | 9      |
| 162   | 1239.0527        | 0.0141 | -0.0167          | 10     |
| 167   | 1240.2148        | 0.0028 | -0.0536          | 9      |
| 169   | 1240.7061        | 0.0026 | -0.0419          | 9      |
| 170   | 1240.9427        | 0.0045 | -0.0451          | 10     |
| 171   | 1241.1982        | 0.0034 | -0.0294          | 9      |
| 172   | 1241.4413        | 0.0031 | -0.0261          | 9      |
| 173   | 1241.6885        | 0.0013 | -0.0187          | 10     |
| 174   | 1241.9513        | 0.0048 | 0.0043           | 10     |
| 175   | 1242.1883        | 0.0044 | 0.0015           | 8      |

**Table E6.** Times of negative-superhump maxima in KIC 9406652 during time interval 6 (BJD 2456200–2456312) (continued).

| $E^*$ | Max <sup>†</sup> | Error  | $O - C^\ddagger$ | $N^\S$ |
|-------|------------------|--------|------------------|--------|
| 176   | 1242.4392        | 0.0035 | 0.0126           | 9      |
| 177   | 1242.6911        | 0.0046 | 0.0247           | 9      |
| 178   | 1242.9511        | 0.0035 | 0.0449           | 9      |
| 185   | 1244.5217        | 0.0056 | -0.0631          | 10     |
| 186   | 1244.7841        | 0.0037 | -0.0405          | 9      |
| 187   | 1245.0253        | 0.0039 | -0.0391          | 9      |
| 188   | 1245.2708        | 0.0060 | -0.0334          | 10     |
| 189   | 1245.5135        | 0.0078 | -0.0305          | 8      |
| 190   | 1245.7598        | 0.0070 | -0.0240          | 6      |
| 215   | 1251.7650        | 0.0089 | -0.0138          | 10     |
| 216   | 1252.0195        | 0.0033 | 0.0009           | 9      |
| 217   | 1252.2542        | 0.0055 | -0.0042          | 8      |
| 218   | 1252.4932        | 0.0077 | -0.0050          | 9      |
| 219   | 1252.7627        | 0.0072 | 0.0247           | 10     |
| 220   | 1253.0096        | 0.0017 | 0.0318           | 9      |
| 221   | 1253.2099        | 0.0087 | -0.0077          | 9      |
| 223   | 1253.7169        | 0.0066 | 0.0197           | 10     |
| 224   | 1253.9600        | 0.0104 | 0.0230           | 9      |
| 225   | 1254.1974        | 0.0069 | 0.0206           | 9      |
| 226   | 1254.4370        | 0.0057 | 0.0204           | 10     |
| 227   | 1254.6807        | 0.0046 | 0.0243           | 10     |
| 228   | 1254.9343        | 0.0038 | 0.0381           | 9      |
| 229   | 1255.1627        | 0.0068 | 0.0267           | 8      |
| 230   | 1255.4256        | 0.0038 | 0.0498           | 10     |
| 231   | 1255.6599        | 0.0057 | 0.0443           | 10     |
| 232   | 1255.9345        | 0.0094 | 0.0791           | 9      |
| 235   | 1256.5428        | 0.0099 | -0.0320          | 9      |
| 236   | 1256.8003        | 0.0090 | -0.0143          | 9      |
| 237   | 1257.0329        | 0.0049 | -0.0215          | 9      |
| 238   | 1257.2811        | 0.0053 | -0.0131          | 10     |
| 239   | 1257.5225        | 0.0070 | -0.0115          | 9      |
| 240   | 1257.7657        | 0.0047 | -0.0081          | 9      |
| 241   | 1258.0192        | 0.0101 | 0.0056           | 10     |
| 242   | 1258.2676        | 0.0101 | 0.0142           | 9      |
| 243   | 1258.5071        | 0.0090 | 0.0139           | 9      |
| 244   | 1258.7423        | 0.0103 | 0.0093           | 9      |
| 245   | 1258.9992        | 0.0047 | 0.0264           | 10     |
| 246   | 1259.2577        | 0.0083 | 0.0451           | 10     |
| 247   | 1259.4836        | 0.0055 | 0.0312           | 9      |
| 248   | 1259.7263        | 0.0054 | 0.0341           | 9      |
| 249   | 1259.9766        | 0.0074 | 0.0446           | 10     |
| 250   | 1260.2108        | 0.0099 | 0.0390           | 10     |
| 251   | 1260.4096        | 0.0091 | -0.0020          | 9      |
| 252   | 1260.6396        | 0.0101 | -0.0118          | 9      |
| 253   | 1260.9272        | 0.0074 | 0.0360           | 10     |
| 254   | 1261.1404        | 0.0024 | 0.0094           | 8      |
| 255   | 1261.3826        | 0.0049 | 0.0118           | 9      |
| 256   | 1261.6311        | 0.0058 | 0.0205           | 9      |
| 257   | 1261.8580        | 0.0128 | 0.0076           | 10     |
| 258   | 1262.1193        | 0.0076 | 0.0291           | 9      |
| 259   | 1262.3571        | 0.0078 | 0.0271           | 9      |
| 260   | 1262.5972        | 0.0103 | 0.0274           | 10     |

**Table E6.** Times of negative-superhump maxima in KIC 9406652 during time interval 6 (BJD 2456200–2456312) (continued).

| $E^*$ | Max <sup>†</sup> | Error  | $O - C^\ddagger$ | $N^\S$ |
|-------|------------------|--------|------------------|--------|
| 261   | 1262.8451        | 0.0068 | 0.0355           | 10     |
| 262   | 1263.0853        | 0.0055 | 0.0359           | 9      |
| 263   | 1263.3273        | 0.0042 | 0.0381           | 9      |
| 264   | 1263.5649        | 0.0043 | 0.0359           | 10     |
| 265   | 1263.8157        | 0.0057 | 0.0469           | 10     |
| 268   | 1264.5439        | 0.0102 | 0.0557           | 10     |
| 270   | 1264.9841        | 0.0121 | 0.0163           | 9      |
| 271   | 1265.1998        | 0.0059 | -0.0078          | 9      |
| 272   | 1265.4500        | 0.0040 | 0.0026           | 10     |
| 273   | 1265.6967        | 0.0050 | 0.0095           | 9      |
| 274   | 1265.9571        | 0.0067 | 0.0301           | 9      |
| 275   | 1266.1912        | 0.0132 | 0.0244           | 9      |
| 276   | 1266.4241        | 0.0074 | 0.0175           | 10     |
| 277   | 1266.6730        | 0.0026 | 0.0266           | 9      |
| 278   | 1266.9106        | 0.0037 | 0.0244           | 9      |
| 279   | 1267.1521        | 0.0042 | 0.0261           | 9      |
| 280   | 1267.3927        | 0.0042 | 0.0268           | 10     |
| 281   | 1267.6288        | 0.0050 | 0.0232           | 9      |
| 282   | 1267.8722        | 0.0045 | 0.0268           | 9      |
| 283   | 1268.1099        | 0.0068 | 0.0247           | 10     |
| 288   | 1269.2886        | 0.0107 | 0.0044           | 6      |
| 289   | 1269.5321        | 0.0031 | 0.0081           | 9      |
| 290   | 1269.7762        | 0.0029 | 0.0124           | 9      |
| 291   | 1270.0138        | 0.0066 | 0.0102           | 10     |
| 292   | 1270.2650        | 0.0068 | 0.0216           | 9      |
| 293   | 1270.5035        | 0.0037 | 0.0203           | 9      |
| 294   | 1270.7549        | 0.0060 | 0.0319           | 9      |
| 295   | 1270.9914        | 0.0049 | 0.0286           | 10     |
| 296   | 1271.2229        | 0.0059 | 0.0203           | 9      |
| 297   | 1271.4719        | 0.0044 | 0.0295           | 9      |
| 298   | 1271.7111        | 0.0030 | 0.0289           | 10     |
| 299   | 1271.9597        | 0.0037 | 0.0377           | 10     |
| 300   | 1272.1982        | 0.0050 | 0.0364           | 9      |
| 301   | 1272.4486        | 0.0103 | 0.0470           | 9      |
| 302   | 1272.6887        | 0.0131 | 0.0473           | 10     |
| 303   | 1272.9114        | 0.0036 | 0.0302           | 10     |
| 304   | 1273.1460        | 0.0125 | 0.0250           | 9      |
| 305   | 1273.3722        | 0.0049 | 0.0114           | 9      |
| 306   | 1273.6113        | 0.0056 | 0.0107           | 10     |
| 307   | 1273.8547        | 0.0040 | 0.0143           | 8      |
| 308   | 1274.0958        | 0.0065 | 0.0156           | 9      |
| 309   | 1274.3402        | 0.0086 | 0.0202           | 9      |
| 310   | 1274.5820        | 0.0088 | 0.0222           | 10     |
| 311   | 1274.8318        | 0.0047 | 0.0322           | 9      |
| 312   | 1275.0746        | 0.0047 | 0.0352           | 9      |
| 313   | 1275.3064        | 0.0070 | 0.0272           | 10     |
| 314   | 1275.5532        | 0.0043 | 0.0342           | 10     |
| 315   | 1275.7865        | 0.0033 | 0.0277           | 9      |
| 316   | 1276.0144        | 0.0035 | 0.0158           | 9      |
| 317   | 1276.2751        | 0.0059 | 0.0367           | 10     |
| 318   | 1276.5033        | 0.0059 | 0.0251           | 10     |
| 319   | 1276.7347        | 0.0094 | 0.0167           | 9      |

**Table E6.** Times of negative-superhump maxima in KIC 9406652 during time interval 6 (BJD 2456200–2456312) (continued).

| $E^*$ | Max <sup>†</sup> | Error  | $O - C^\ddagger$ | $N^\S$ |
|-------|------------------|--------|------------------|--------|
| 320   | 1276.9715        | 0.0035 | 0.0137           | 9      |
| 321   | 1277.1841        | 0.0063 | -0.0135          | 10     |
| 322   | 1277.4394        | 0.0057 | 0.0020           | 10     |
| 323   | 1277.6743        | 0.0031 | -0.0029          | 9      |
| 324   | 1277.9237        | 0.0032 | 0.0067           | 9      |
| 325   | 1278.1623        | 0.0051 | 0.0055           | 10     |
| 326   | 1278.4044        | 0.0063 | 0.0078           | 9      |
| 327   | 1278.6387        | 0.0068 | 0.0023           | 9      |
| 328   | 1278.8811        | 0.0033 | 0.0049           | 9      |
| 329   | 1279.1430        | 0.0047 | 0.0270           | 10     |
| 330   | 1279.3761        | 0.0058 | 0.0203           | 9      |
| 331   | 1279.6141        | 0.0067 | 0.0185           | 9      |
| 332   | 1279.8501        | 0.0068 | 0.0147           | 9      |
| 333   | 1280.0961        | 0.0052 | 0.0209           | 10     |
| 334   | 1280.3335        | 0.0024 | 0.0185           | 9      |
| 335   | 1280.5810        | 0.0064 | 0.0262           | 9      |
| 336   | 1280.7878        | 0.0068 | -0.0068          | 10     |
| 337   | 1281.0237        | 0.0058 | -0.0107          | 10     |
| 338   | 1281.2629        | 0.0088 | -0.0113          | 9      |
| 339   | 1281.4975        | 0.0066 | -0.0165          | 9      |
| 340   | 1281.7482        | 0.0046 | -0.0056          | 10     |
| 341   | 1281.9919        | 0.0050 | -0.0017          | 9      |
| 342   | 1282.2332        | 0.0035 | -0.0002          | 9      |
| 343   | 1282.4761        | 0.0054 | 0.0029           | 9      |
| 344   | 1282.7277        | 0.0085 | 0.0147           | 9      |
| 345   | 1282.9523        | 0.0073 | -0.0005          | 9      |
| 346   | 1283.2007        | 0.0080 | 0.0081           | 9      |
| 347   | 1283.4492        | 0.0068 | 0.0168           | 8      |
| 348   | 1283.6905        | 0.0046 | 0.0183           | 10     |
| 349   | 1283.9244        | 0.0027 | 0.0124           | 9      |
| 350   | 1284.1633        | 0.0032 | 0.0115           | 9      |
| 351   | 1284.4205        | 0.0105 | 0.0289           | 10     |
| 352   | 1284.6455        | 0.0048 | 0.0141           | 10     |
| 353   | 1284.8972        | 0.0079 | 0.0260           | 9      |
| 354   | 1285.0960        | 0.0094 | -0.0150          | 9      |
| 355   | 1285.3571        | 0.0065 | 0.0063           | 10     |
| 356   | 1285.5650        | 0.0115 | -0.0256          | 10     |
| 357   | 1285.8150        | 0.0070 | -0.0154          | 8      |
| 358   | 1286.0523        | 0.0025 | -0.0179          | 9      |
| 359   | 1286.3119        | 0.0051 | 0.0019           | 10     |
| 360   | 1286.5419        | 0.0047 | -0.0079          | 9      |
| 361   | 1286.7898        | 0.0089 | 0.0002           | 9      |
| 362   | 1287.0279        | 0.0059 | -0.0015          | 9      |
| 363   | 1287.2680        | 0.0046 | -0.0012          | 10     |
| 364   | 1287.5087        | 0.0065 | -0.0003          | 9      |
| 365   | 1287.7598        | 0.0054 | 0.0110           | 9      |
| 366   | 1287.9930        | 0.0071 | 0.0044           | 9      |
| 367   | 1288.2418        | 0.0034 | 0.0134           | 10     |
| 368   | 1288.4776        | 0.0061 | 0.0094           | 9      |
| 370   | 1288.9856        | 0.0166 | 0.0378           | 10     |
| 372   | 1289.3784        | 0.0187 | -0.0490          | 9      |
| 374   | 1289.8749        | 0.0050 | -0.0321          | 10     |

**Table E6.** Times of negative-superhump maxima in KIC 9406652 during time interval 6 (BJD 2456200–2456312) (continued).

| $E^*$ | Max <sup>†</sup> | Error  | $O - C^{\ddagger}$ | $N^{\S}$ |
|-------|------------------|--------|--------------------|----------|
| 375   | 1290.1229        | 0.0055 | -0.0239            | 10       |
| 376   | 1290.3727        | 0.0031 | -0.0139            | 9        |
| 377   | 1290.6165        | 0.0017 | -0.0099            | 9        |
| 378   | 1290.8573        | 0.0075 | -0.0089            | 10       |
| 379   | 1291.0862        | 0.0130 | -0.0198            | 9        |
| 380   | 1291.3425        | 0.0070 | -0.0033            | 9        |
| 381   | 1291.5868        | 0.0065 | 0.0012             | 9        |
| 382   | 1291.8480        | 0.0083 | 0.0226             | 9        |
| 383   | 1292.0637        | 0.0078 | -0.0015            | 9        |
| 384   | 1292.3174        | 0.0067 | 0.0124             | 9        |
| 385   | 1292.5529        | 0.0036 | 0.0081             | 10       |
| 386   | 1292.8060        | 0.0123 | 0.0214             | 10       |
| 391   | 1293.9519        | 0.0170 | -0.0317            | 9        |
| 392   | 1294.1898        | 0.0046 | -0.0336            | 9        |
| 393   | 1294.4432        | 0.0049 | -0.0200            | 10       |
| 394   | 1294.6733        | 0.0100 | -0.0297            | 8        |
| 395   | 1294.9367        | 0.0058 | -0.0061            | 9        |
| 396   | 1295.1457        | 0.0131 | -0.0369            | 9        |
| 397   | 1295.4108        | 0.0100 | -0.0116            | 10       |
| 398   | 1295.6615        | 0.0127 | -0.0007            | 9        |
| 399   | 1295.8812        | 0.0086 | -0.0208            | 9        |
| 400   | 1296.1500        | 0.0102 | 0.0082             | 9        |
| 401   | 1296.3925        | 0.0127 | 0.0109             | 10       |
| 402   | 1296.6360        | 0.0061 | 0.0146             | 9        |
| 403   | 1296.8658        | 0.0061 | 0.0046             | 9        |
| 404   | 1297.1309        | 0.0170 | 0.0299             | 10       |
| 409   | 1298.2441        | 0.0128 | -0.0559            | 10       |
| 410   | 1298.5046        | 0.0040 | -0.0352            | 9        |
| 411   | 1298.7533        | 0.0043 | -0.0263            | 9        |
| 412   | 1298.9999        | 0.0075 | -0.0195            | 10       |
| 413   | 1299.2318        | 0.0079 | -0.0274            | 9        |
| 414   | 1299.4665        | 0.0110 | -0.0325            | 9        |
| 415   | 1299.6961        | 0.0130 | -0.0427            | 9        |
| 416   | 1299.9689        | 0.0079 | -0.0097            | 10       |
| 417   | 1300.2323        | 0.0073 | 0.0139             | 9        |
| 418   | 1300.4503        | 0.0124 | -0.0079            | 9        |
| 419   | 1300.6939        | 0.0089 | -0.0041            | 8        |
| 420   | 1300.9542        | 0.0199 | 0.0164             | 10       |
| 425   | 1302.0573        | 0.0100 | -0.0795            | 9        |
| 426   | 1302.3156        | 0.0089 | -0.0610            | 9        |
| 427   | 1302.5699        | 0.0054 | -0.0465            | 10       |
| 428   | 1302.8174        | 0.0064 | -0.0388            | 10       |
| 429   | 1303.0627        | 0.0092 | -0.0333            | 9        |
| 430   | 1303.3074        | 0.0068 | -0.0284            | 9        |

**Table E6.** Times of negative-superhump maxima in KIC 9406652 during time interval 6 (BJD 2456200–2456312) (continued).

| $E^*$ | Max <sup>†</sup> | Error  | $O - C^{\ddagger}$ | $N^{\S}$ |
|-------|------------------|--------|--------------------|----------|
| 431   | 1303.5506        | 0.0143 | -0.0250            | 9        |
| 444   | 1306.6458        | 0.0087 | -0.0472            | 8        |
| 445   | 1306.8956        | 0.0069 | -0.0372            | 9        |
| 446   | 1307.1213        | 0.0095 | -0.0513            | 10       |
| 447   | 1307.3711        | 0.0059 | -0.0413            | 10       |
| 455   | 1309.2427        | 0.0132 | -0.0881            | 9        |
| 459   | 1310.2207        | 0.0173 | -0.0693            | 6        |

\*Cycle counts.

†BJD–2455000.0.

‡  $C = 2456200.2252 + 0.2398 E$ .

§Number of points used for determining the maximum.

**Table E7.** Times of maxima of super-orbital modulations in KIC 9406652 during BJD 2455296–2456312.

| $E^*$ | Max <sup>†</sup> | Error  | $O - C^{\ddagger}$ | $N^{\S}$ |
|-------|------------------|--------|--------------------|----------|
| 0     | 111.2111         | 0.0649 | 0.5510             | 160      |
| 1     | 114.8191         | 0.0744 | 0.0309             | 161      |
| 2     | 118.6719         | 0.0537 | -0.2446            | 160      |
| 3     | 122.8481         | 0.0285 | -0.1966            | 160      |
| 4     | 127.5496         | 0.0477 | 0.3766             | 160      |
| 5     | 131.3386         | 0.0354 | 0.0375             | 161      |
| 6     | 136.7092         | 0.0840 | 1.2799             | 126      |
| 10    | 153.1571         | 0.0512 | 1.2149             | 159      |
| 11    | 156.8011         | 0.0519 | 0.7307             | 160      |
| 12    | 160.3680         | 0.0478 | 0.1693             | 160      |
| 13    | 165.1691         | 0.0665 | 0.8422             | 159      |
| 14    | 168.9000         | 0.0511 | 0.4449             | 161      |
| 15    | 173.2239         | 0.0585 | 0.6406             | 122      |
| 16    | 177.3479         | 0.0325 | 0.6364             | 161      |
| 17    | 181.2534         | 0.0261 | 0.4137             | 158      |
| 18    | 185.2329         | 0.0250 | 0.2650             | 160      |
| 19    | 189.3859         | 0.0212 | 0.2898             | 160      |
| 20    | 193.1056         | 0.0184 | -0.1187            | 161      |
| 21    | 196.5439         | 0.0355 | -0.8087            | 160      |
| 26    | 217.8049         | 0.0914 | -0.1888            | 161      |
| 27    | 221.7506         | 0.0760 | -0.3713            | 158      |
| 28    | 225.6344         | 0.0434 | -0.6156            | 160      |
| 29    | 230.3823         | 0.0558 | 0.0040             | 113      |
| 32    | 242.0010         | 0.0521 | -0.7619            | 160      |
| 33    | 246.4117         | 0.0356 | -0.4795            | 161      |
| 34    | 250.3745         | 0.0544 | -0.6449            | 159      |
| 36    | 258.6454         | 0.0594 | -0.6304            | 161      |
| 38    | 266.8897         | 0.0374 | -0.6425            | 161      |
| 39    | 270.6515         | 0.0826 | -1.0089            | 161      |
| 40    | 274.3019         | 0.0498 | -1.4868            | 161      |
| 41    | 279.0799         | 0.0550 | -0.8370            | 160      |
| 42    | 283.1797         | 0.0601 | -0.8654            | 161      |
| 43    | 287.2059         | 0.1183 | -0.9674            | 160      |
| 48    | 308.7004         | 0.0383 | -0.1140            | 160      |
| 50    | 317.0621         | 0.0421 | -0.0087            | 161      |
| 53    | 329.0555         | 0.0209 | -0.4000            | 161      |
| 54    | 332.3752         | 0.0756 | -1.2084            | 161      |
| 55    | 336.9099         | 0.0335 | -0.8020            | 160      |
| 56    | 341.6020         | 0.0390 | -0.2381            | 159      |
| 57    | 345.8326         | 0.0758 | -0.1357            | 156      |
| 63    | 370.7341         | 0.0570 | -0.0035            | 161      |
| 64    | 374.8410         | 0.0865 | -0.0248            | 160      |
| 67    | 388.3625         | 0.0330 | 1.1120             | 160      |
| 68    | 392.0250         | 0.0494 | 0.6463             | 159      |
| 70    | 400.5309         | 0.0464 | 0.8958             | 161      |
| 72    | 408.8604         | 0.0272 | 0.9688             | 160      |
| 73    | 412.7953         | 0.0185 | 0.7755             | 159      |
| 74    | 417.0991         | 0.0265 | 0.9512             | 160      |
| 75    | 420.9504         | 0.0555 | 0.6742             | 158      |
| 76    | 424.8580         | 0.0677 | 0.4536             | 157      |
| 77    | 429.6580         | 0.1227 | 1.1253             | 161      |
| 80    | 443.4263         | 0.0529 | 2.5090             | 160      |

**Table E7.** Times of maxima of super-orbital modulations in KIC 9406652 during BJD 2455296–2456312 (continued).

| $E^*$ | Max <sup>†</sup> | Error  | $O - C^{\ddagger}$ | $N^{\S}$ |
|-------|------------------|--------|--------------------|----------|
| 81    | 447.5069         | 0.0323 | 2.4615             | 160      |
| 82    | 450.9693         | 0.0294 | 1.7956             | 157      |
| 83    | 455.0399         | 0.0317 | 1.7380             | 160      |
| 84    | 458.7953         | 0.0331 | 1.3652             | 160      |
| 85    | 463.0295         | 0.0288 | 1.4712             | 158      |
| 86    | 466.8901         | 0.0714 | 1.2036             | 161      |
| 91    | 487.9718         | 0.0595 | 1.6442             | 161      |
| 93    | 496.1696         | 0.0605 | 1.5856             | 161      |
| 101   | 526.0904         | 0.1044 | -1.5194            | 160      |
| 102   | 530.9681         | 0.0460 | -0.7699            | 161      |
| 103   | 534.7121         | 0.0175 | -1.1541            | 160      |
| 104   | 539.0250         | 0.1012 | -0.9694            | 116      |
| 105   | 543.4223         | 0.1705 | -0.7003            | 159      |
| 108   | 556.5749         | 0.1544 | 0.0676             | 160      |
| 109   | 558.2739         | 0.4324 | -2.3616            | 161      |
| 111   | 568.6020         | 0.0960 | -0.2900            | 129      |
| 112   | 572.8341         | 0.0523 | -0.1860            | 160      |
| 114   | 580.4566         | 0.0178 | -0.8200            | 161      |
| 115   | 584.3340         | 0.0587 | -1.0708            | 161      |
| 120   | 605.7358         | 0.0317 | -0.3101            | 159      |
| 121   | 609.7151         | 0.0357 | -0.4590            | 160      |
| 122   | 613.4503         | 0.0328 | -0.8520            | 161      |
| 123   | 617.7719         | 0.0411 | -0.6586            | 160      |
| 124   | 621.1387         | 0.0655 | -1.4201            | 161      |
| 126   | 629.8687         | 0.2195 | -0.9464            | 160      |
| 128   | 638.5355         | 0.0972 | -0.5361            | 158      |
| 129   | 643.3265         | 0.0814 | 0.1267             | 157      |
| 130   | 646.8133         | 0.0368 | -0.5148            | 158      |
| 131   | 650.9864         | 0.0422 | -0.4698            | 159      |
| 132   | 655.7686         | 0.0476 | 0.1841             | 158      |
| 133   | 658.7354         | 0.0618 | -0.9773            | 158      |
| 134   | 663.3220         | 0.0687 | -0.5189            | 157      |
| 137   | 674.6903         | 0.1743 | -1.5352            | 159      |
| 138   | 679.7192         | 0.0535 | -0.6346            | 161      |
| 139   | 684.6476         | 0.0234 | 0.1657             | 160      |
| 145   | 710.4795         | 0.0204 | 1.2283             | 161      |
| 147   | 717.5499         | 0.0183 | 0.0422             | 159      |
| 148   | 722.2685         | 0.0180 | 0.6327             | 158      |
| 149   | 725.6601         | 0.0257 | -0.1040            | 158      |
| 150   | 729.1576         | 0.0552 | -0.7347            | 152      |
| 157   | 758.6000         | 0.0384 | -0.1899            | 124      |
| 158   | 762.8501         | 0.0566 | -0.0679            | 159      |
| 162   | 779.6379         | 0.0363 | 0.2070             | 160      |
| 163   | 782.2866         | 0.0861 | -1.2725            | 161      |
| 164   | 788.2415         | 0.0794 | 0.5542             | 117      |
| 171   | 815.5111         | 0.0943 | -1.0737            | 125      |
| 172   | 820.9808         | 0.0321 | 0.2678             | 159      |
| 173   | 824.8609         | 0.0435 | 0.0197             | 160      |
| 174   | 829.4060         | 0.0264 | 0.4365             | 157      |
| 175   | 833.3556         | 0.0249 | 0.2579             | 156      |
| 176   | 837.3334         | 0.0313 | 0.1075             | 159      |
| 181   | 858.3365         | 0.0426 | 0.4695             | 158      |

**Table E7.** Times of maxima of super-orbital modulations in KIC 9406652 during BJD 2455296–2456312 (continued).

| $E^*$ | Max <sup>†</sup> | Error  | $O - C^{\ddagger}$ | $N^{\S}$ |
|-------|------------------|--------|--------------------|----------|
| 182   | 862.6130         | 0.0152 | 0.6178             | 156      |
| 183   | 866.6476         | 0.0204 | 0.5242             | 158      |
| 184   | 870.6212         | 0.0167 | 0.3695             | 161      |
| 185   | 875.1957         | 0.0218 | 0.8159             | 158      |
| 186   | 879.2613         | 0.0314 | 0.7532             | 114      |
| 187   | 882.8930         | 0.0270 | 0.2568             | 161      |
| 188   | 886.9308         | 0.0279 | 0.1663             | 159      |
| 189   | 891.1798         | 0.0326 | 0.2871             | 158      |
| 190   | 894.8272         | 0.0304 | -0.1937            | 161      |
| 191   | 898.9136         | 0.0530 | -0.2356            | 159      |
| 192   | 903.4744         | 0.1187 | 0.1971             | 139      |
| 196   | 920.7449         | 0.0275 | 0.9547             | 161      |
| 199   | 933.2093         | 0.0423 | 1.0344             | 161      |
| 200   | 936.7988         | 0.0520 | 0.4957             | 139      |
| 201   | 941.4188         | 0.0418 | 0.9876             | 161      |
| 202   | 944.7597         | 0.0305 | 0.2002             | 160      |
| 203   | 949.0009         | 0.0206 | 0.3132             | 161      |
| 204   | 952.7005         | 0.0291 | -0.1154            | 161      |
| 206   | 960.6502         | 0.0116 | -0.4222            | 161      |
| 207   | 964.5549         | 0.0186 | -0.6456            | 160      |
| 208   | 968.3082         | 0.0274 | -1.0206            | 127      |
| 209   | 972.2822         | 0.0237 | -1.1748            | 160      |
| 210   | 976.1168         | 0.0631 | -1.4684            | 160      |
| 211   | 980.3630         | 0.0583 | -1.3504            | 159      |
| 214   | 992.5808         | 0.1667 | -1.5172            | 161      |
| 215   | 996.4274         | 0.0979 | -1.7989            | 161      |
| 218   | 1009.2902        | 0.1101 | -1.3208            | 160      |
| 219   | 1014.2534        | 0.0191 | -0.4858            | 160      |
| 220   | 1017.5596        | 0.0388 | -1.3077            | 161      |
| 221   | 1022.4393        | 0.0245 | -0.5563            | 161      |
| 222   | 1026.1133        | 0.0515 | -1.0105            | 160      |
| 223   | 1030.3415        | 0.0456 | -0.9105            | 157      |
| 224   | 1034.5395        | 0.0737 | -0.8407            | 161      |
| 234   | 1076.1810        | 0.0482 | -0.4814            | 158      |
| 235   | 1080.5010        | 0.0980 | -0.2896            | 160      |
| 236   | 1084.3010        | 0.0413 | -0.6178            | 159      |
| 237   | 1089.0255        | 0.0204 | -0.0216            | 161      |
| 238   | 1093.1552        | 0.0242 | -0.0200            | 160      |
| 240   | 1101.4316        | 0.0787 | -0.0001            | 161      |

\* Cycle counts.

<sup>†</sup> BJD–2455000.0.

<sup>‡</sup>  $C = 2455111.2111 + 4.128215 E$ .

<sup>§</sup> Number of points used for determining the maximum.

**Table E8.** Results of the regression for the model of form,  $a \cos(2\pi(\varphi - b)) + 1$  during BJD 2455318–2456312 in subsection 3.4.2 in the main texts. The  $p$  value is less than  $2.0 \times 10^{-16}$ .

| Start     | End       | $a$    | Error of $a^*$ | $b$     | Error of $b^*$ |
|-----------|-----------|--------|----------------|---------|----------------|
| 296.7610  | 346.7610  | 0.0210 | 0.0011         | 0.6678  | 0.0081         |
| 346.7610  | 396.7610  | 0.0535 | 0.0010         | 0.0620  | 0.0030         |
| 396.7610  | 446.7610  | 0.0248 | 0.0011         | 0.3773  | 0.0073         |
| 446.7610  | 496.7610  | 0.0207 | 0.0009         | 0.3952  | 0.0066         |
| 496.7610  | 552.4667  | 0.0417 | 0.0012         | 0.1258  | 0.0047         |
| 568.5679  | 608.5679  | 0.0256 | 0.0011         | 0.5406  | 0.0067         |
| 608.5679  | 642.9667  | 0.0320 | 0.0018         | 0.3494  | 0.0089         |
| 643.2119  | 688.2119  | 0.0155 | 0.0007         | 0.2776  | 0.0077         |
| 688.2119  | 733.2119  | 0.0062 | 0.0005         | 0.1809  | 0.0121         |
| 733.2119  | 778.2119  | 0.0242 | 0.0011         | 0.6461  | 0.0070         |
| 778.2119  | 823.2119  | 0.0299 | 0.0014         | 0.6034  | 0.0077         |
| 823.2119  | 852.9864  | 0.0226 | 0.0009         | 0.1600  | 0.0064         |
| 875.0130  | 920.0130  | 0.0228 | 0.0018         | 0.0898  | 0.0122         |
| 920.0130  | 965.0130  | 0.0097 | 0.0007         | -0.1629 | 0.0122         |
| 965.0130  | 1010.0130 | 0.0062 | 0.0008         | 0.5853  | 0.0208         |
| 1010.0130 | 1057.8930 | 0.0236 | 0.0005         | 0.4130  | 0.0032         |
| 1058.1380 | 1108.1380 | 0.0518 | 0.0006         | 0.5606  | 0.0019         |
| 1108.1380 | 1158.1380 | 0.0450 | 0.0014         | 0.1785  | 0.0049         |
| 1158.1380 | 1184.9920 | 0.0387 | 0.0009         | 0.4744  | 0.0038         |
| 1200.2360 | 1260.2360 | 0.0208 | 0.0008         | 0.4180  | 0.0060         |
| 1260.2360 | 1310.2050 | 0.0141 | 0.0005         | 0.3982  | 0.0060         |

\*The standard errors.
